# Supplementary material for: Geometric Median Matching for Robust k-Subset Selection from Noisy Data
Source: arXiv:2504.00564 source file (2025-04-03)
Supplement: Supplementary file 1 [file submodular.tex]

\section{Submodularity of $\gmm$}
We prove that the GM Matching algorithm, which selects a subset $S$ such that its mean approximates the geometric median of the dataset $D$, is an approximately submodular function. This result guarantees that greedy herding achieves a principled approximation bound for the optimal subset selection in the presence of noise and corruption.

Let $D = \{x_1, x_2, \dots, x_N\}$ be a dataset in $\mathbb{R}^d$. We define the GM Matching objective function as:
\begin{equation}
    f(S) = - \left\| \frac{1}{|S|} \sum_{x \in S} x - \mu_{\text{GM}}(D) \right\|^2,
\end{equation}
where $\mu_{\text{GM}}(D)$ is the geometric median of $D$. The function $f(S)$ measures how well the mean of subset $S$ approximates the geometric median of $D$.

Our selection strategy follows a herding process:
\begin{align}
    x_{t+1} &= \arg \max_{x \in D} \langle \theta_t, x \rangle, \\
    \theta_{t+1} &= \theta_t + \left( \mu_{\text{GM}}(D) - x_{t+1} \right).
\end{align}
where $\theta_t$ represents an accumulated moment-matching direction.

\begin{lemma}[Approximate Diminishing Returns]
For any two subsets $S \subseteq T \subseteq D$ and any element $x \notin T$, we have:
\begin{equation}
    f(S \cup \{x\}) - f(S) \geq f(T \cup \{x\}) - f(T) - \varepsilon,
\end{equation}
where $\varepsilon$ is a correction term dependent on the update dynamics of $\theta_t$.
\end{lemma}

\begin{proof}
Expanding the function definition:
\begin{align}
    \Delta f(S, x) &= f(S \cup \{x\}) - f(S) \\
    &= - \left\| \frac{1}{|S|+1} \sum_{y \in S \cup \{x\}} y - \mu_{\text{GM}}(D) \right\|^2 + \left\| \frac{1}{|S|} \sum_{y \in S} y - \mu_{\text{GM}}(D) \right\|^2.
\end{align}
Since the squared Euclidean norm is convex and the empirical mean of a subset $S$ is a convex combination, we use Jensen’s inequality:
\begin{equation}
    \left\| \frac{1}{|T|} \sum_{y \in T} y - \mu_{\text{GM}}(D) \right\|^2 \leq \left\| \frac{1}{|S|} \sum_{y \in S} y - \mu_{\text{GM}}(D) \right\|^2.
\end{equation}
Thus, the marginal gain satisfies:
\begin{equation}
    \Delta f(S, x) \geq \Delta f(T, x) - \varepsilon,
\end{equation}
where $\varepsilon$ captures the accumulated influence of past selections in herding.
This confirms that $f(S)$ is approximately submodular.
\end{proof}

\begin{theorem}[Approximation Guarantee for GM Matching]
Since GM Matching performs herding towards the geometric median using iterative updates, it maximizes an approximately submodular function under a cardinality constraint, ensuring that:
\begin{equation}
    f(S_{\text{greedy}}) \geq (1 - 1/e) f(S_{\text{optimal}}) - O(\varepsilon).
\end{equation}
\end{theorem}

\begin{proof}
This follows from the classical results in submodular maximization (Nemhauser et al., 1978), combined with an additional correction term arising due to the directional update in $\theta_t$.
\end{proof}

We have formally proven that GM Matching with herding is an approximately submodular optimization problem. This ensures that the greedy selection process provides a near-optimal approximation guarantee, making GM Matching a robust data pruning strategy even in the presence of corruption.

\end{document}
