# Supplementary material for: Geometric Median Matching for Robust k-Subset Selection from Noisy Data
Source: arXiv:2504.00564 source file (2025-04-03)
Supplement: Supplementary file 2 [file add_exp.tex]

\clearpage
\section{Synthetic Experiments}
\label{sec:app-syn}
We simulate a Gaussian Mixture Model (GMM) with clean and adversarial components to evaluate robust moment estimation in noisy datasets. The clean samples are drawn from a Anisotropic Gaussian distribution with mean $[0, 0]$ and covariance $\begin{bmatrix} 1 & 0.5 \\ 0.5 & 1 \end{bmatrix}$, while the adversarial samples are drawn from a Gaussian with mean $[-5, 5]$ and the same covariance. We generate 1000 samples, forming a corrupted dataset by combining the clean and adversarial data. 

\begin{itemize}
    \item In~\cref{fig:toy-mean-estimation}, we compare the mean of the corrupted dataset (noisy moment) with a robustly estimated mean using the geometric median to mitigate adversarial influence. 
    
    \item Additionally, in~\cref{fig:toy-corr=0}-\ref{fig:toy-corr=45}, we compare different geometric pruning strategies in the toy setting. 
\end{itemize}

\input{plots/toy/fig.toy_mean-estimation}
\begin{figure*}[t] 
\centering
\subfloat[Random]
{\includegraphics[width=0.3\textwidth]{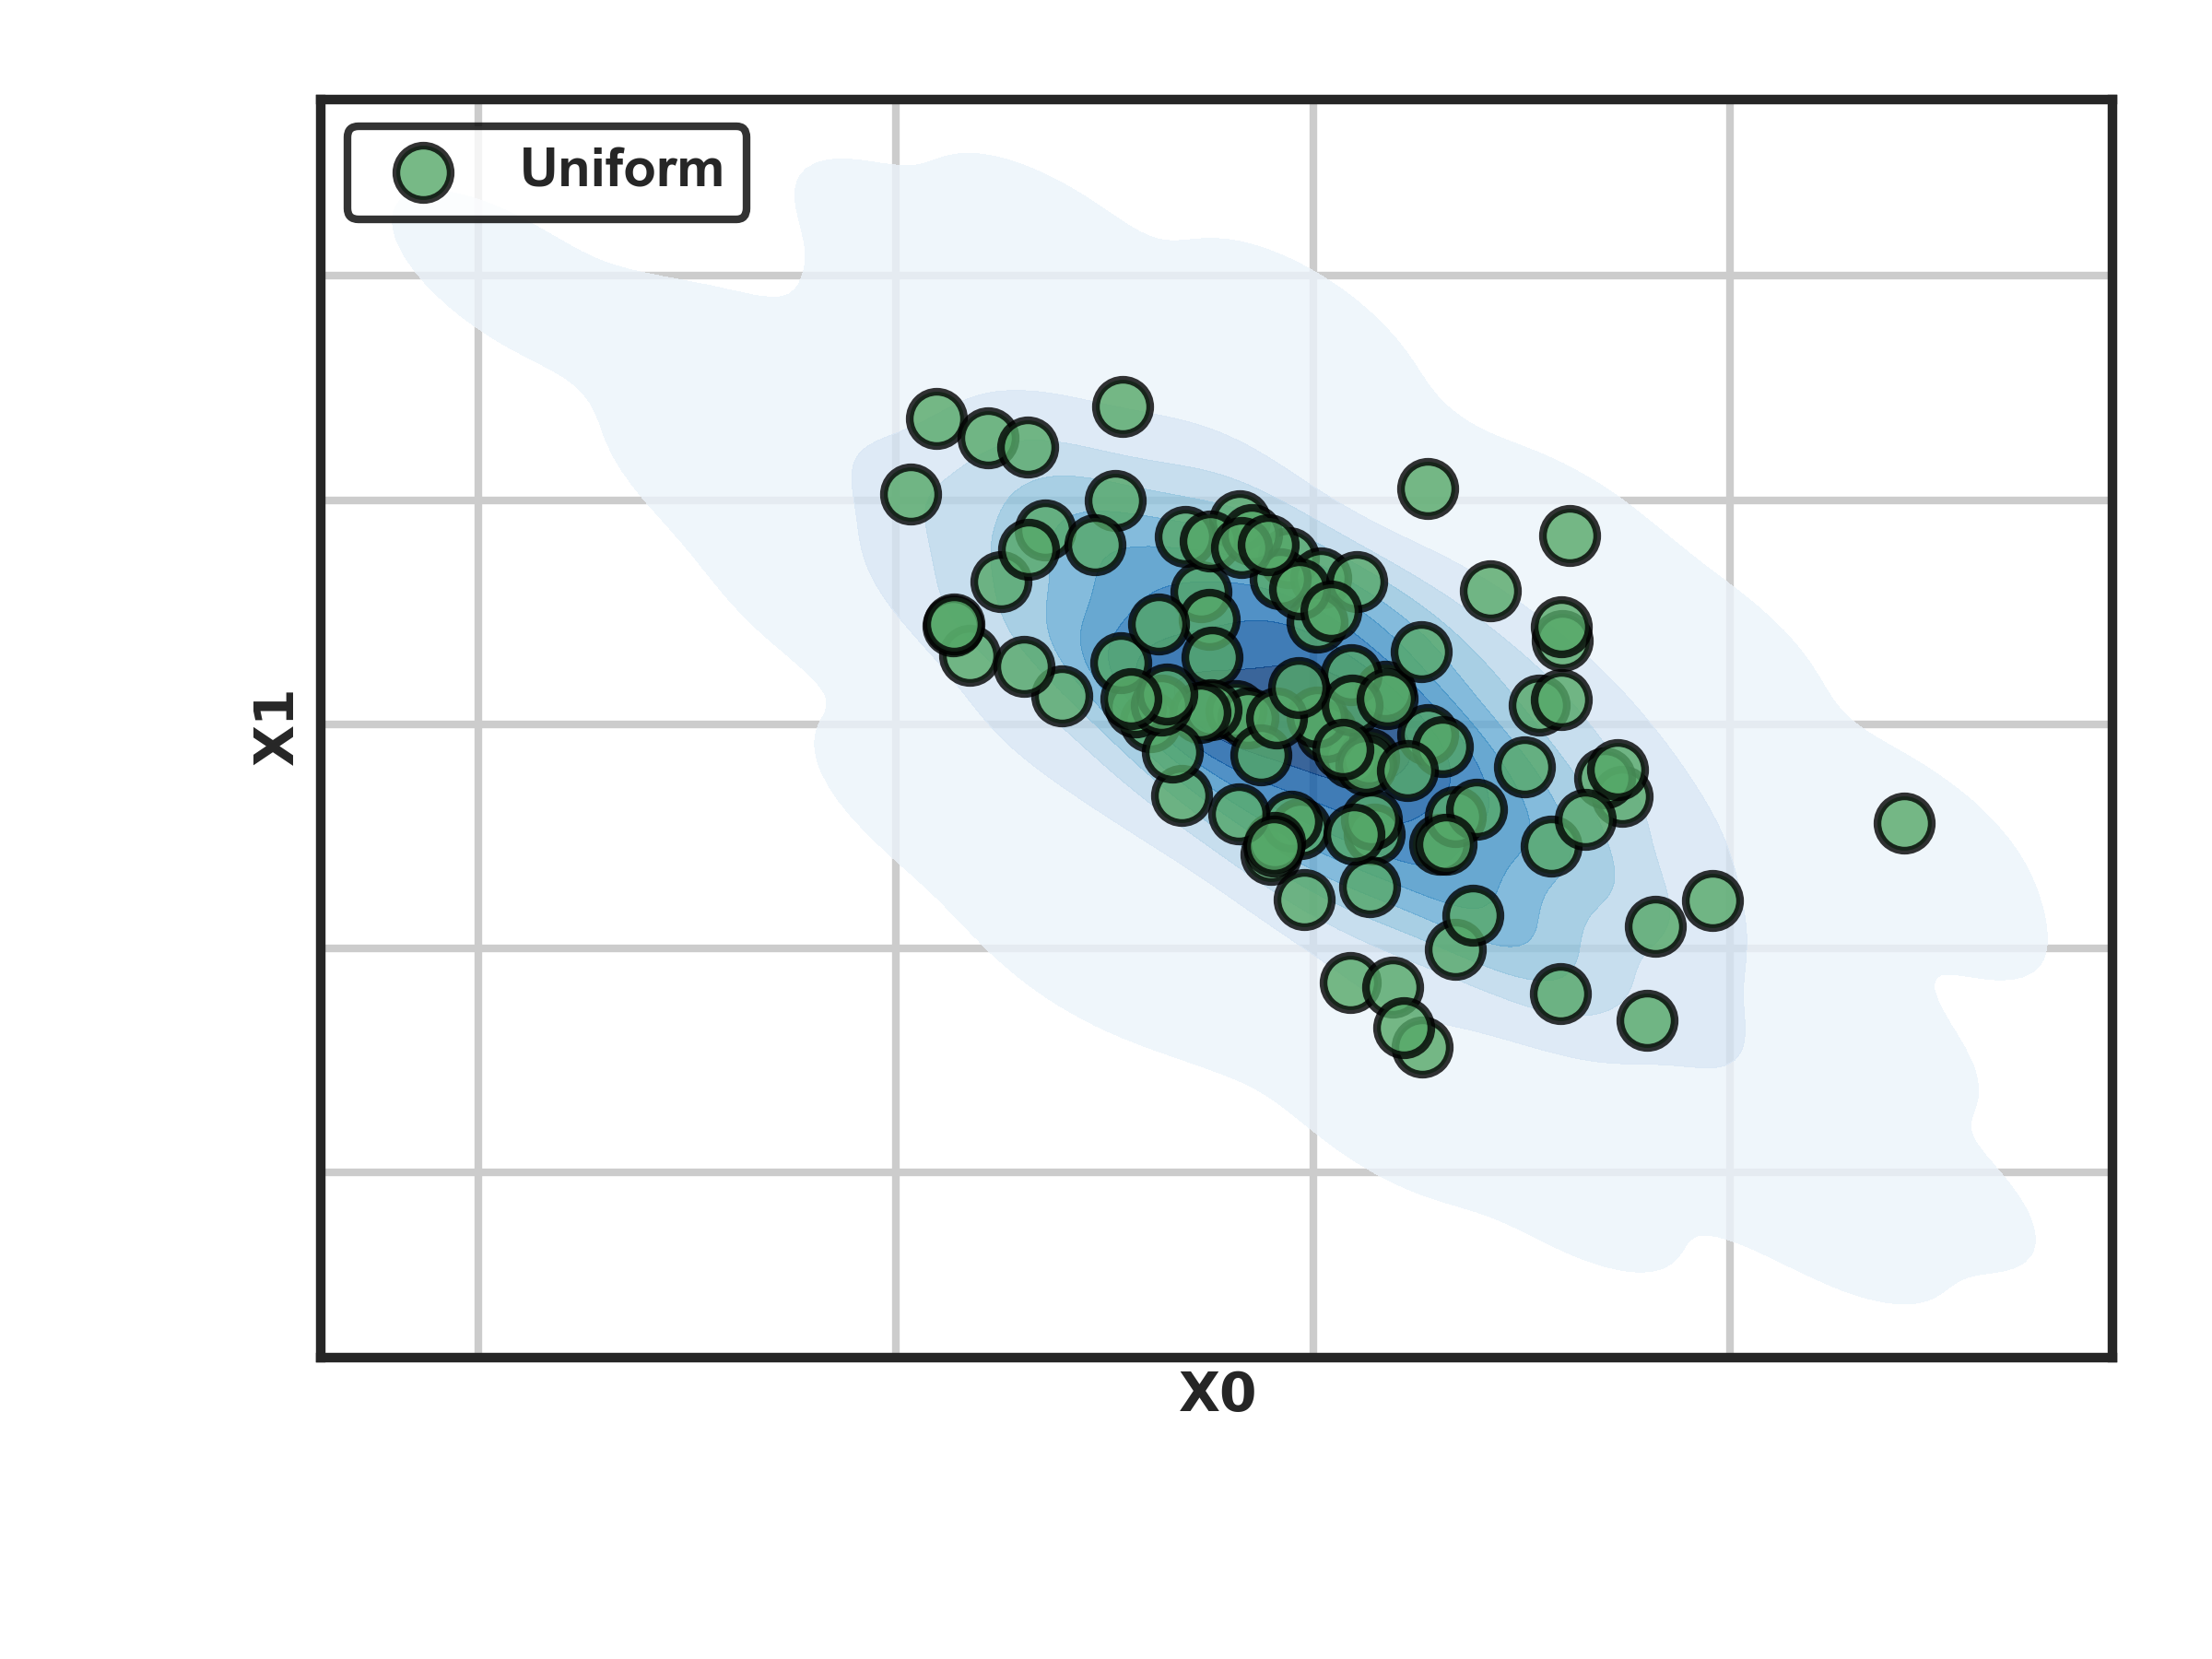}}
\subfloat[Easy]
{\includegraphics[width=0.3\textwidth]{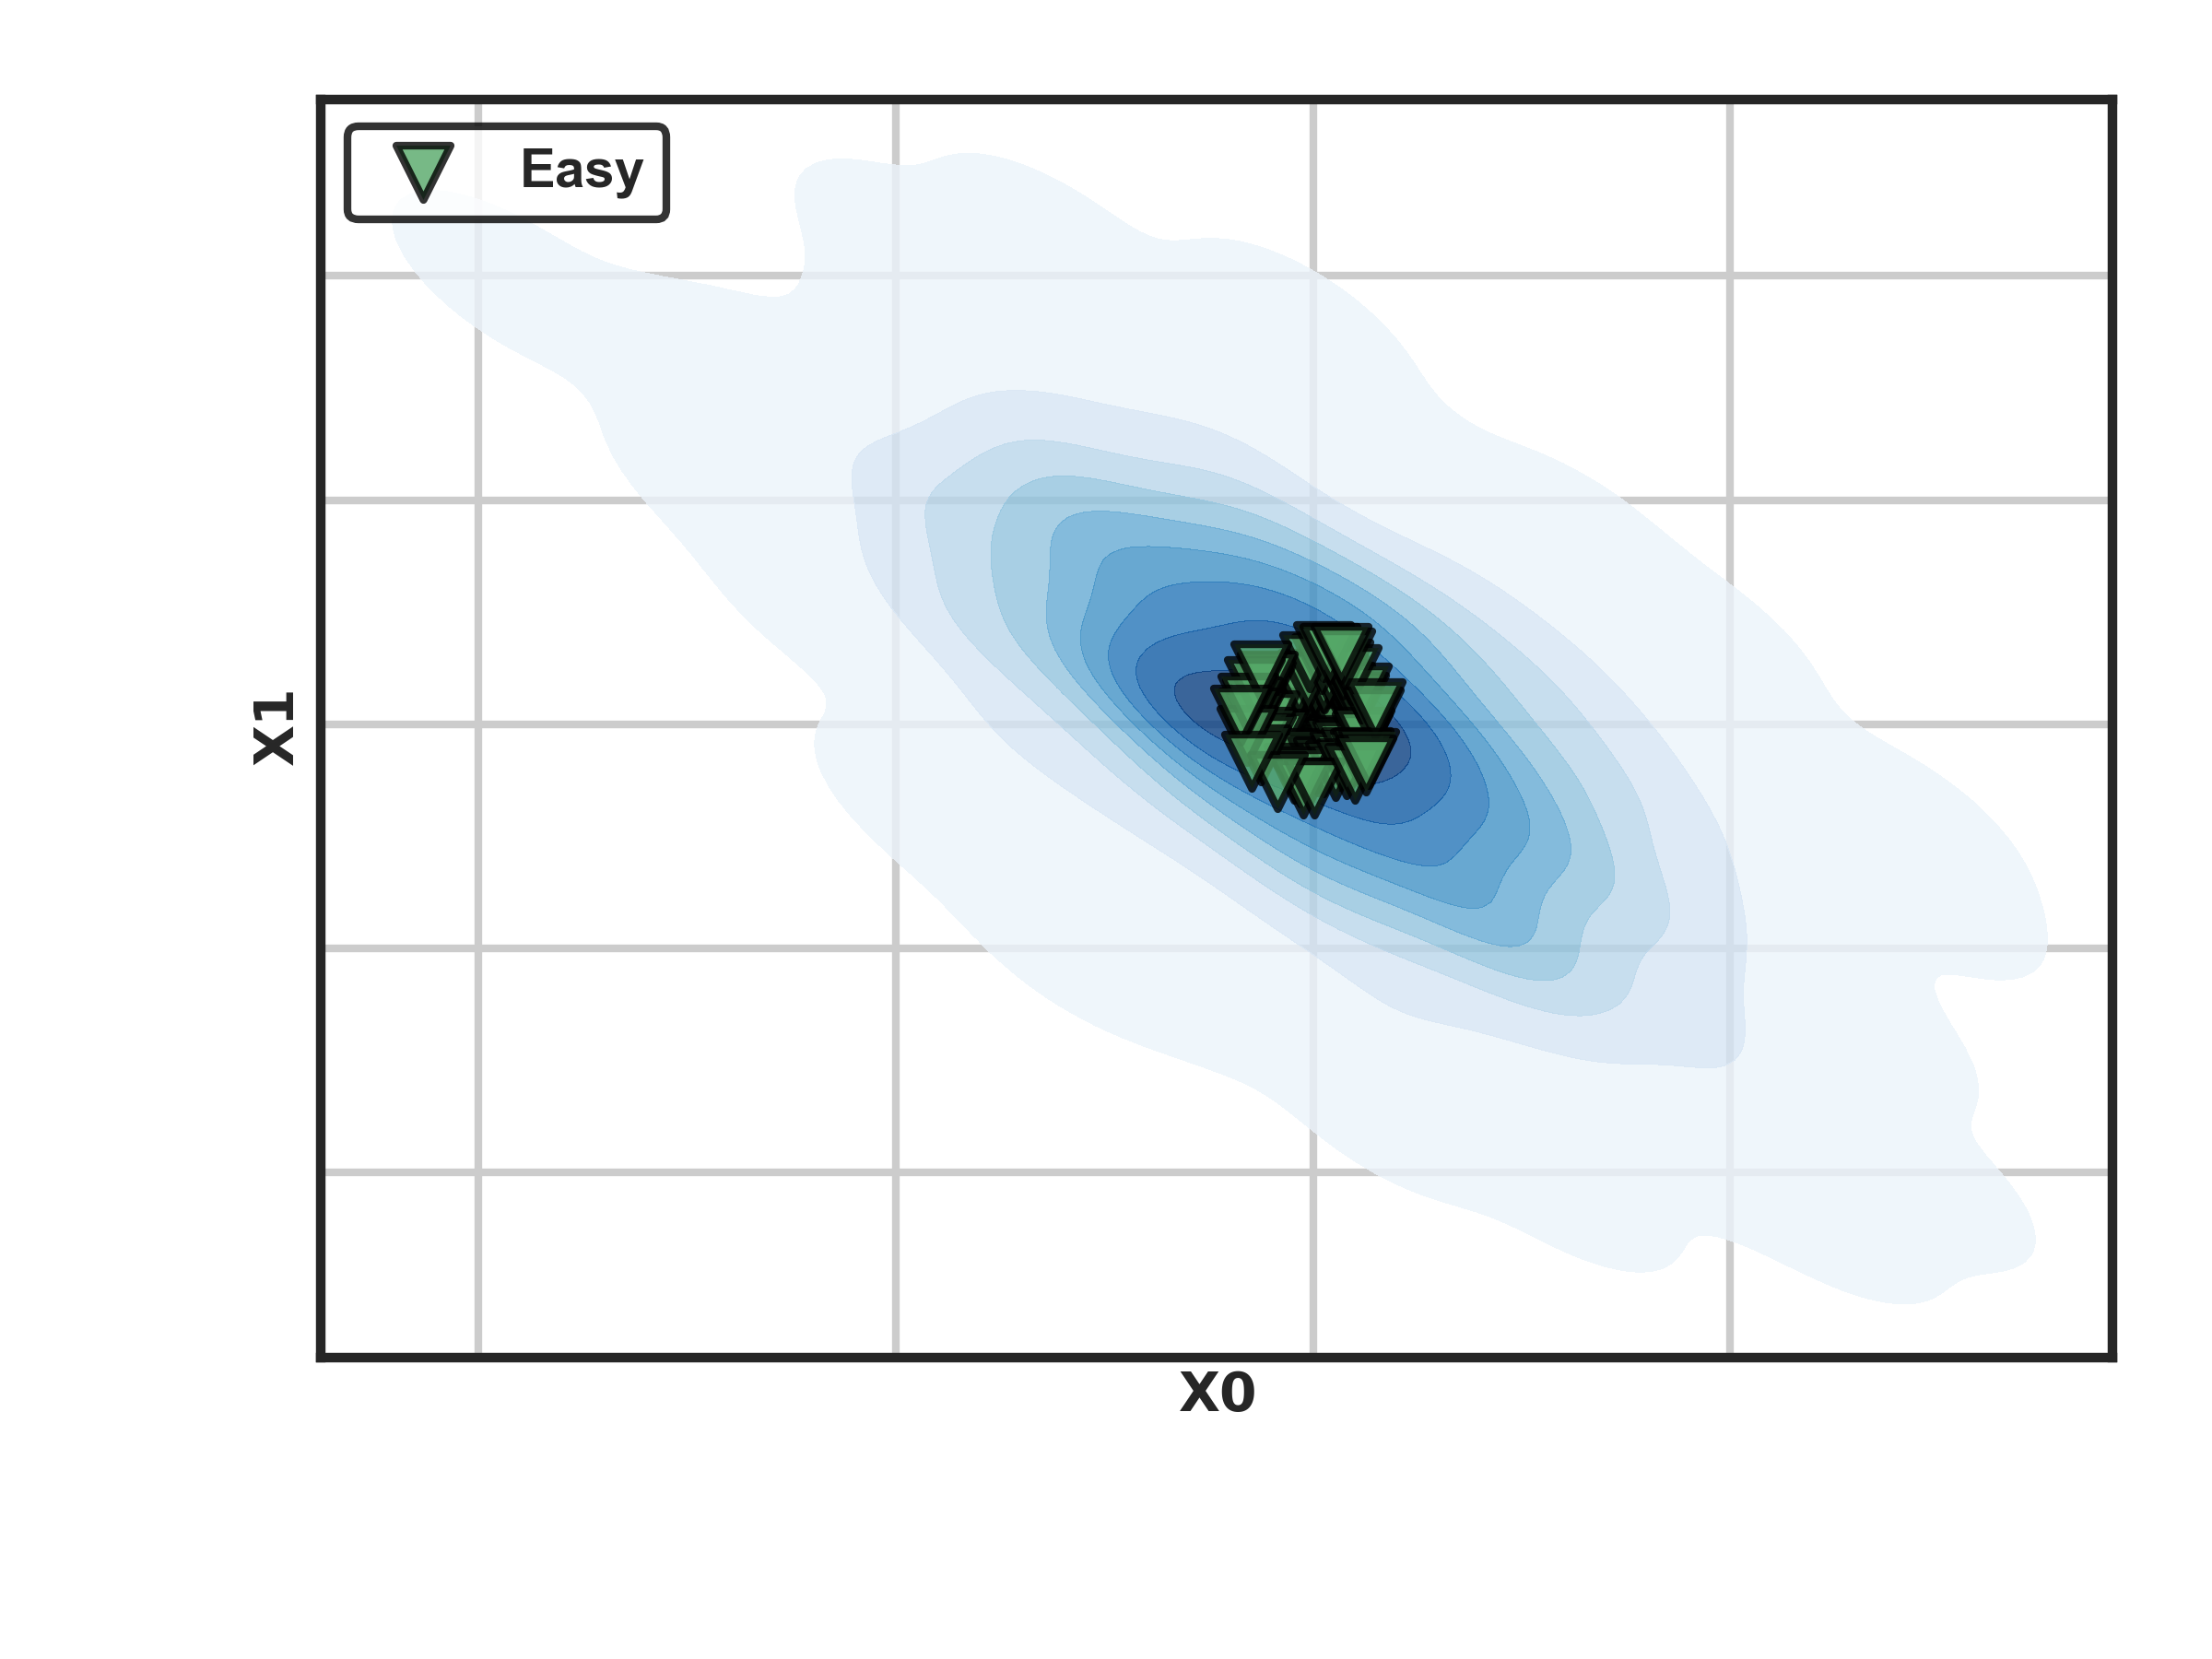}}
\subfloat[Hard]
{\includegraphics[width=0.3\textwidth]{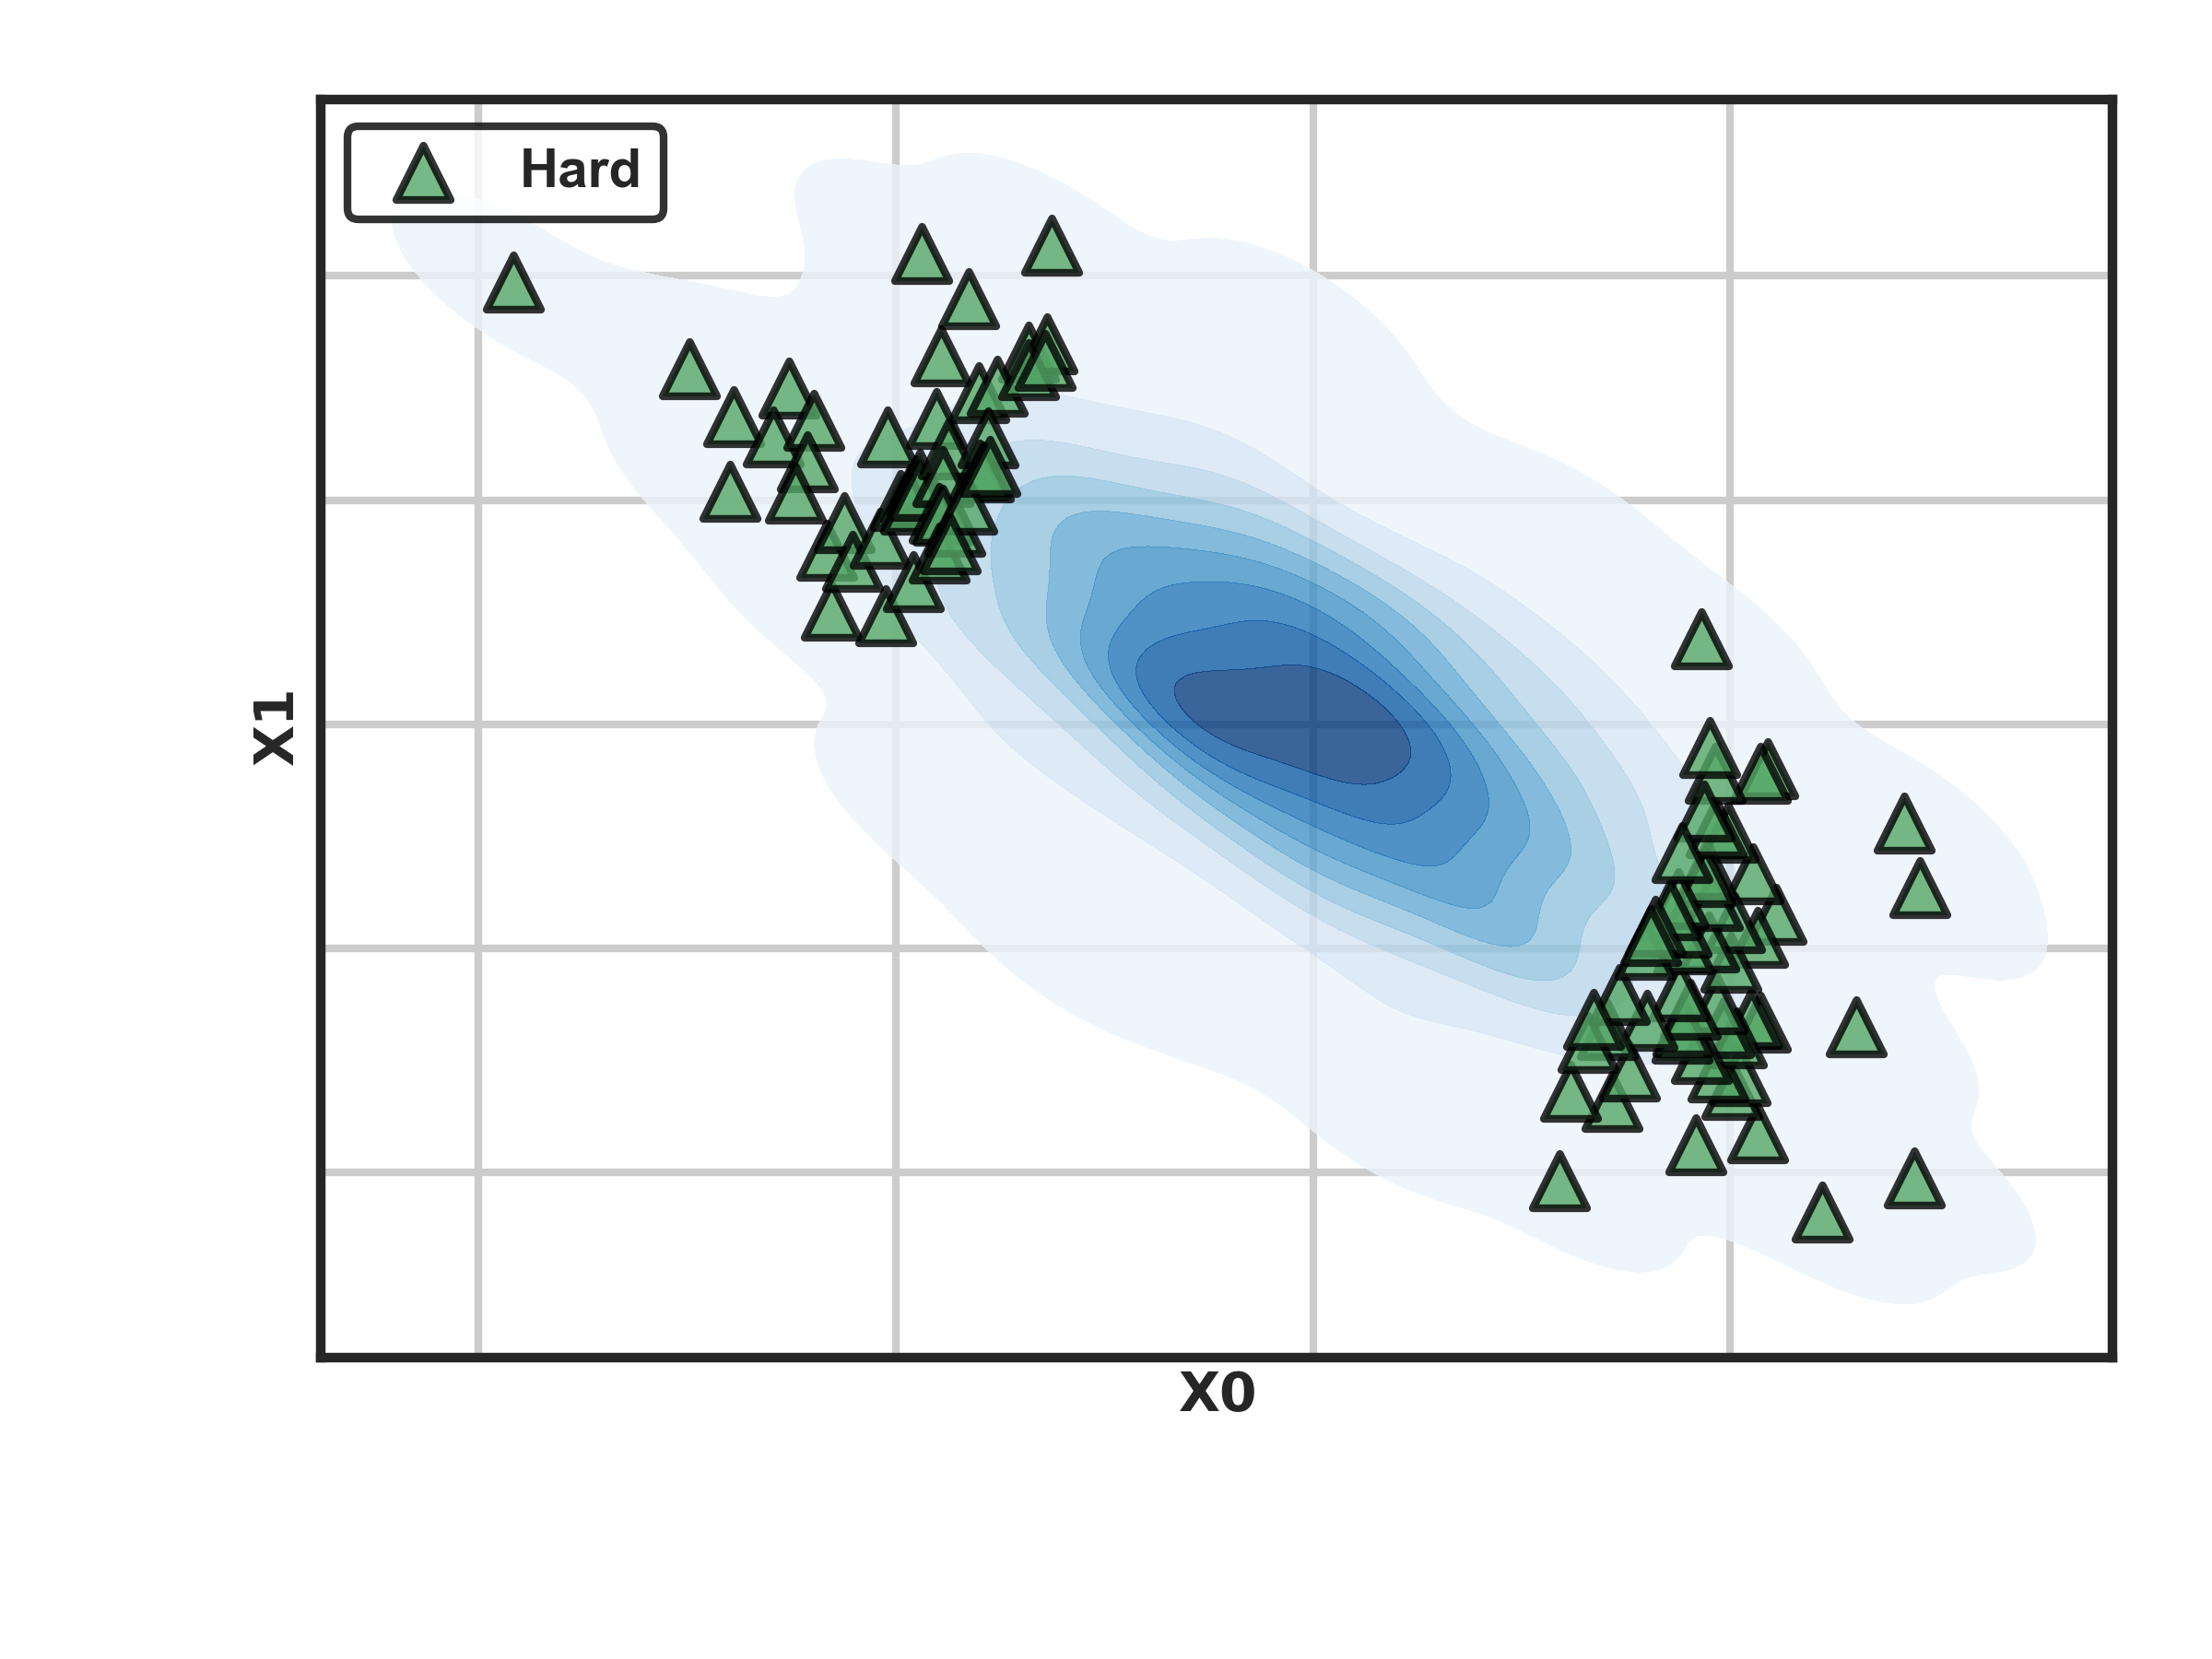}}
\\
\subfloat[Moderate]
{\includegraphics[width=0.3\textwidth]{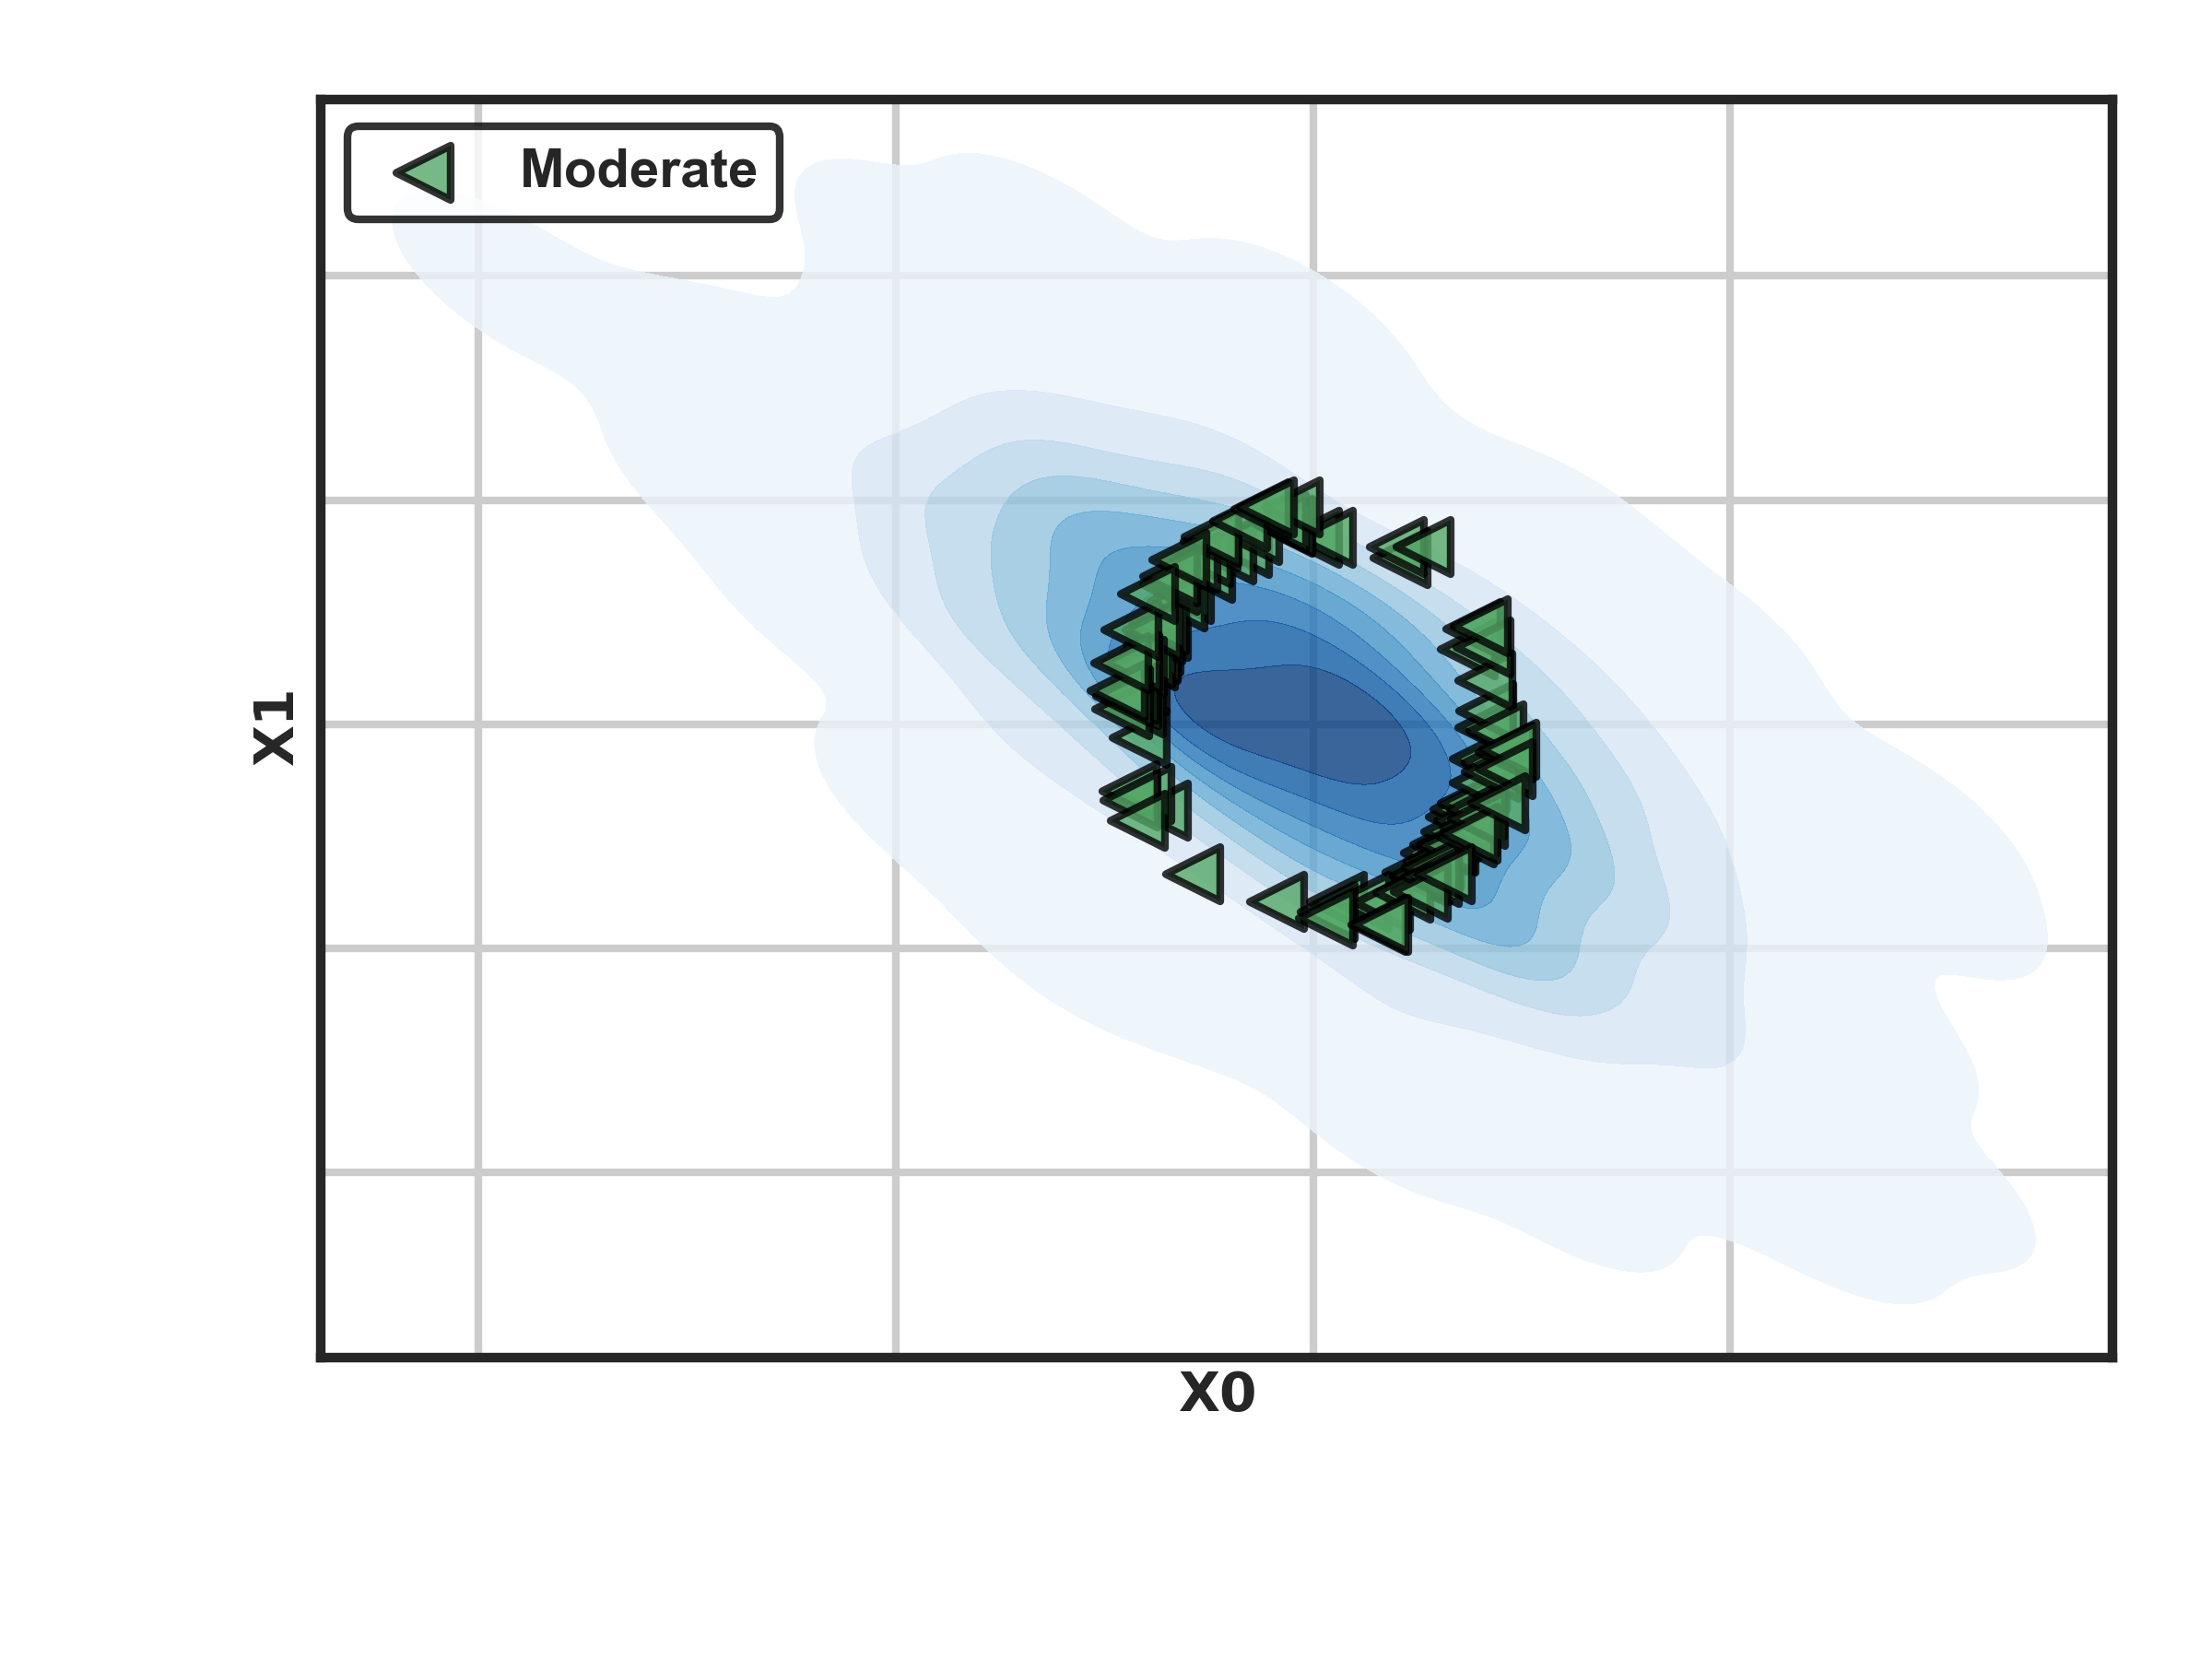}}
\subfloat[Herding]
{\includegraphics[width=0.3\textwidth]{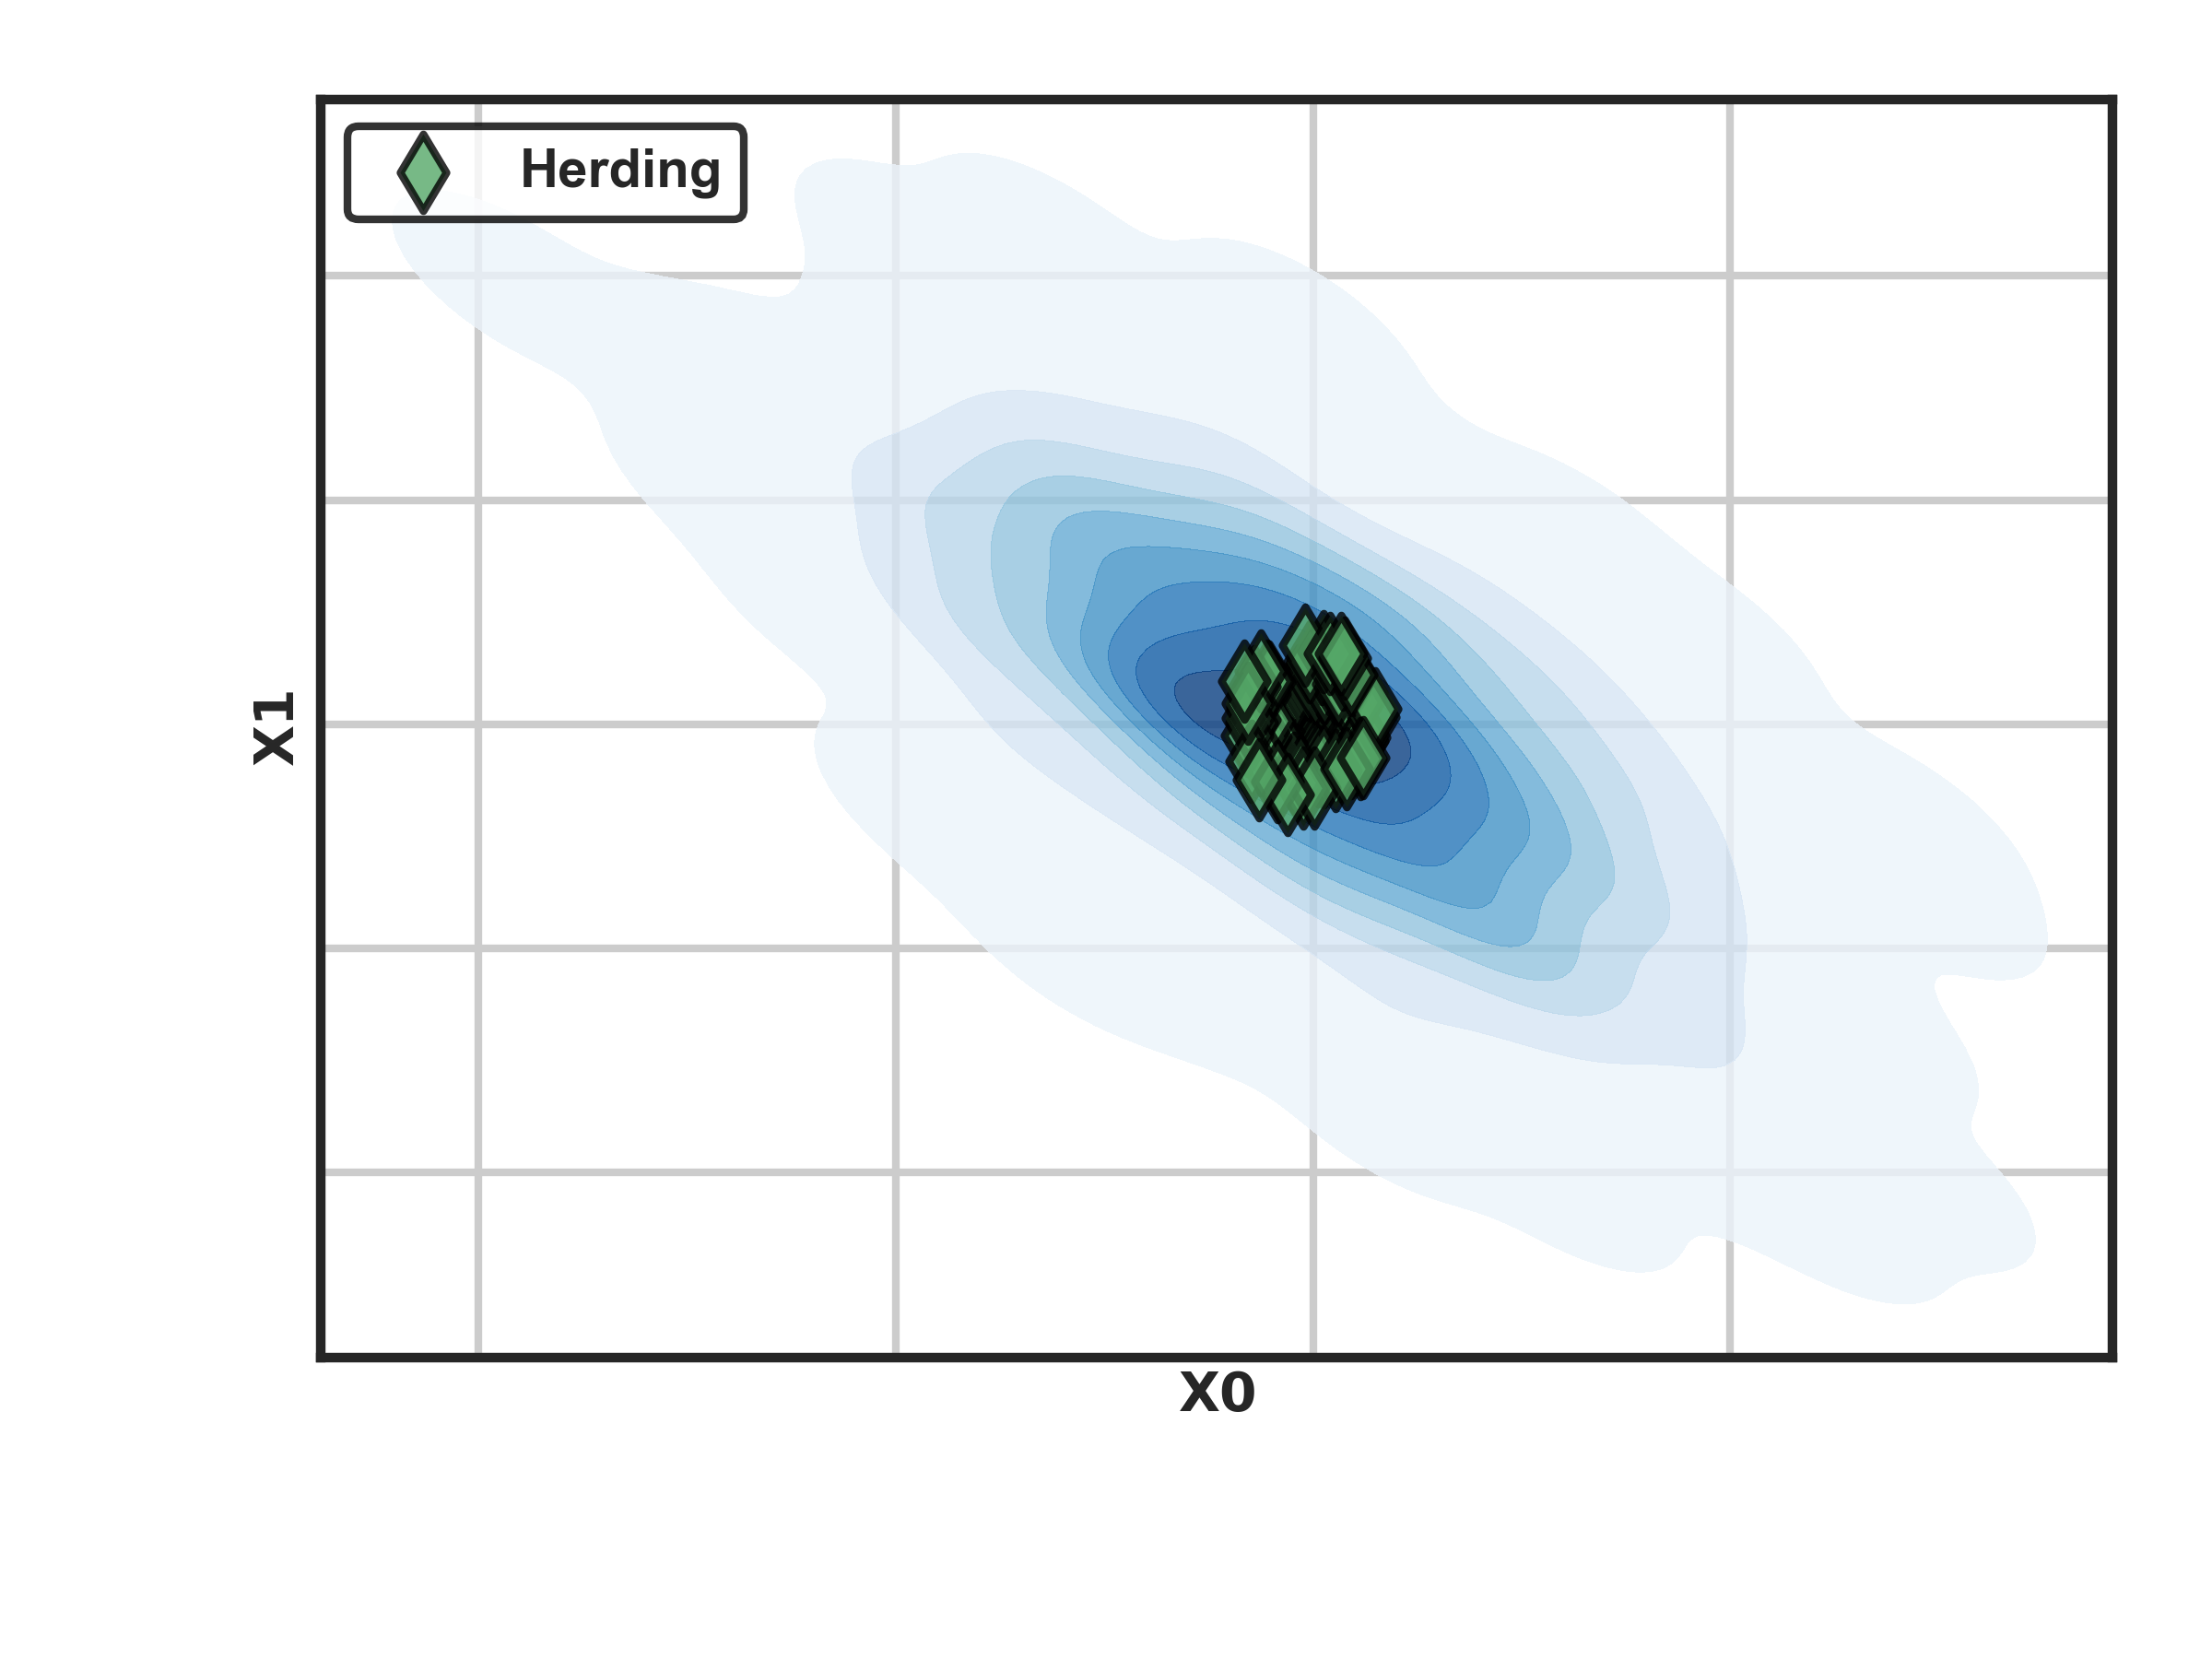}}
\subfloat[$\gmm$]
{\includegraphics[width=0.3\textwidth]{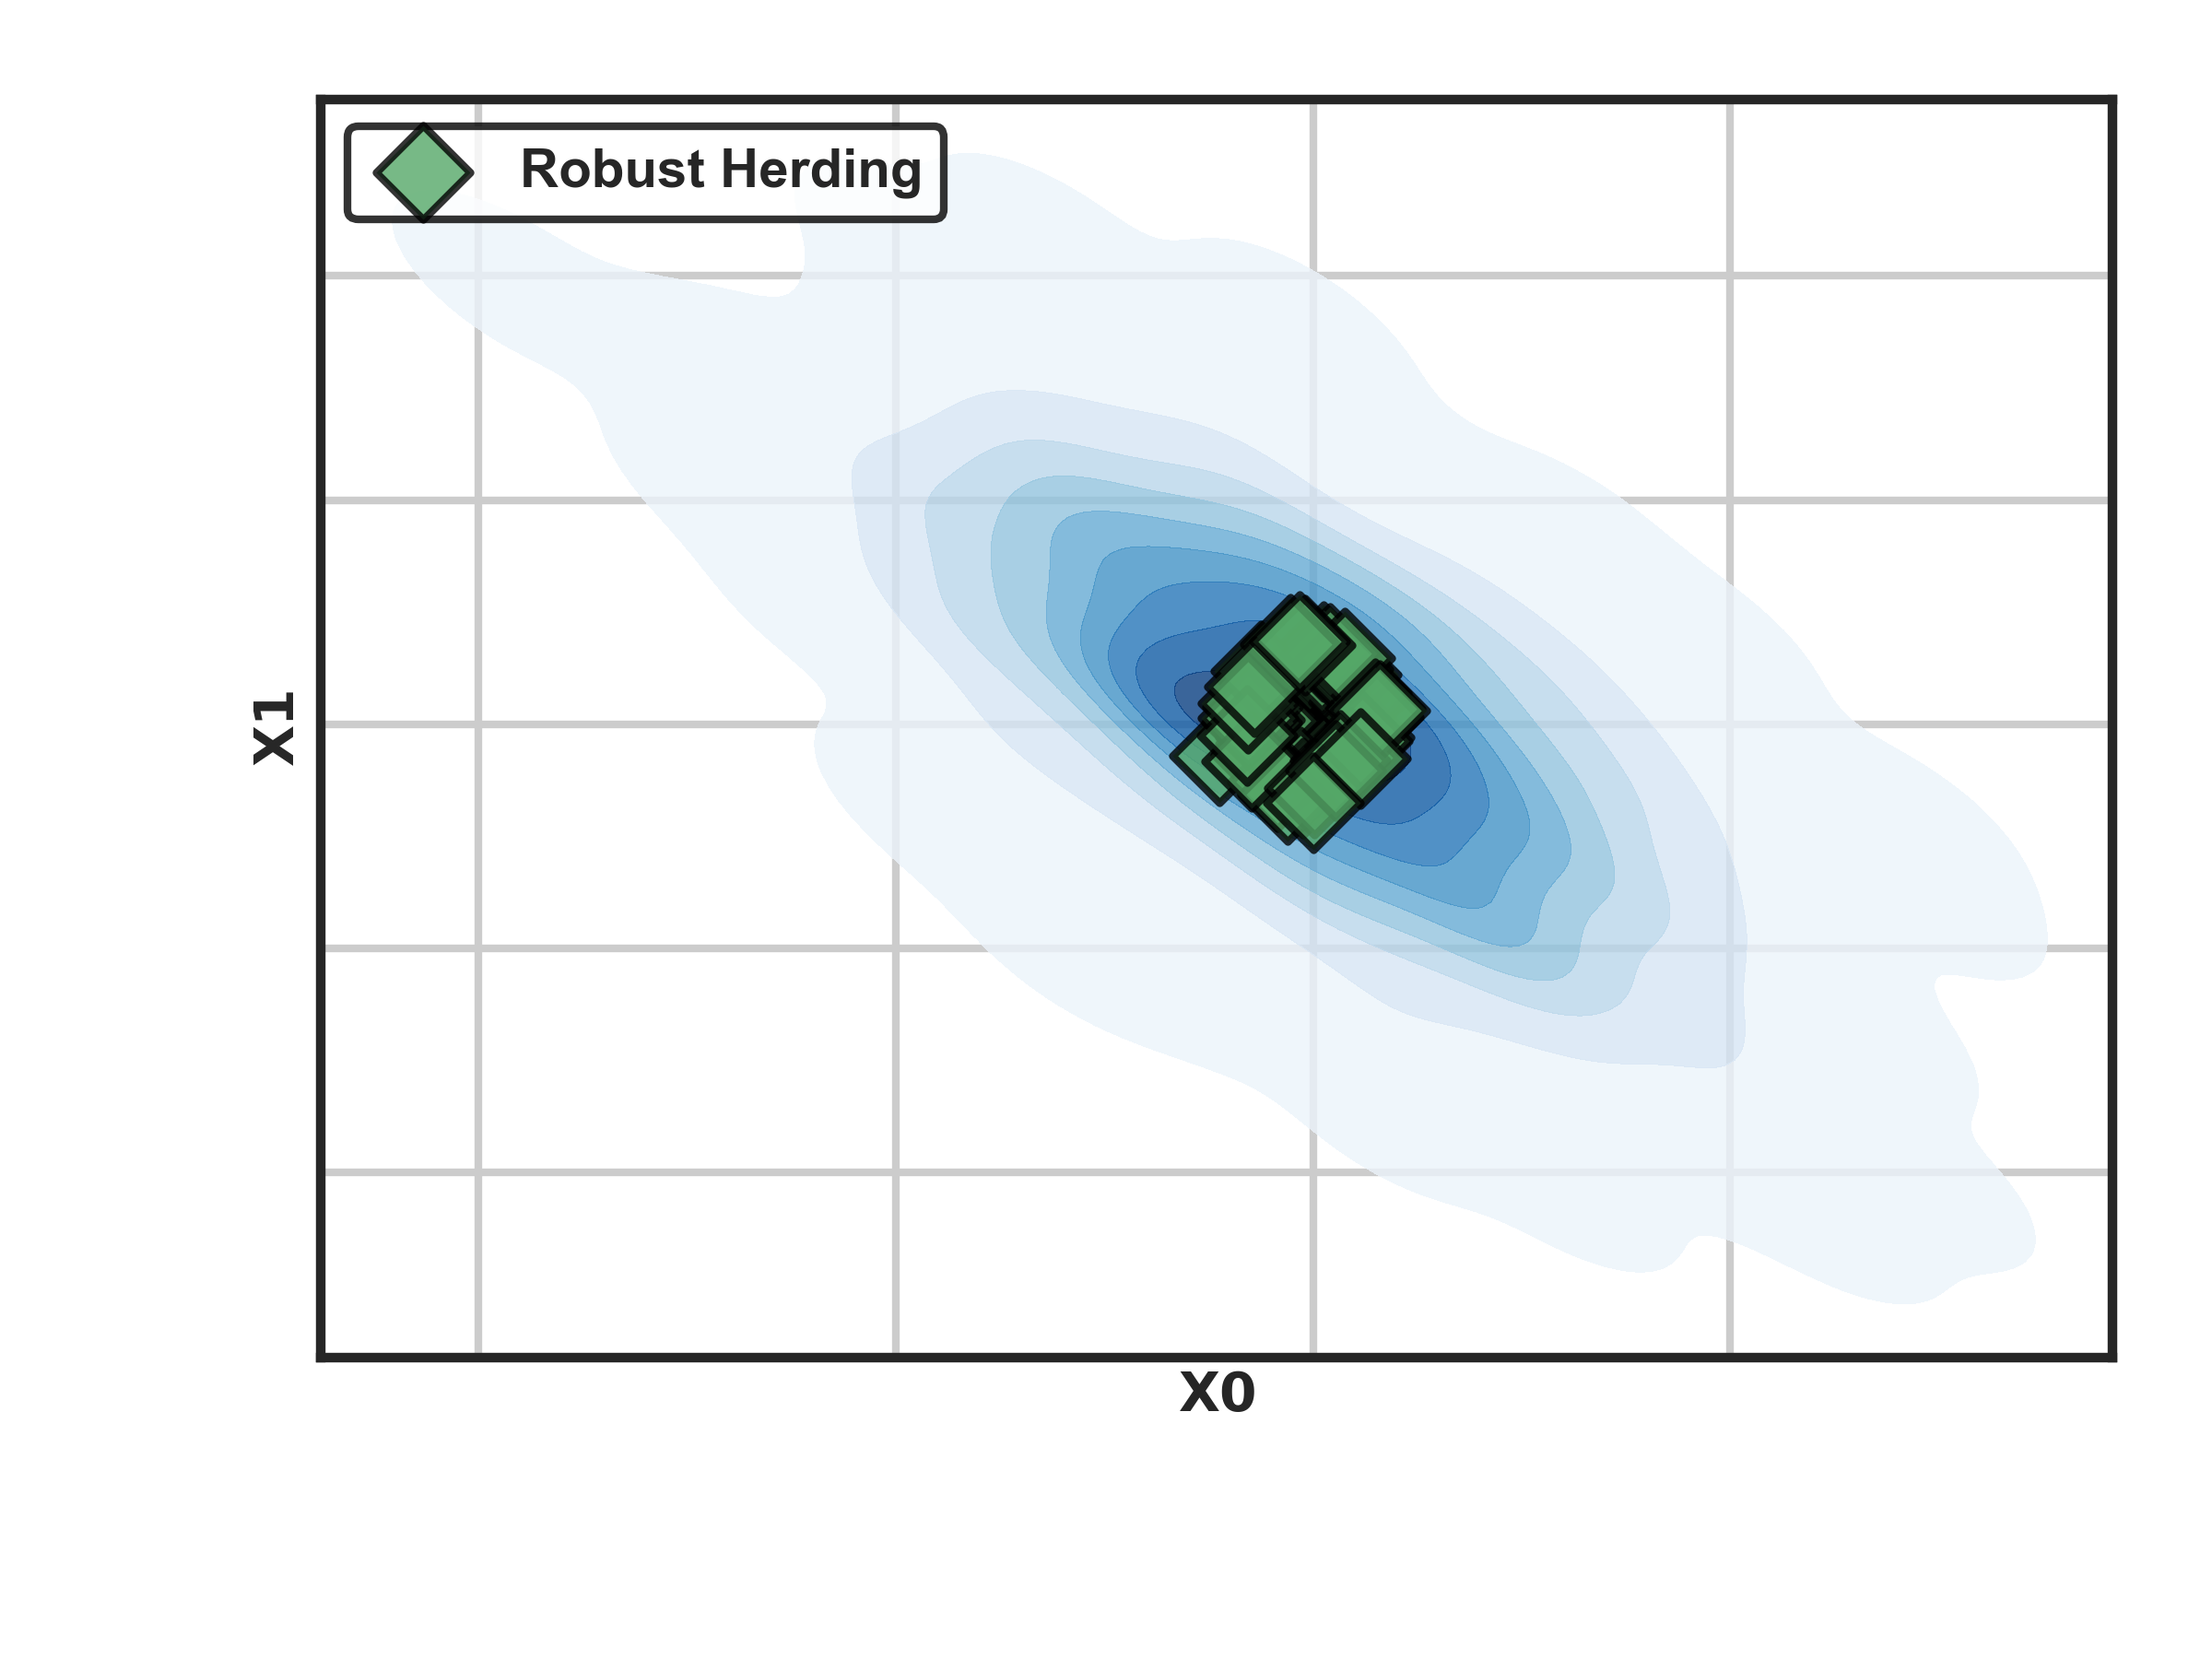}}
\caption{\footnotesize 
{\bf \textsc{(Sampling from Gaussian) No Corruption ($\psi=0$) :} 
} We subset 10\% of the samples using baseline subset selection strategies: Uniform, Easy, Hard, Moderate, Kernel Herding, \textsc{GM Matching} (\cref{sec:exp-baselines}). $\gmm$ and Kernel Herding use identity kernel map $\phi(\vx) = \vx$. 
}
\label{fig:exp-syn-corr=0}
\end{figure*}
\begin{figure*}[t]
\centering
\subfloat[Random]
{\includegraphics[width=0.3\textwidth]{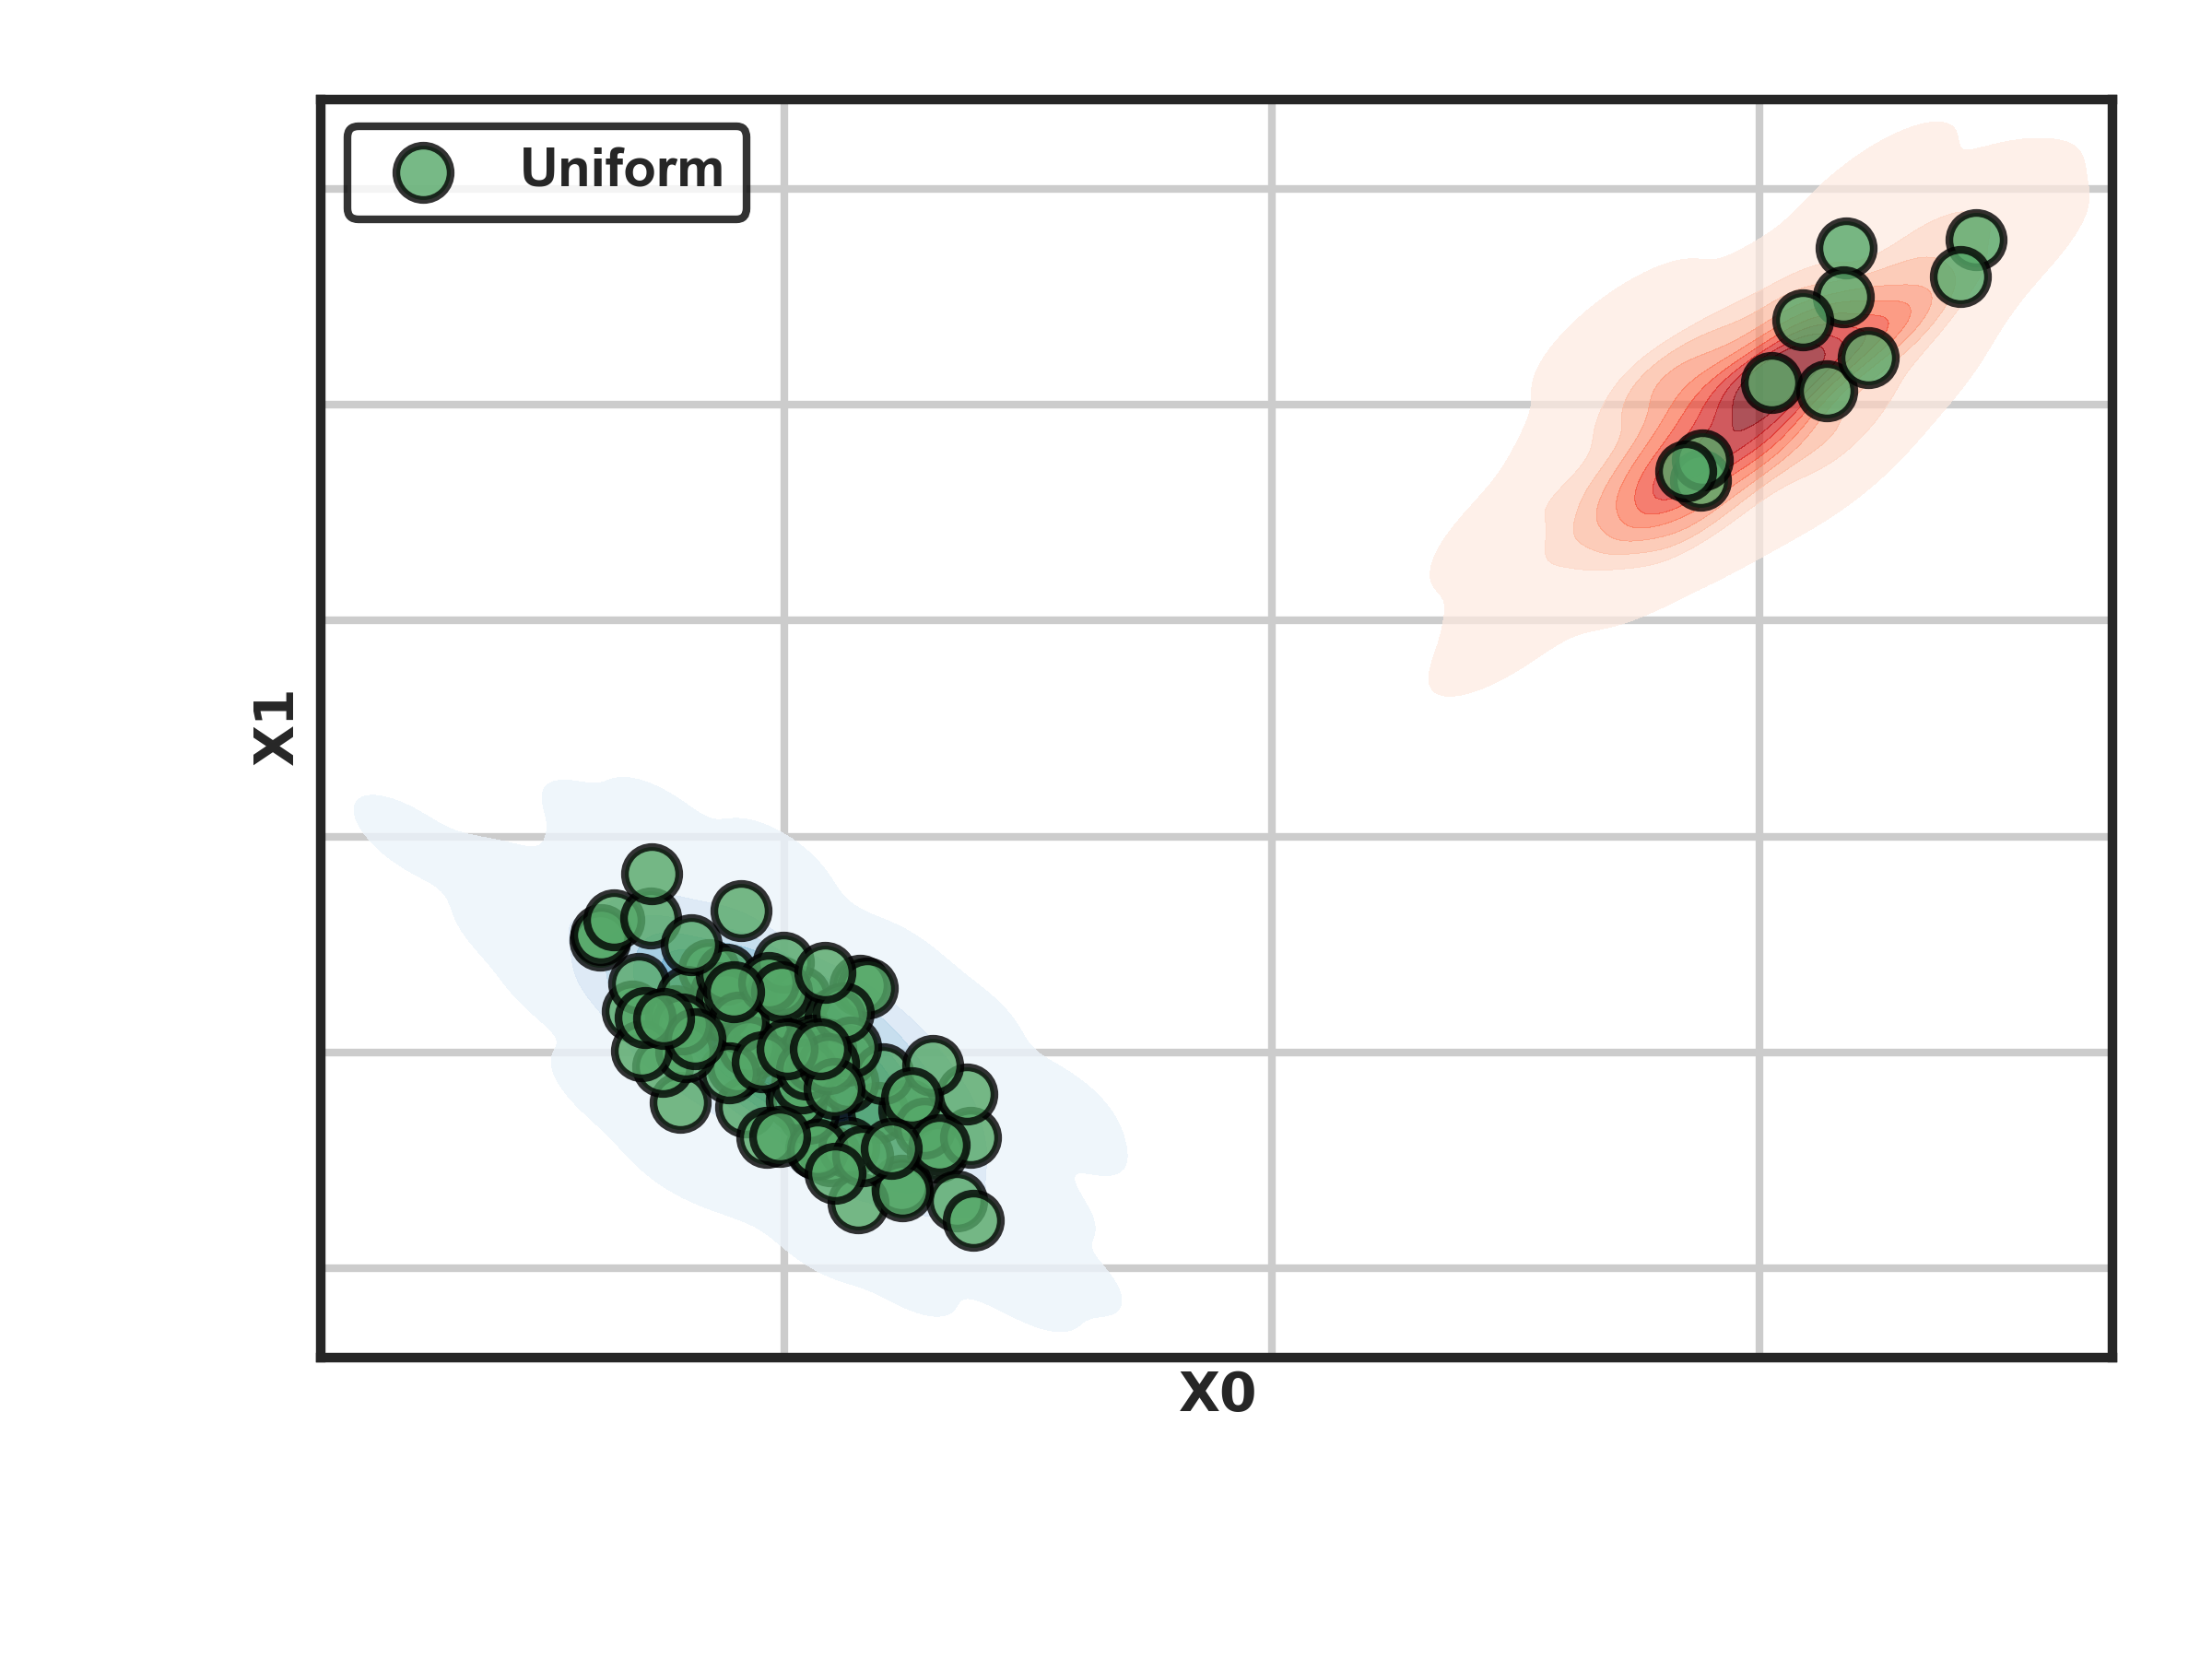}}
\subfloat[Easy]
{\includegraphics[width=0.3\textwidth]{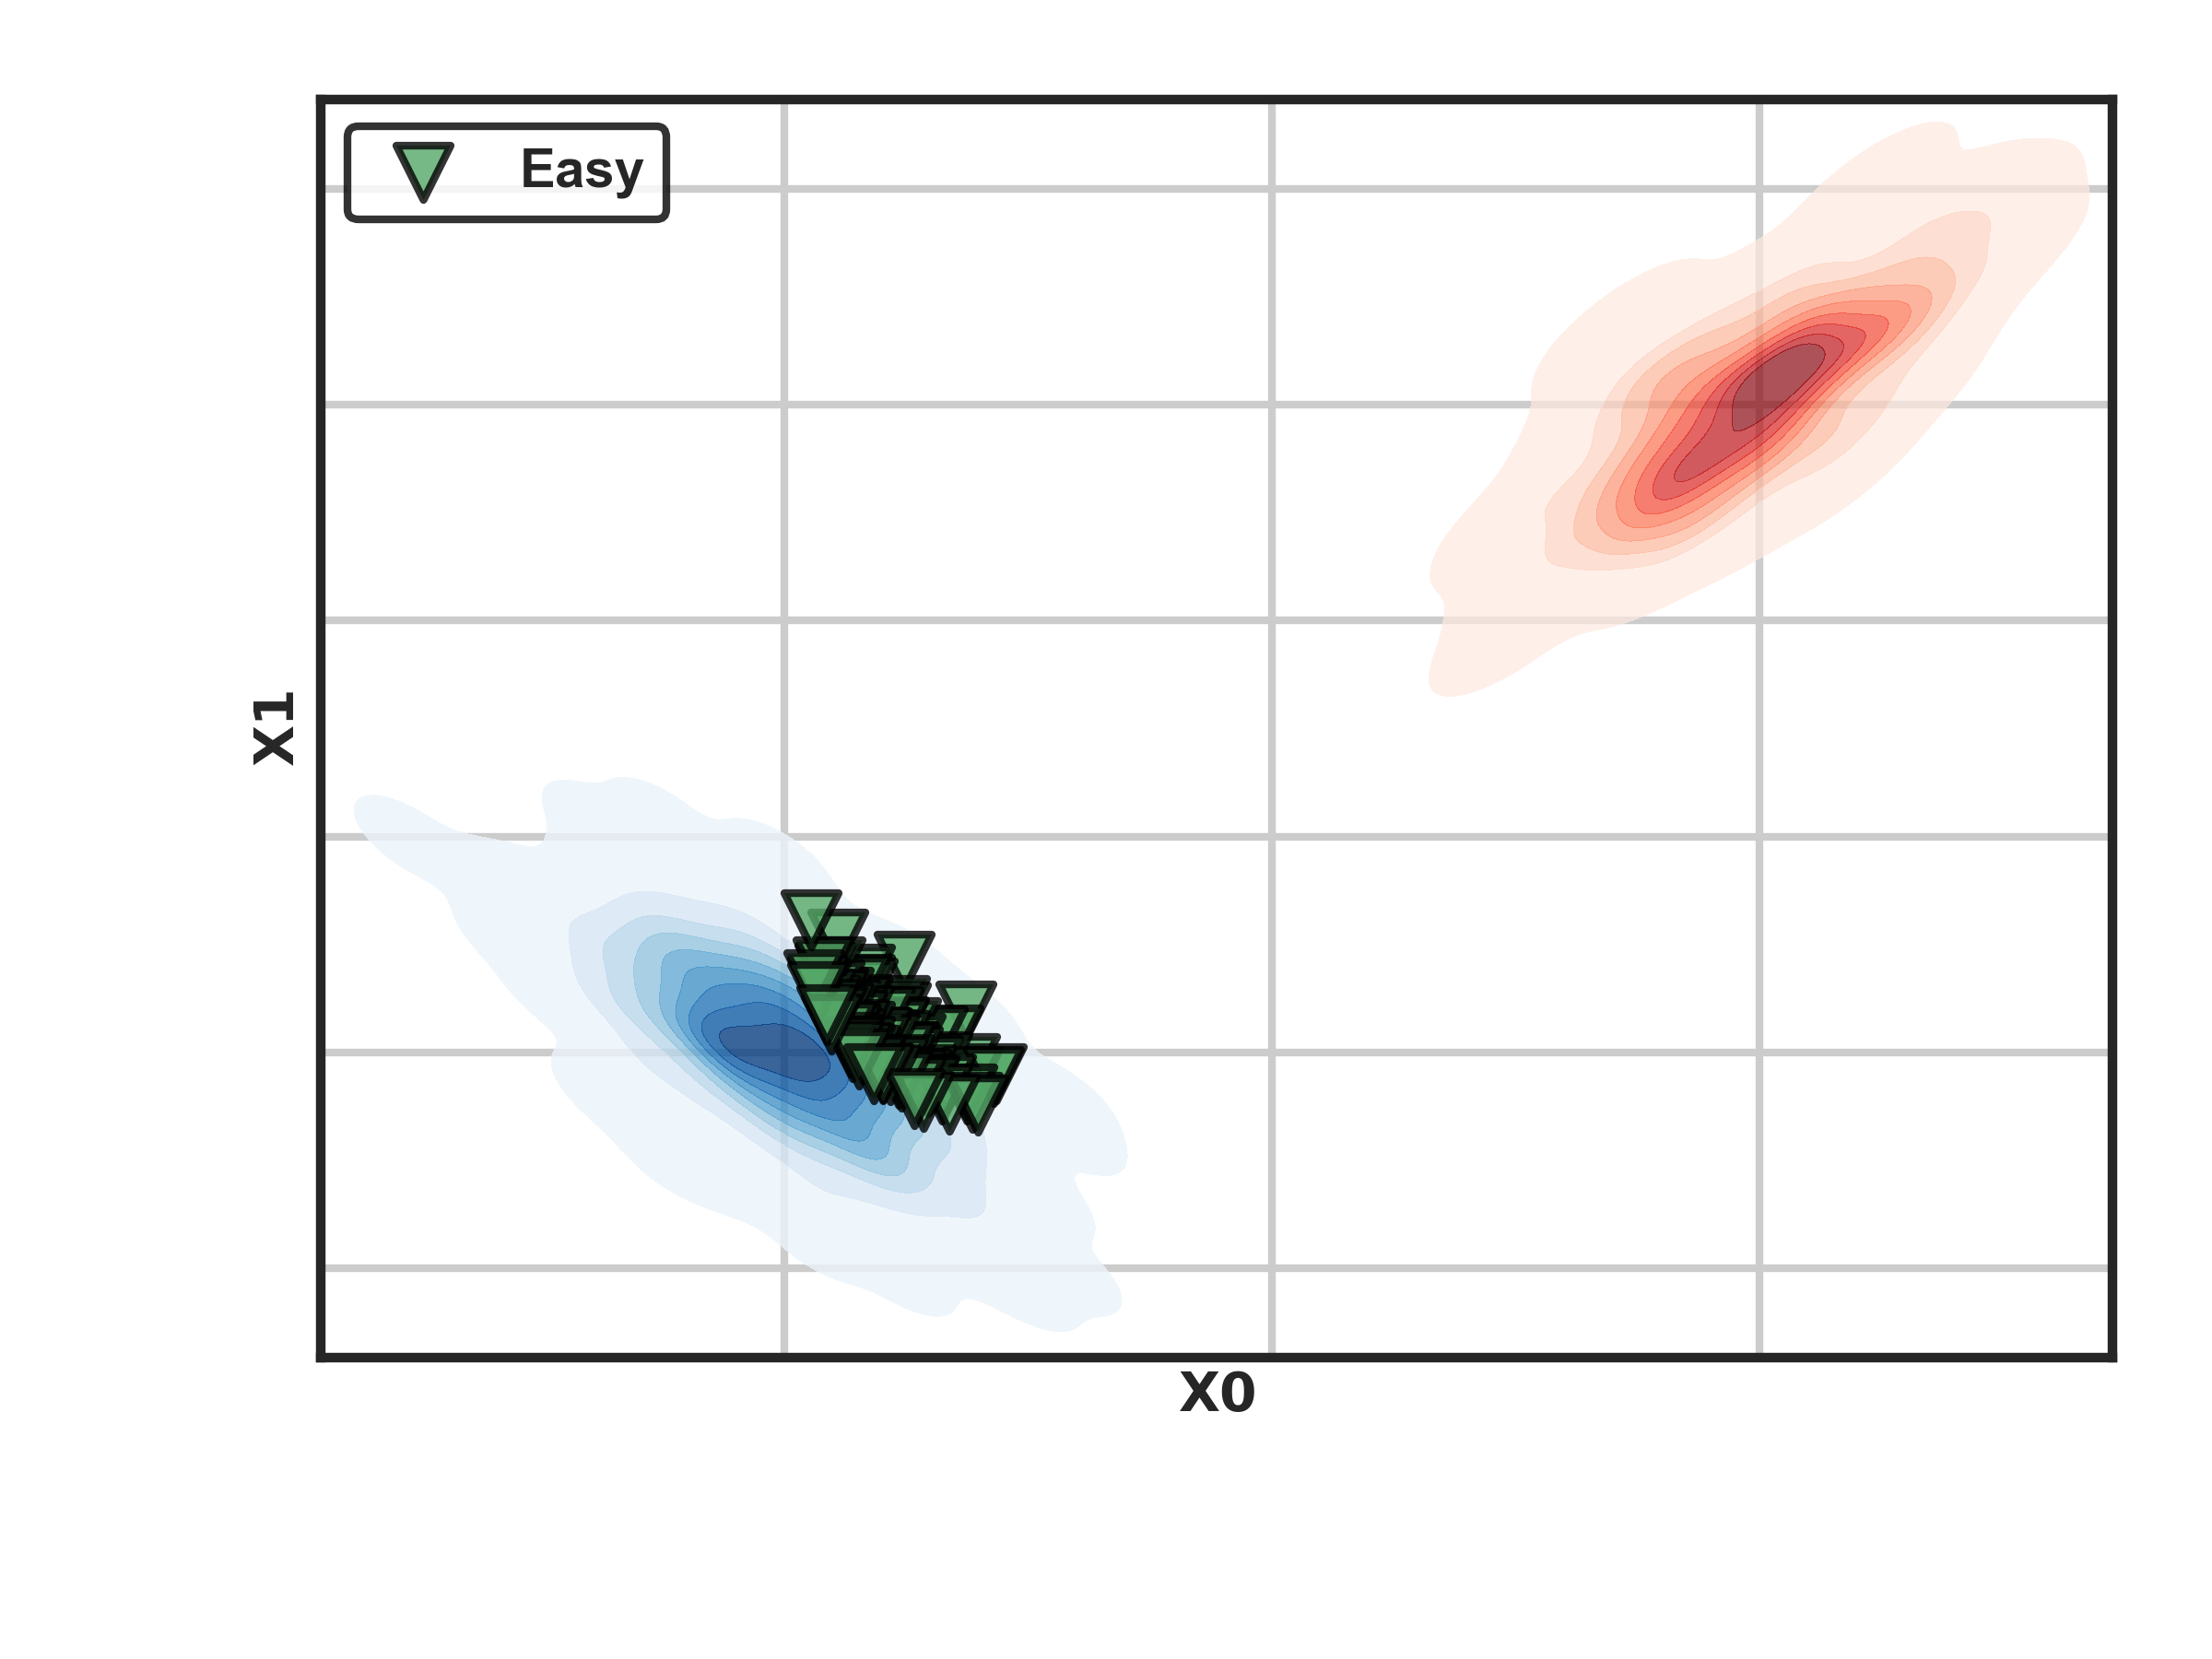}}
\subfloat[Hard]
{\includegraphics[width=0.3\textwidth]{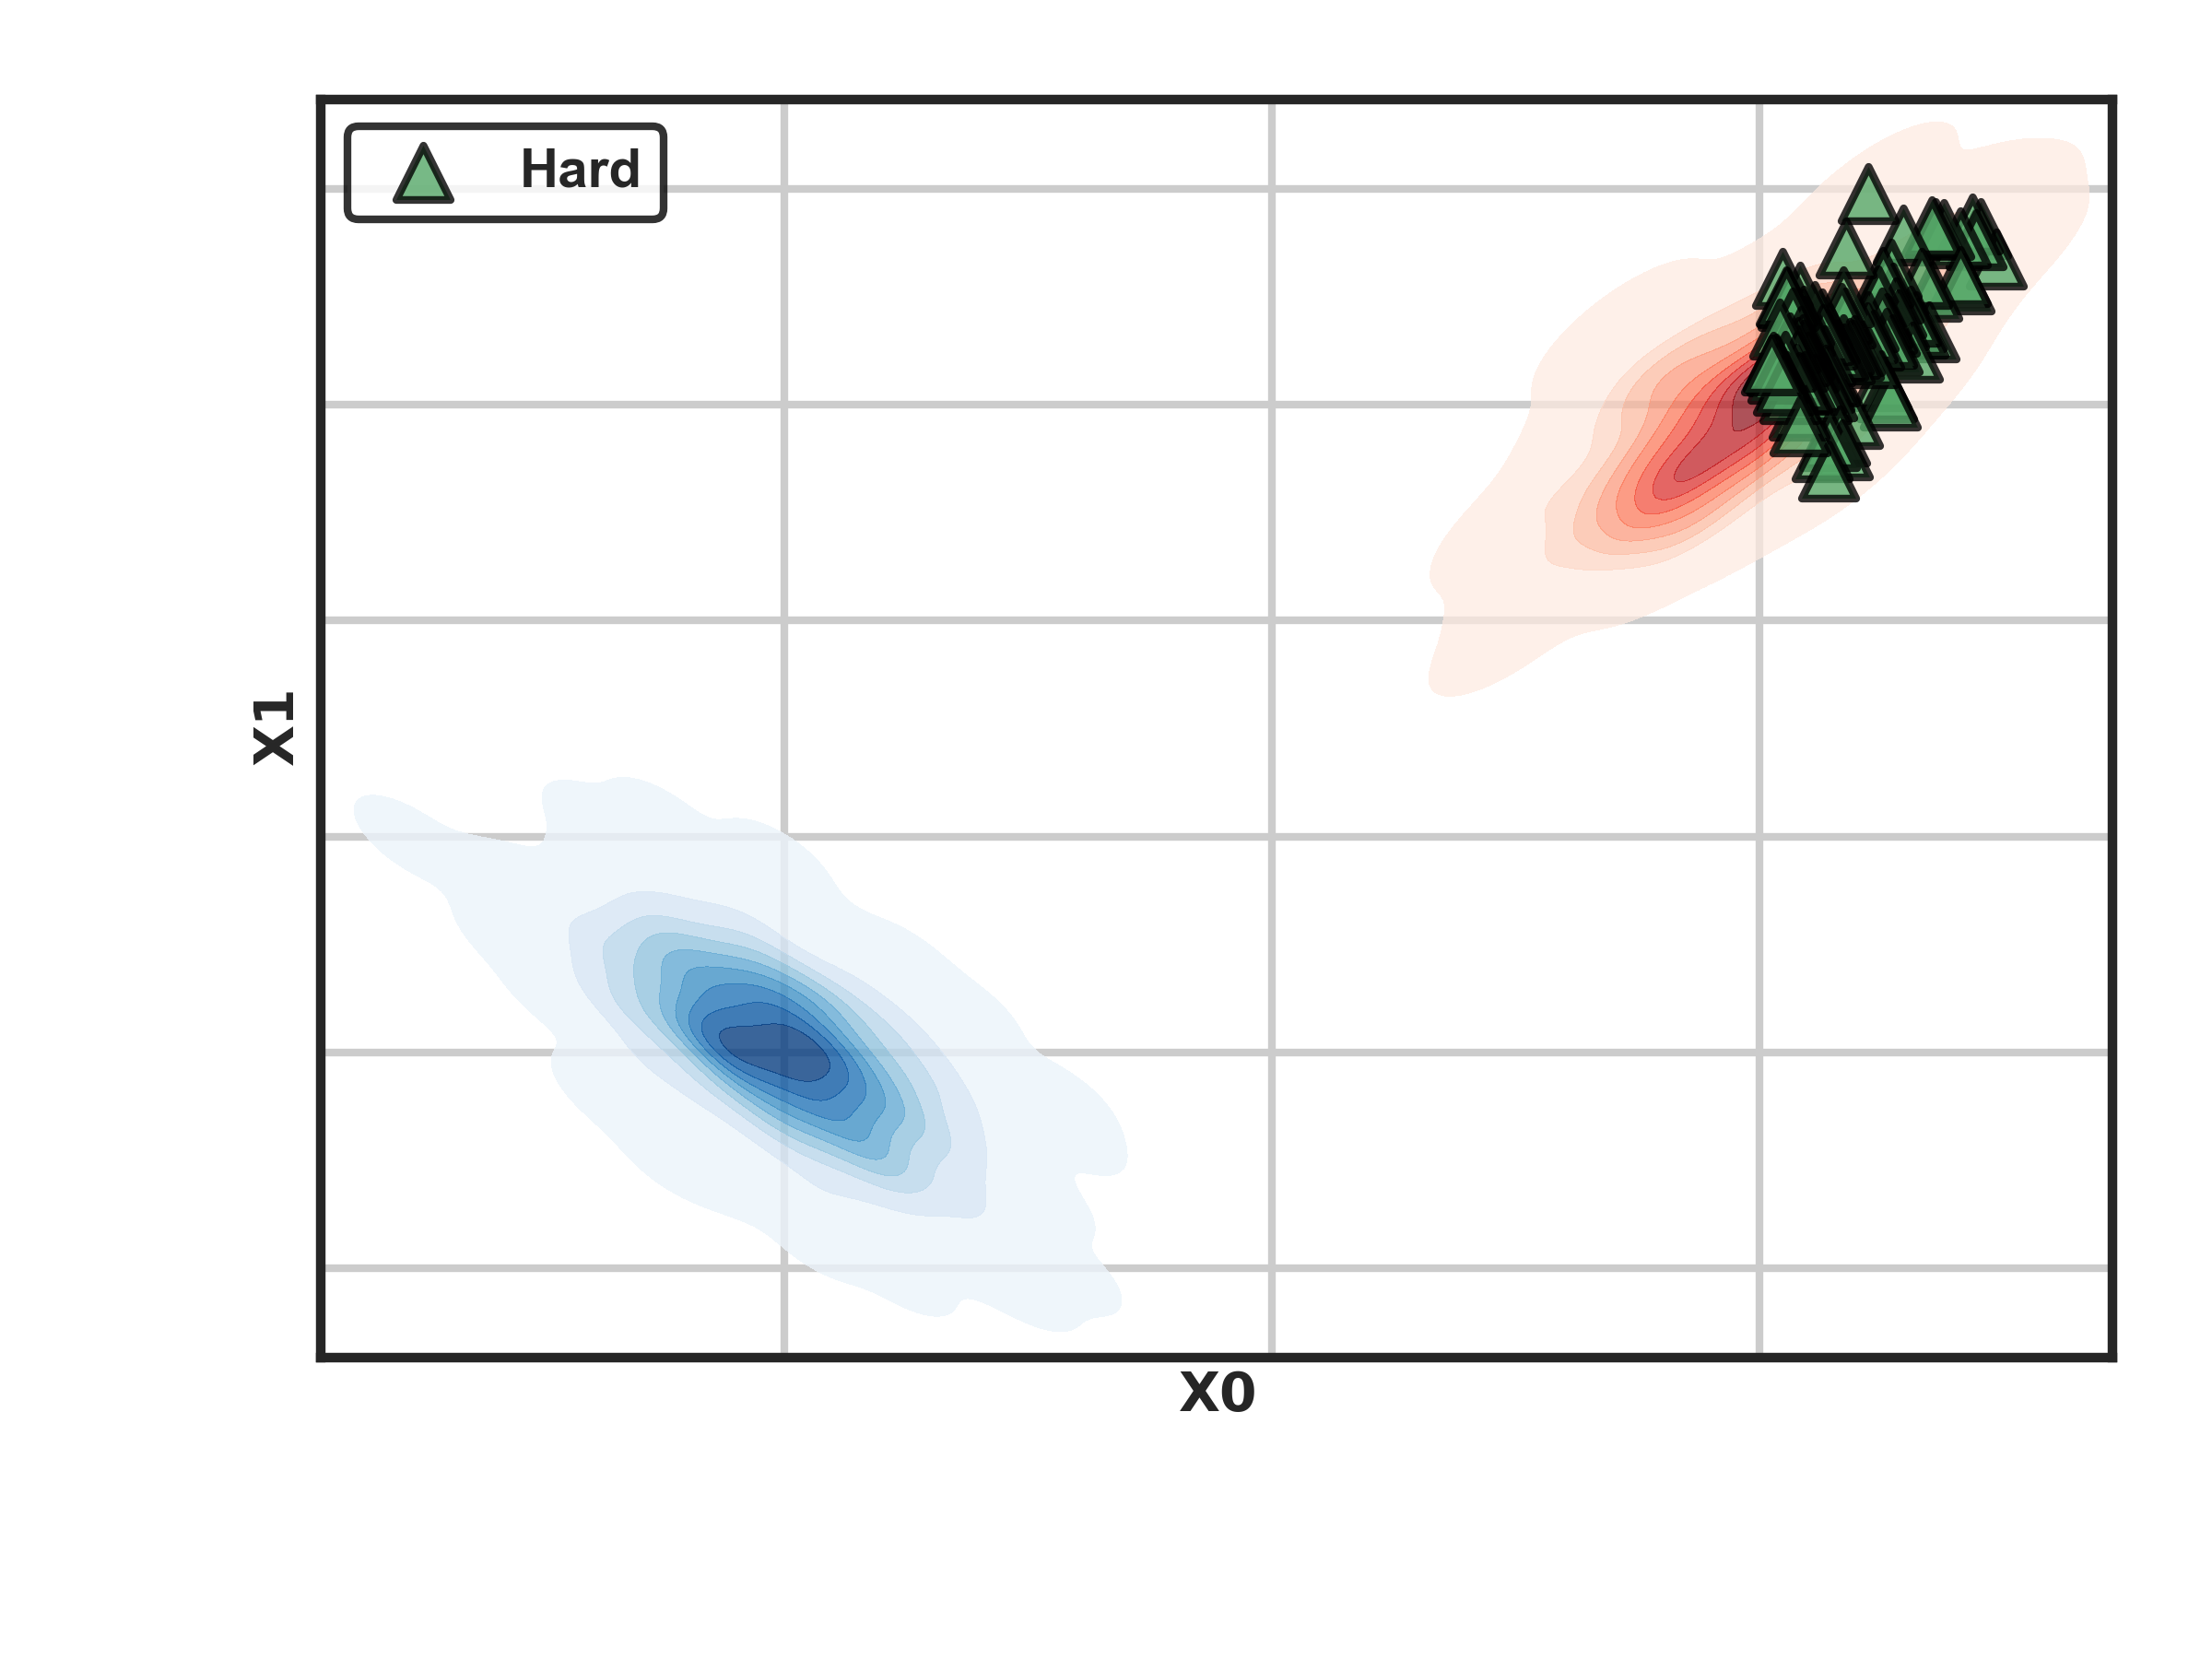}}
\\
\subfloat[Moderate]
{\includegraphics[width=0.3\textwidth]{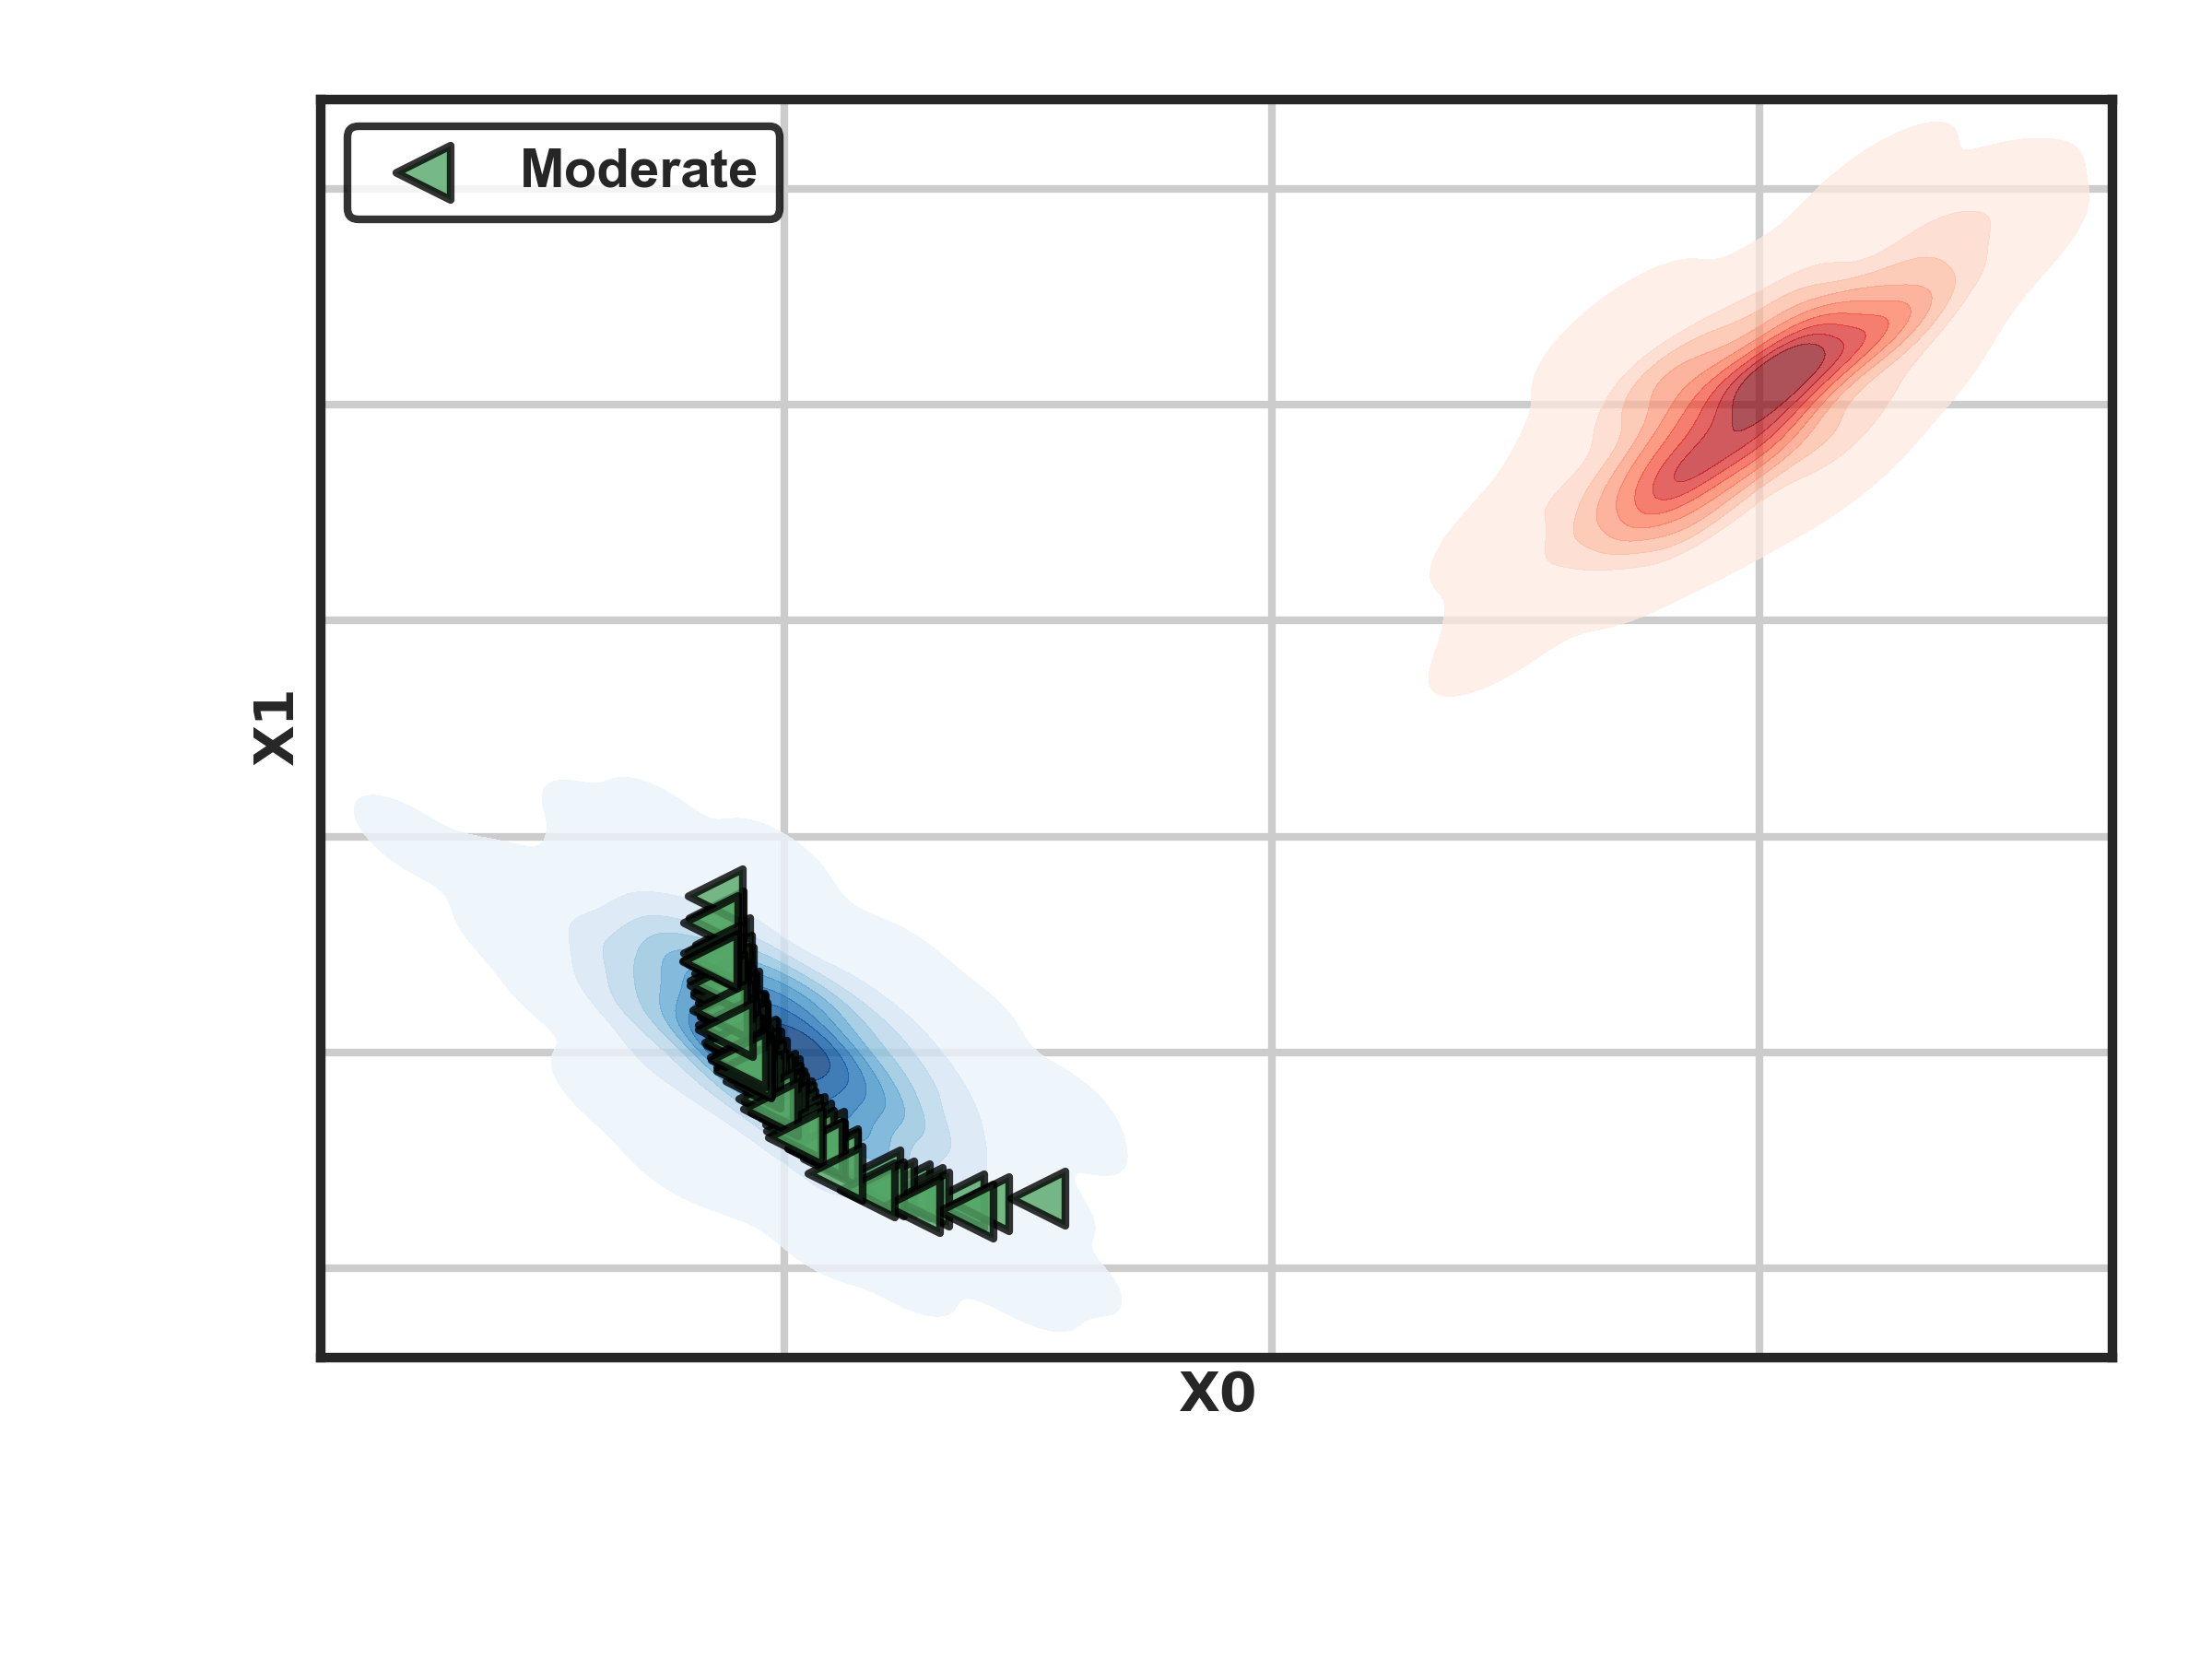}}
\subfloat[Kernel Herding]
{\includegraphics[width=0.3\textwidth]{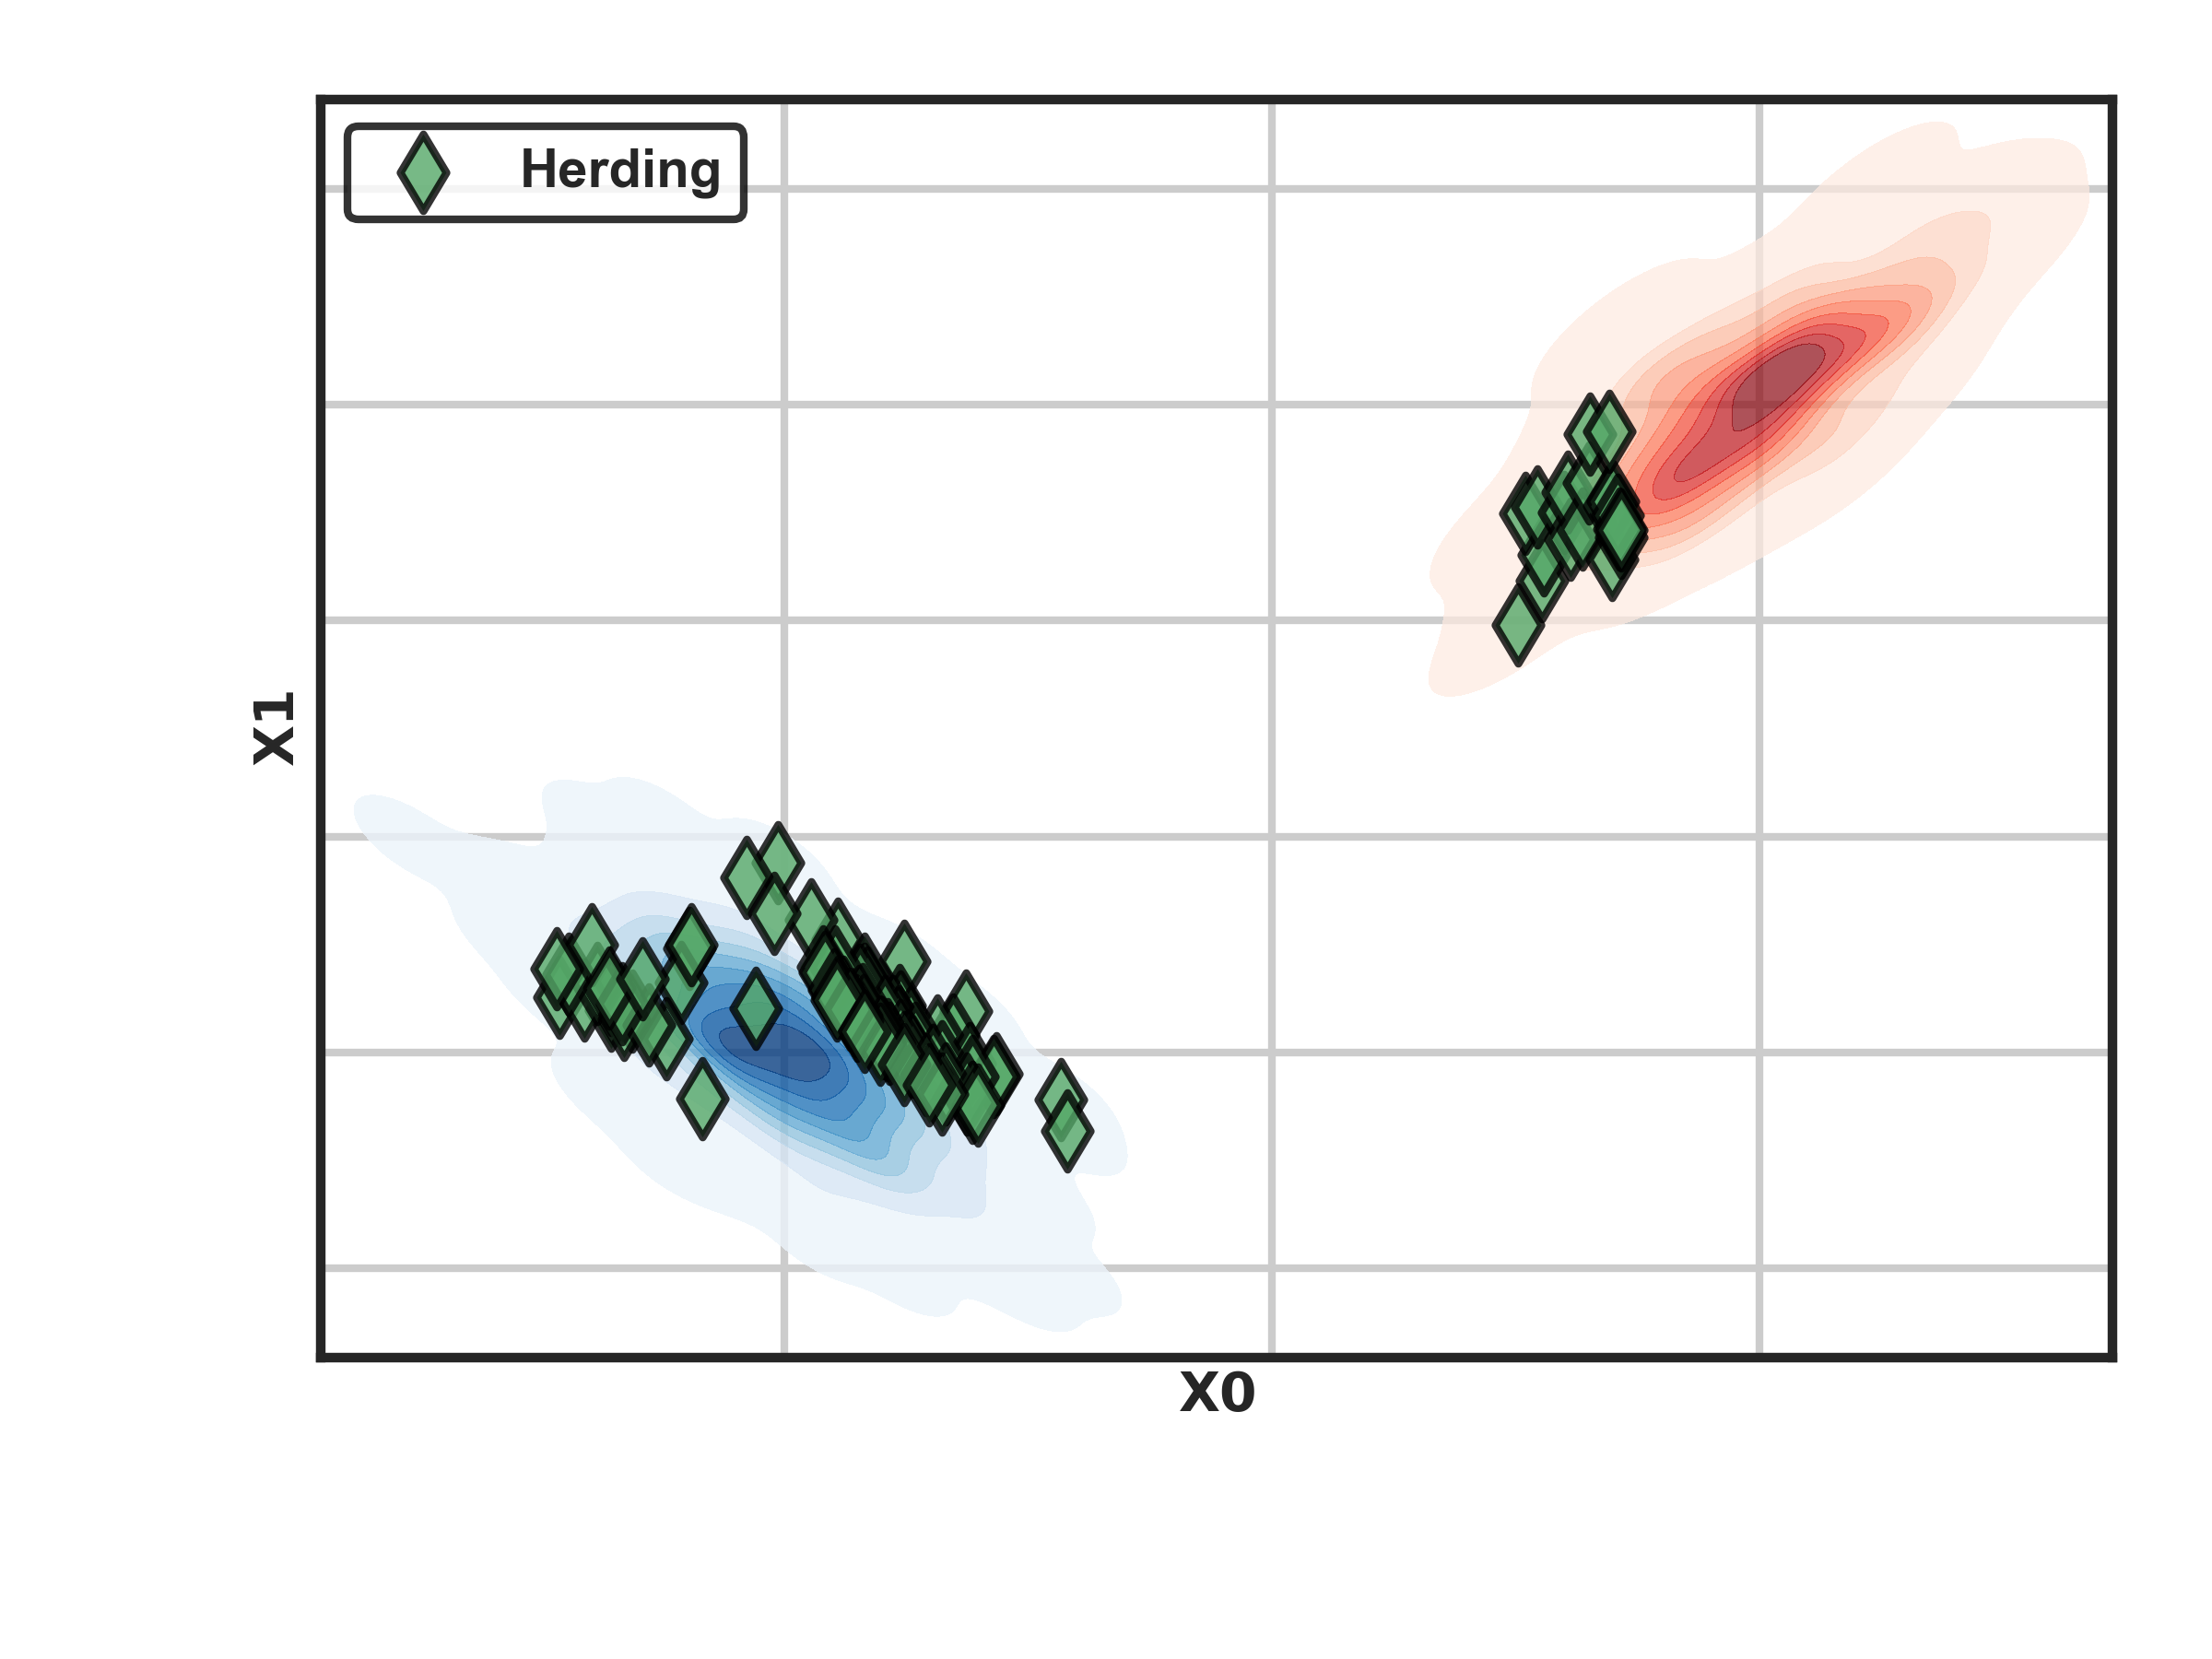}}
\subfloat[$\gmm$]
{\includegraphics[width=0.3\textwidth]{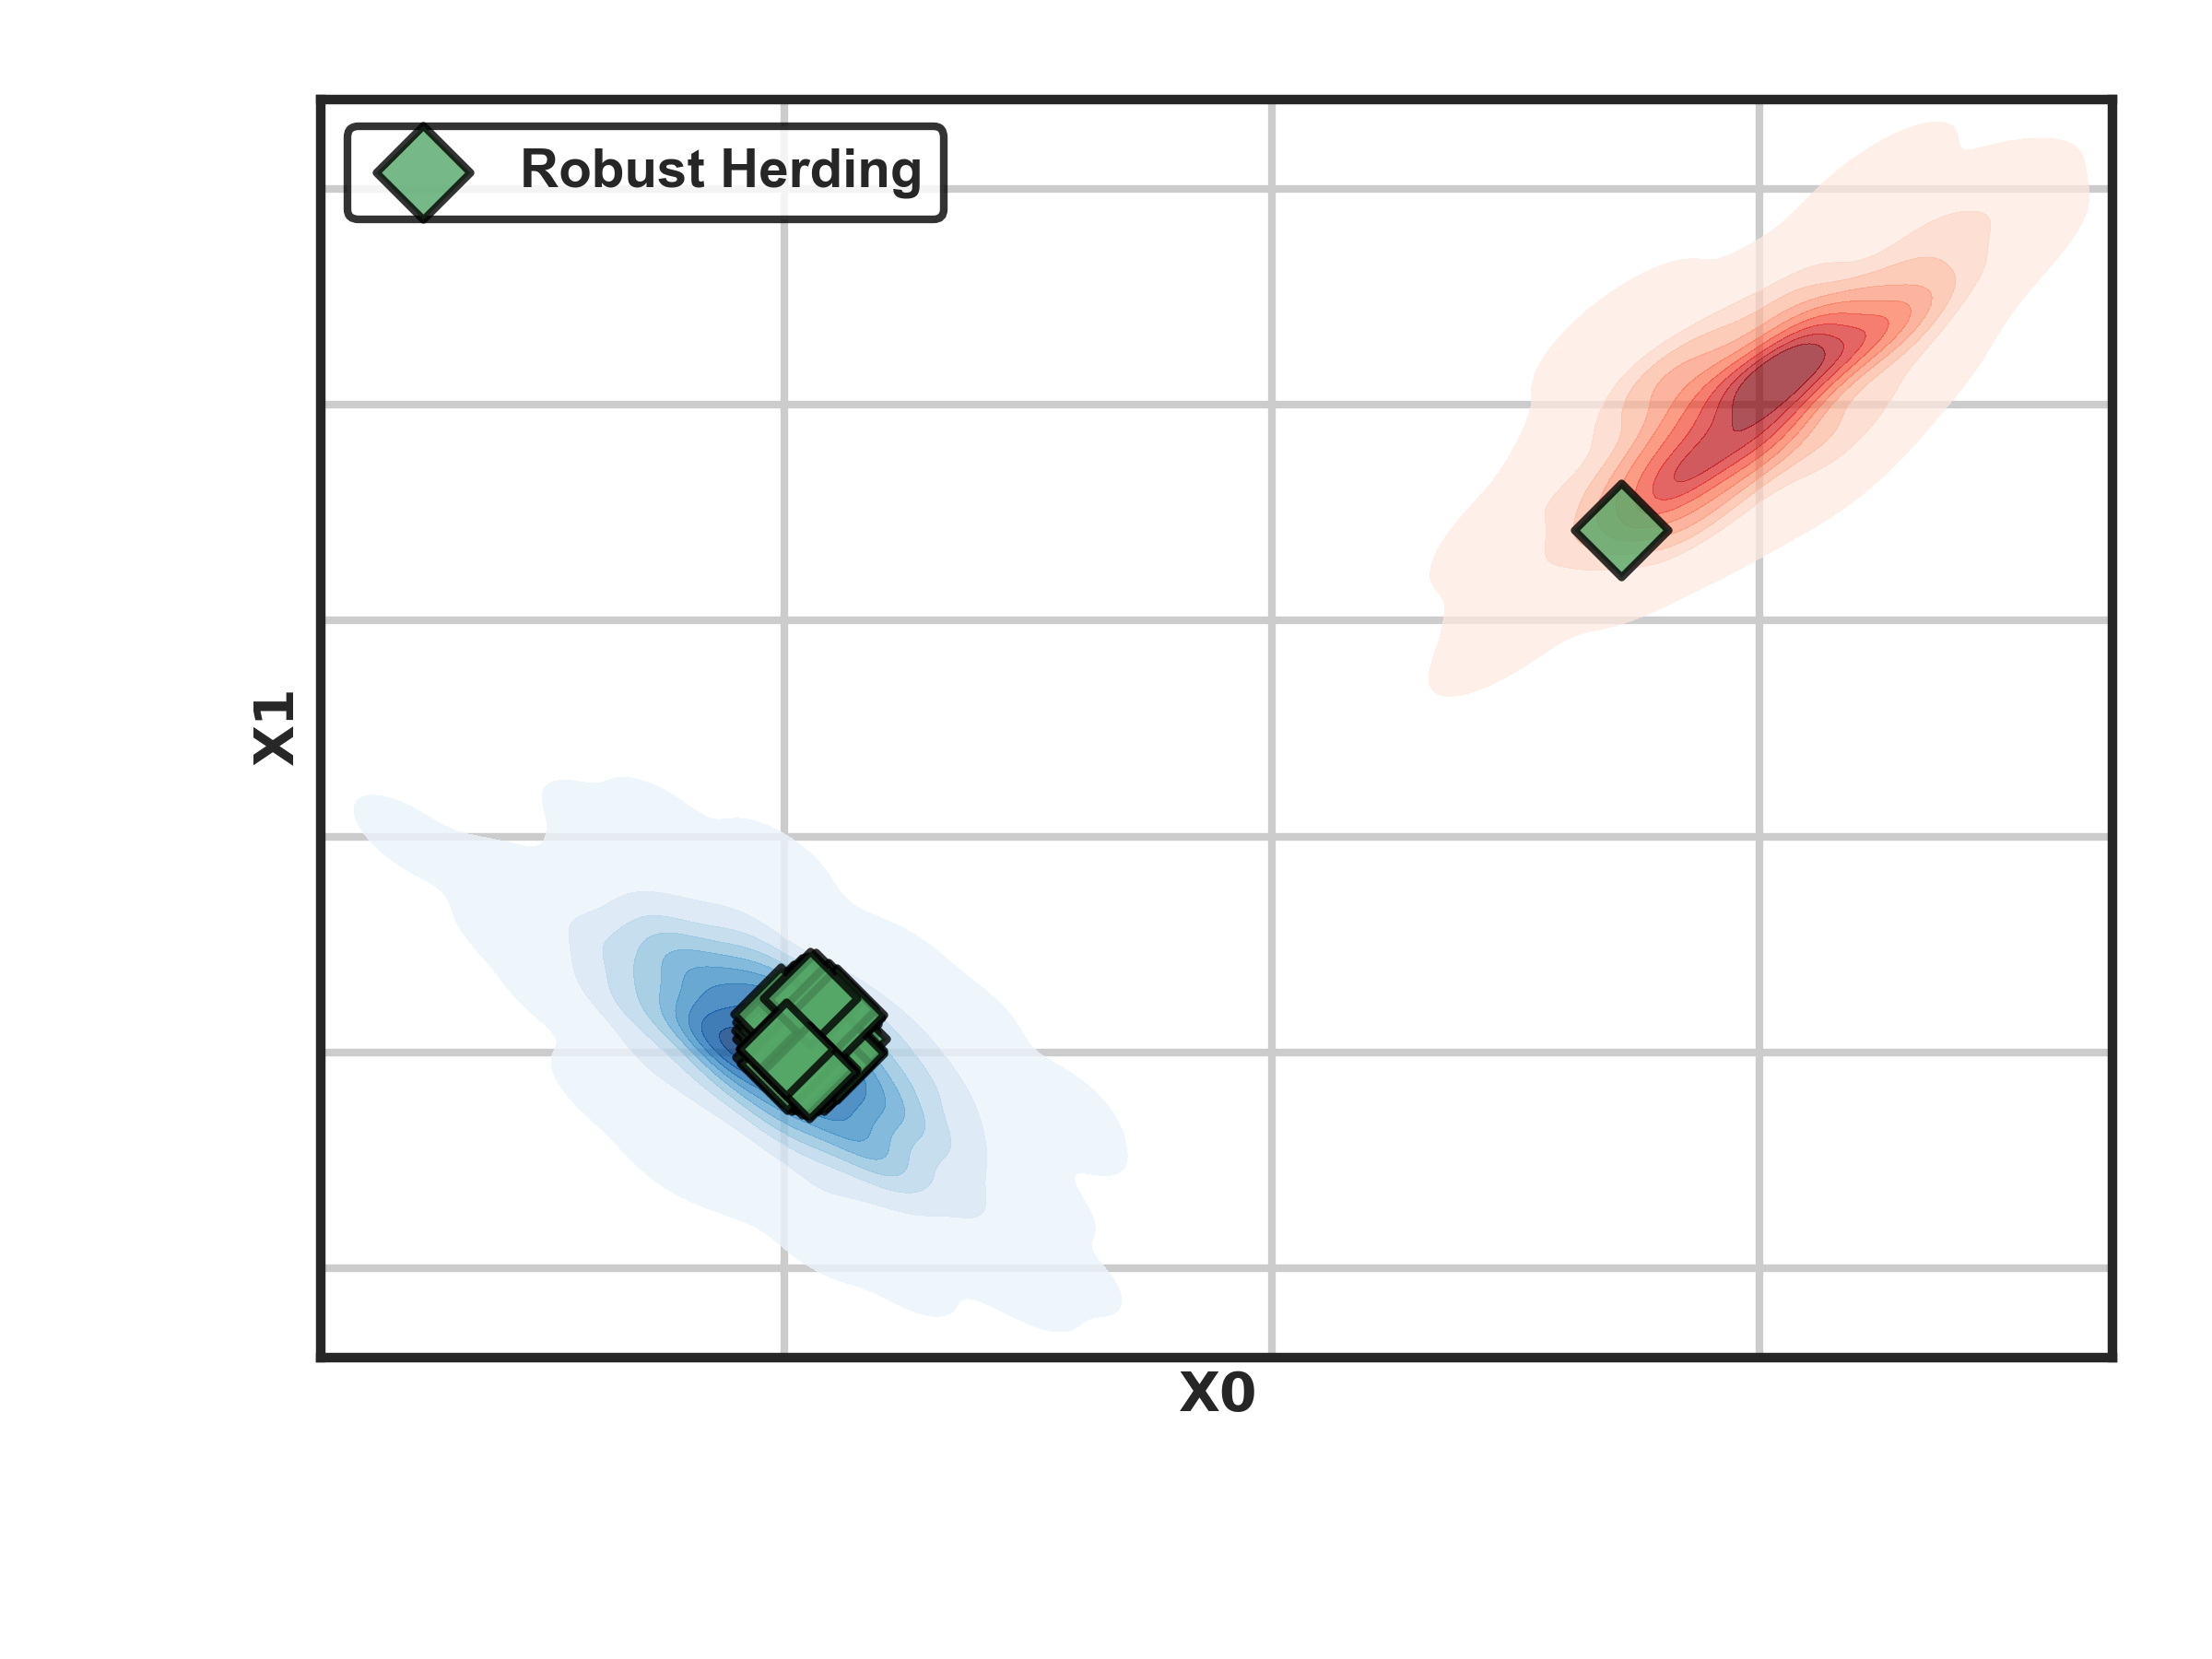}}
\caption{\footnotesize {\bf \textsc{(Sampling from Noisy Gaussian) 20\% Corruption ($\psi=0.2$)}}: In this experiment, 20\% of the samples are corrupted -- drawn from a adversary chosen distribution (red). We select 10\% samples baseline subset selection strategies: Uniform, Easy, Hard, Moderate, Kernel Herding, \textsc{GM Matching} (\cref{sec:exp-baselines}). $\gmm$ and Kernel Herding are performed using an identity kernel map $\phi(\vx) = \vx$. We see that while Easy remains robust, it is clearly sampling from low-density areas -- failing to capture the prototypical samples.}
\label{fig:exp-syn-corr=20}
\end{figure*}
\begin{figure*}[t] 
\centering
\subfloat[Random]
{\includegraphics[width=0.3\textwidth]{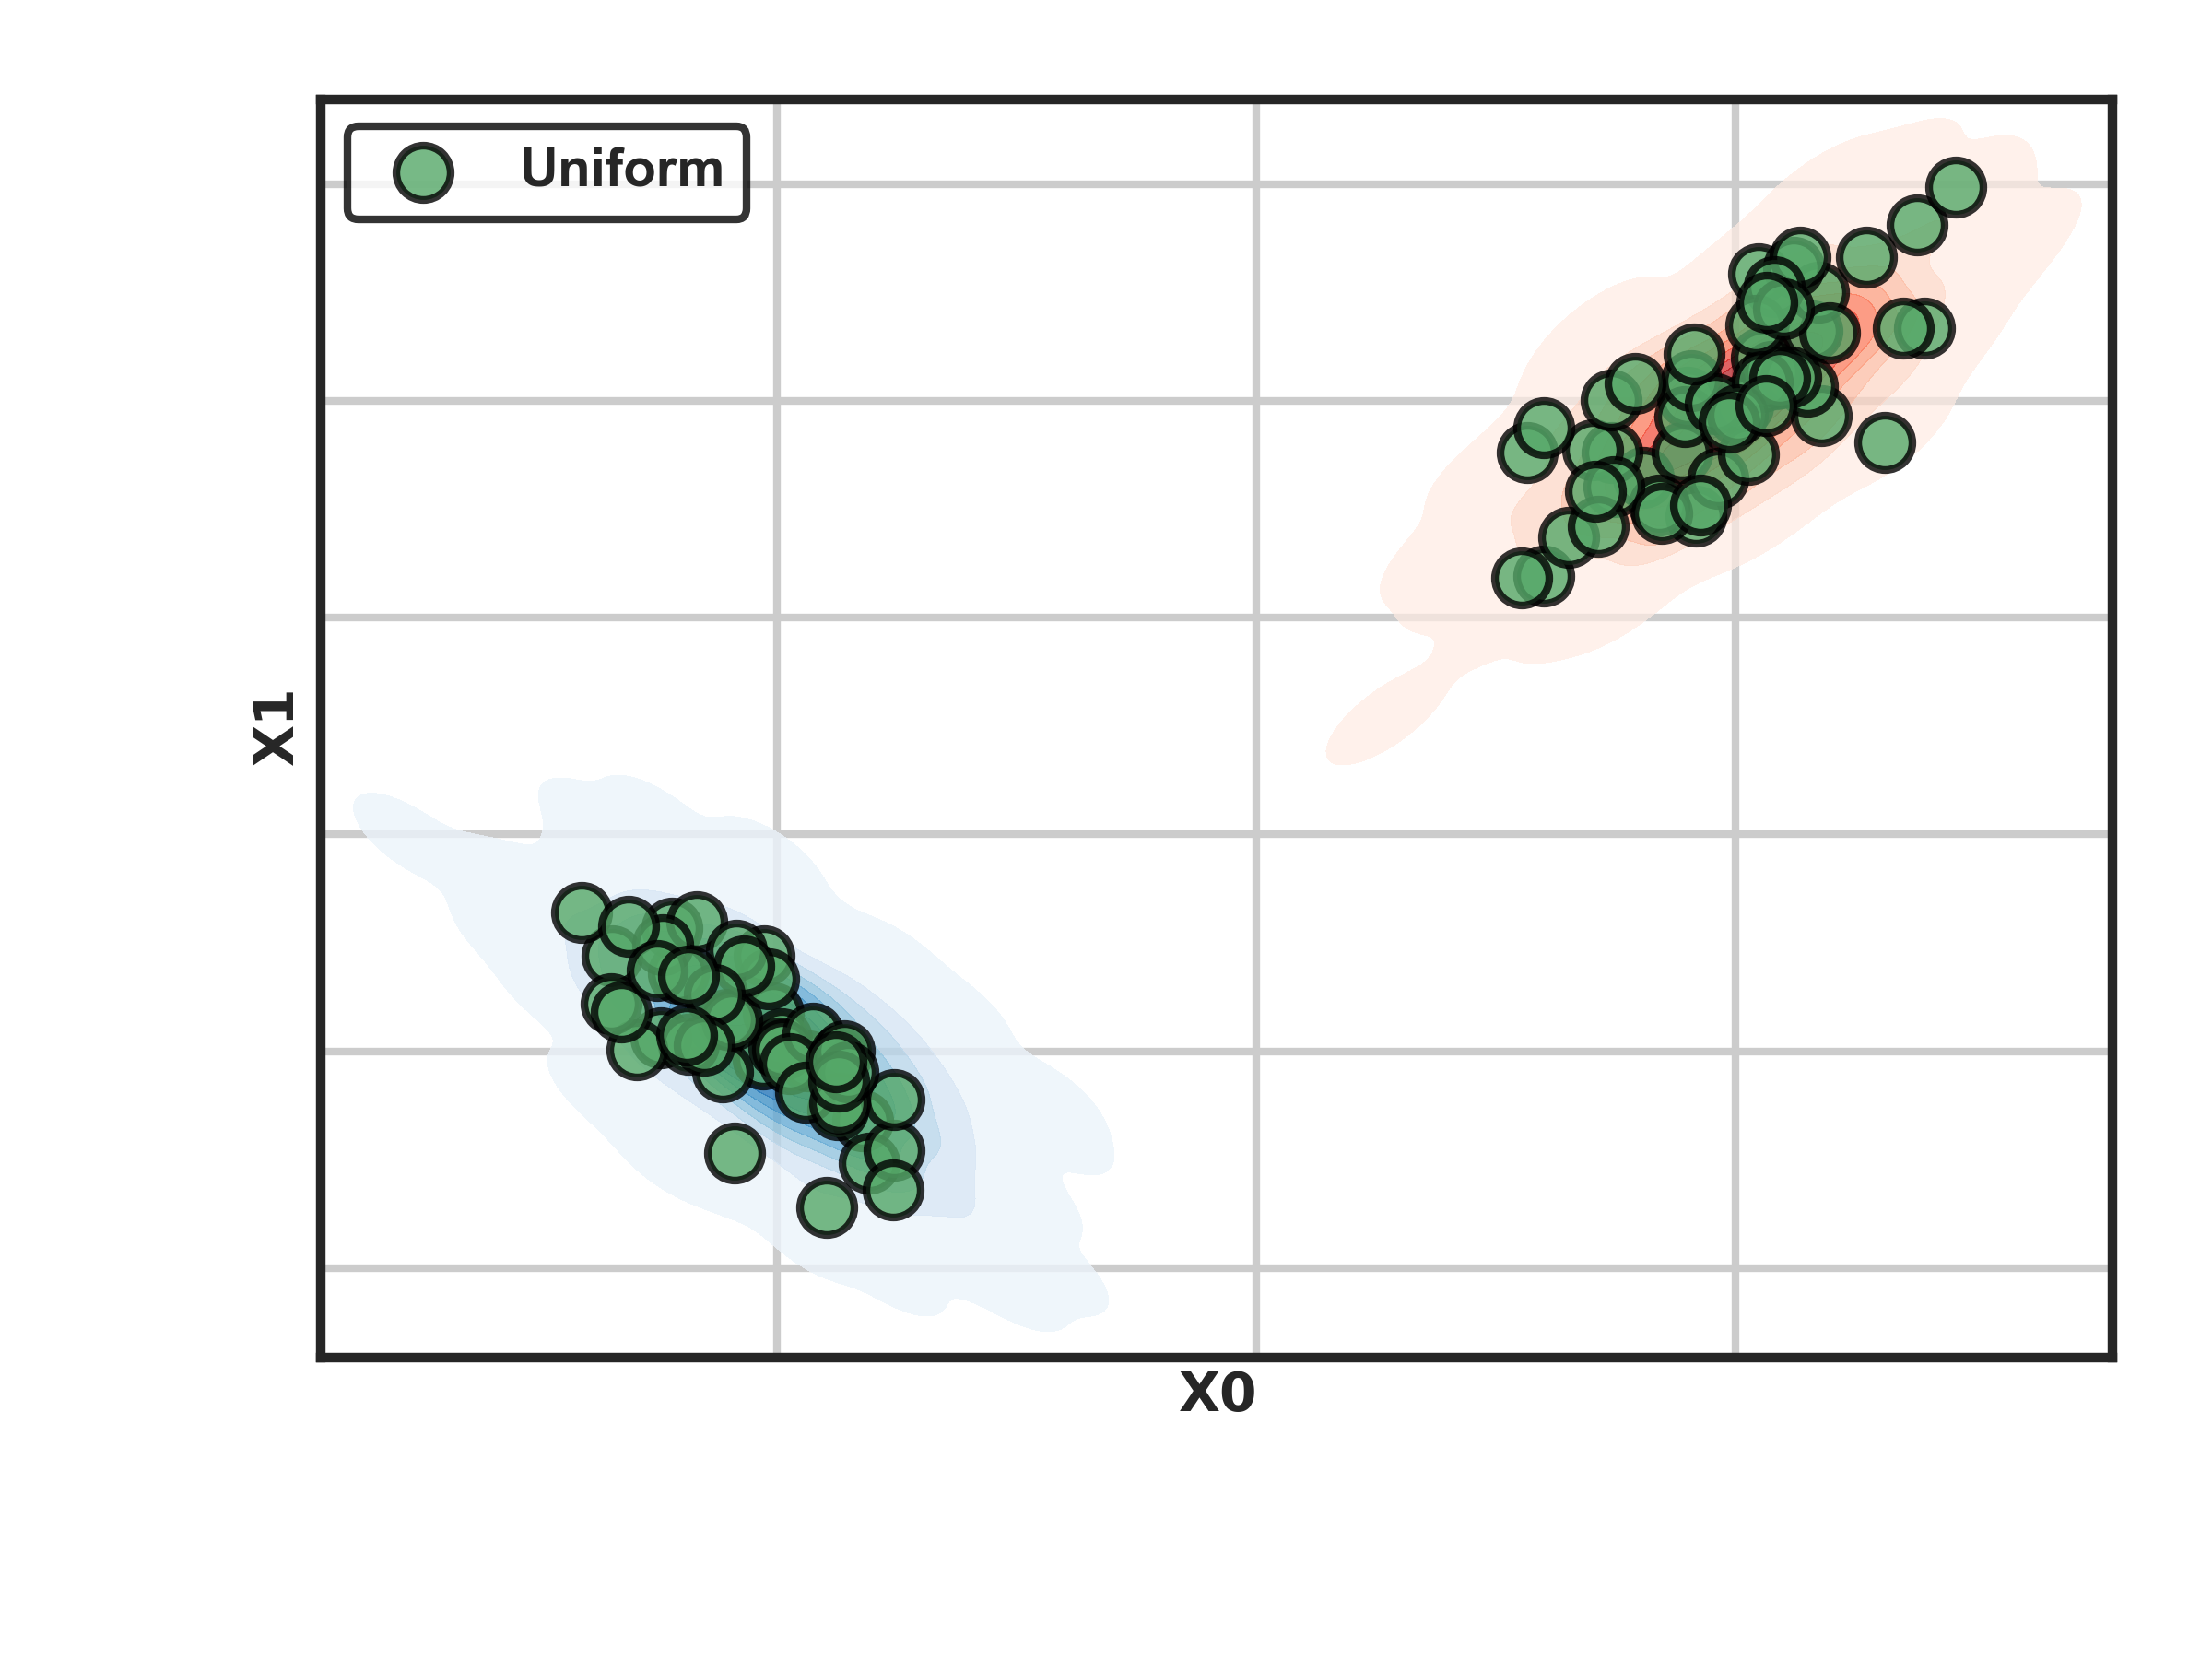}}
\subfloat[Easy]
{\includegraphics[width=0.3\textwidth]{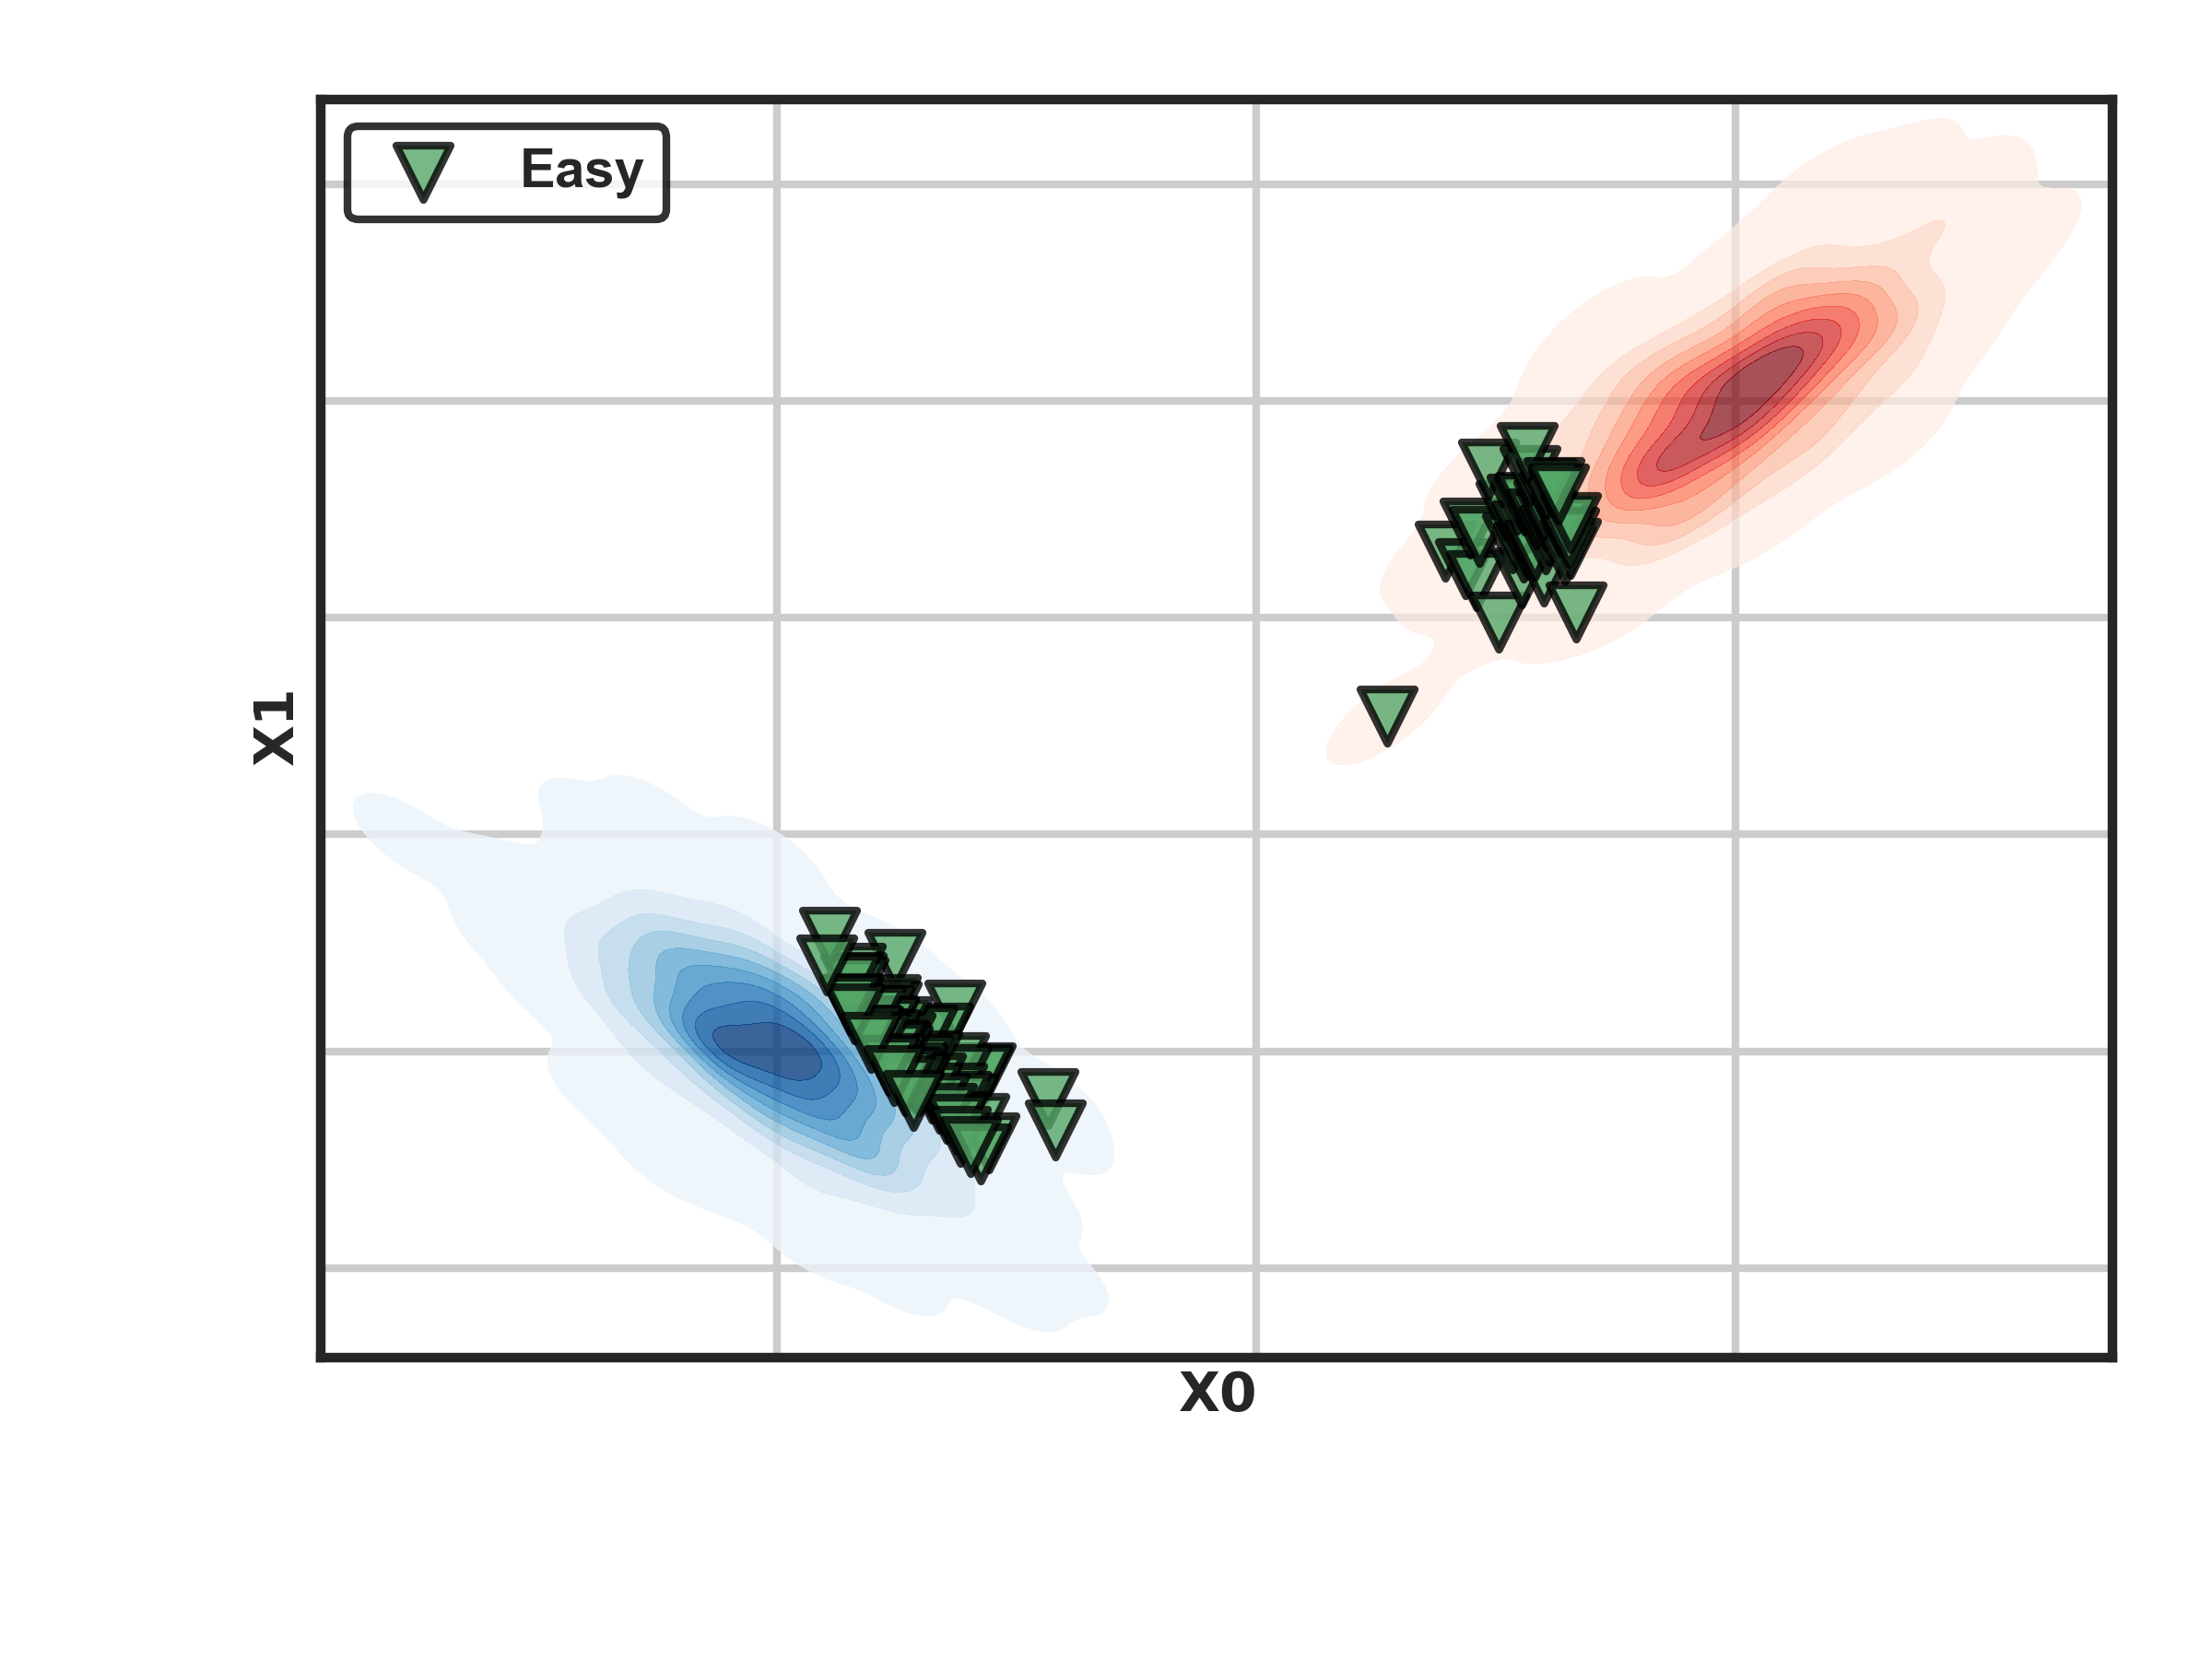}}
\subfloat[Hard]
{\includegraphics[width=0.3\textwidth]{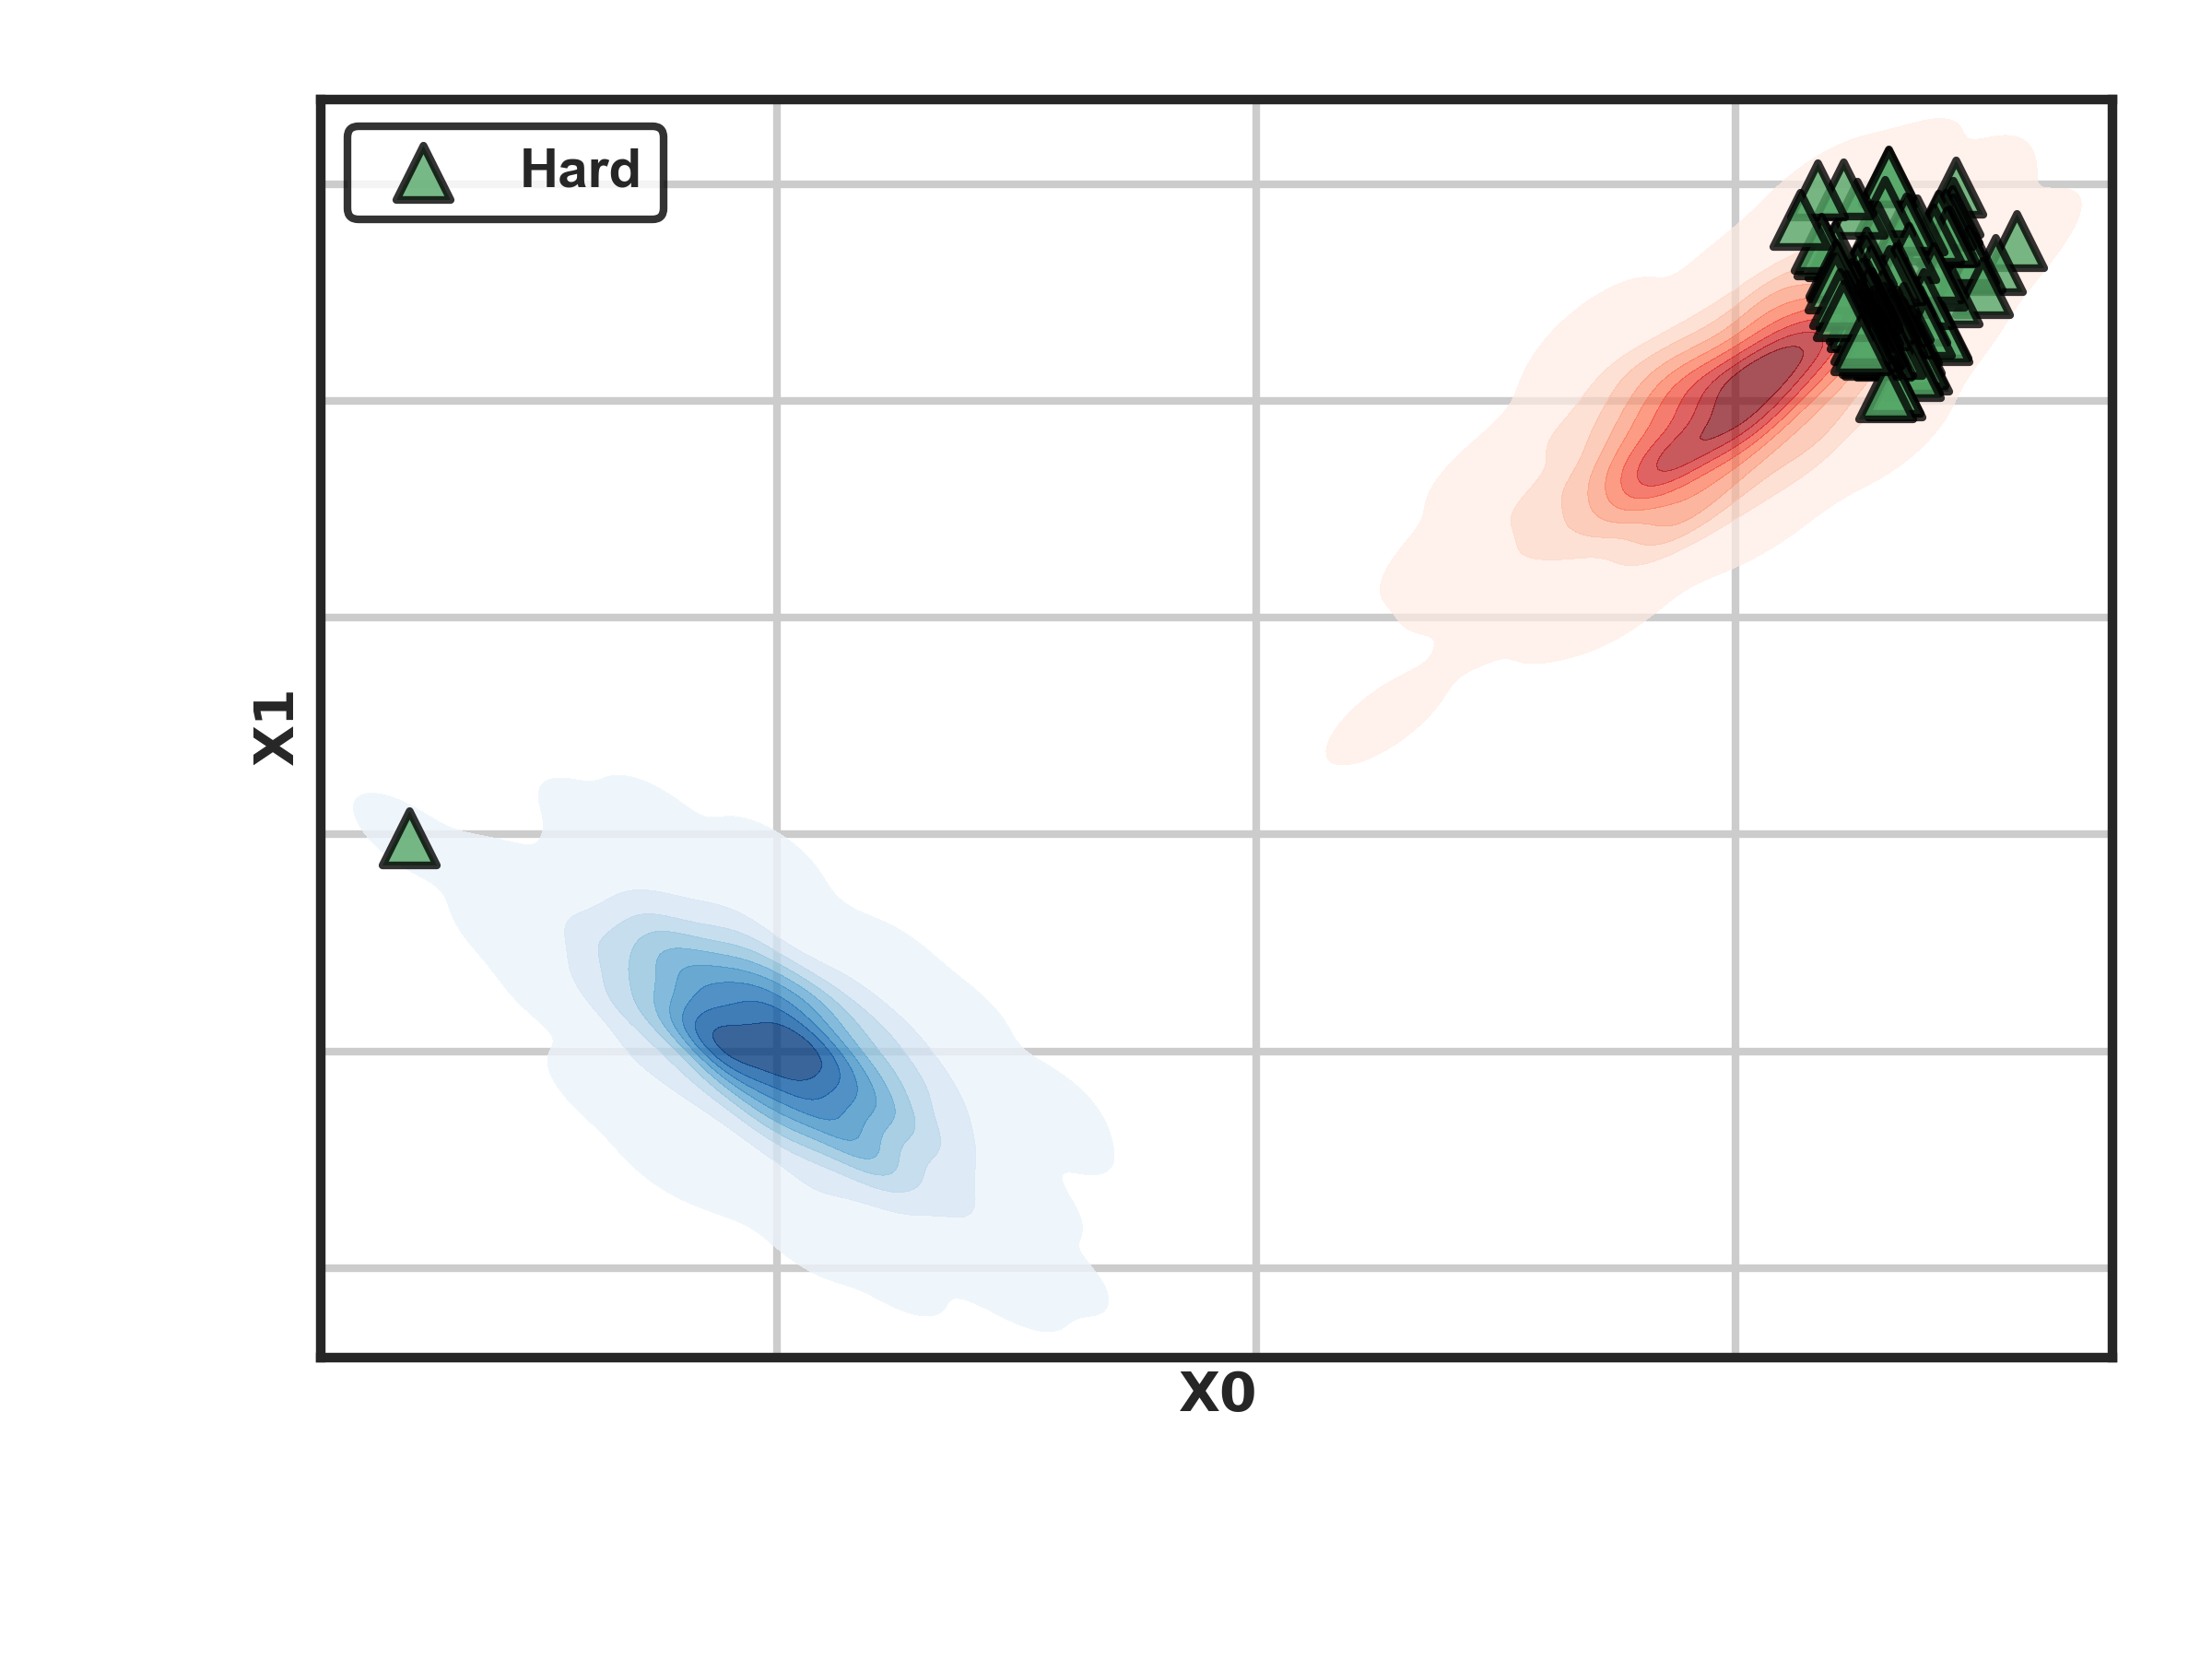}}
\\
\subfloat[Moderate]
{\includegraphics[width=0.3\textwidth]{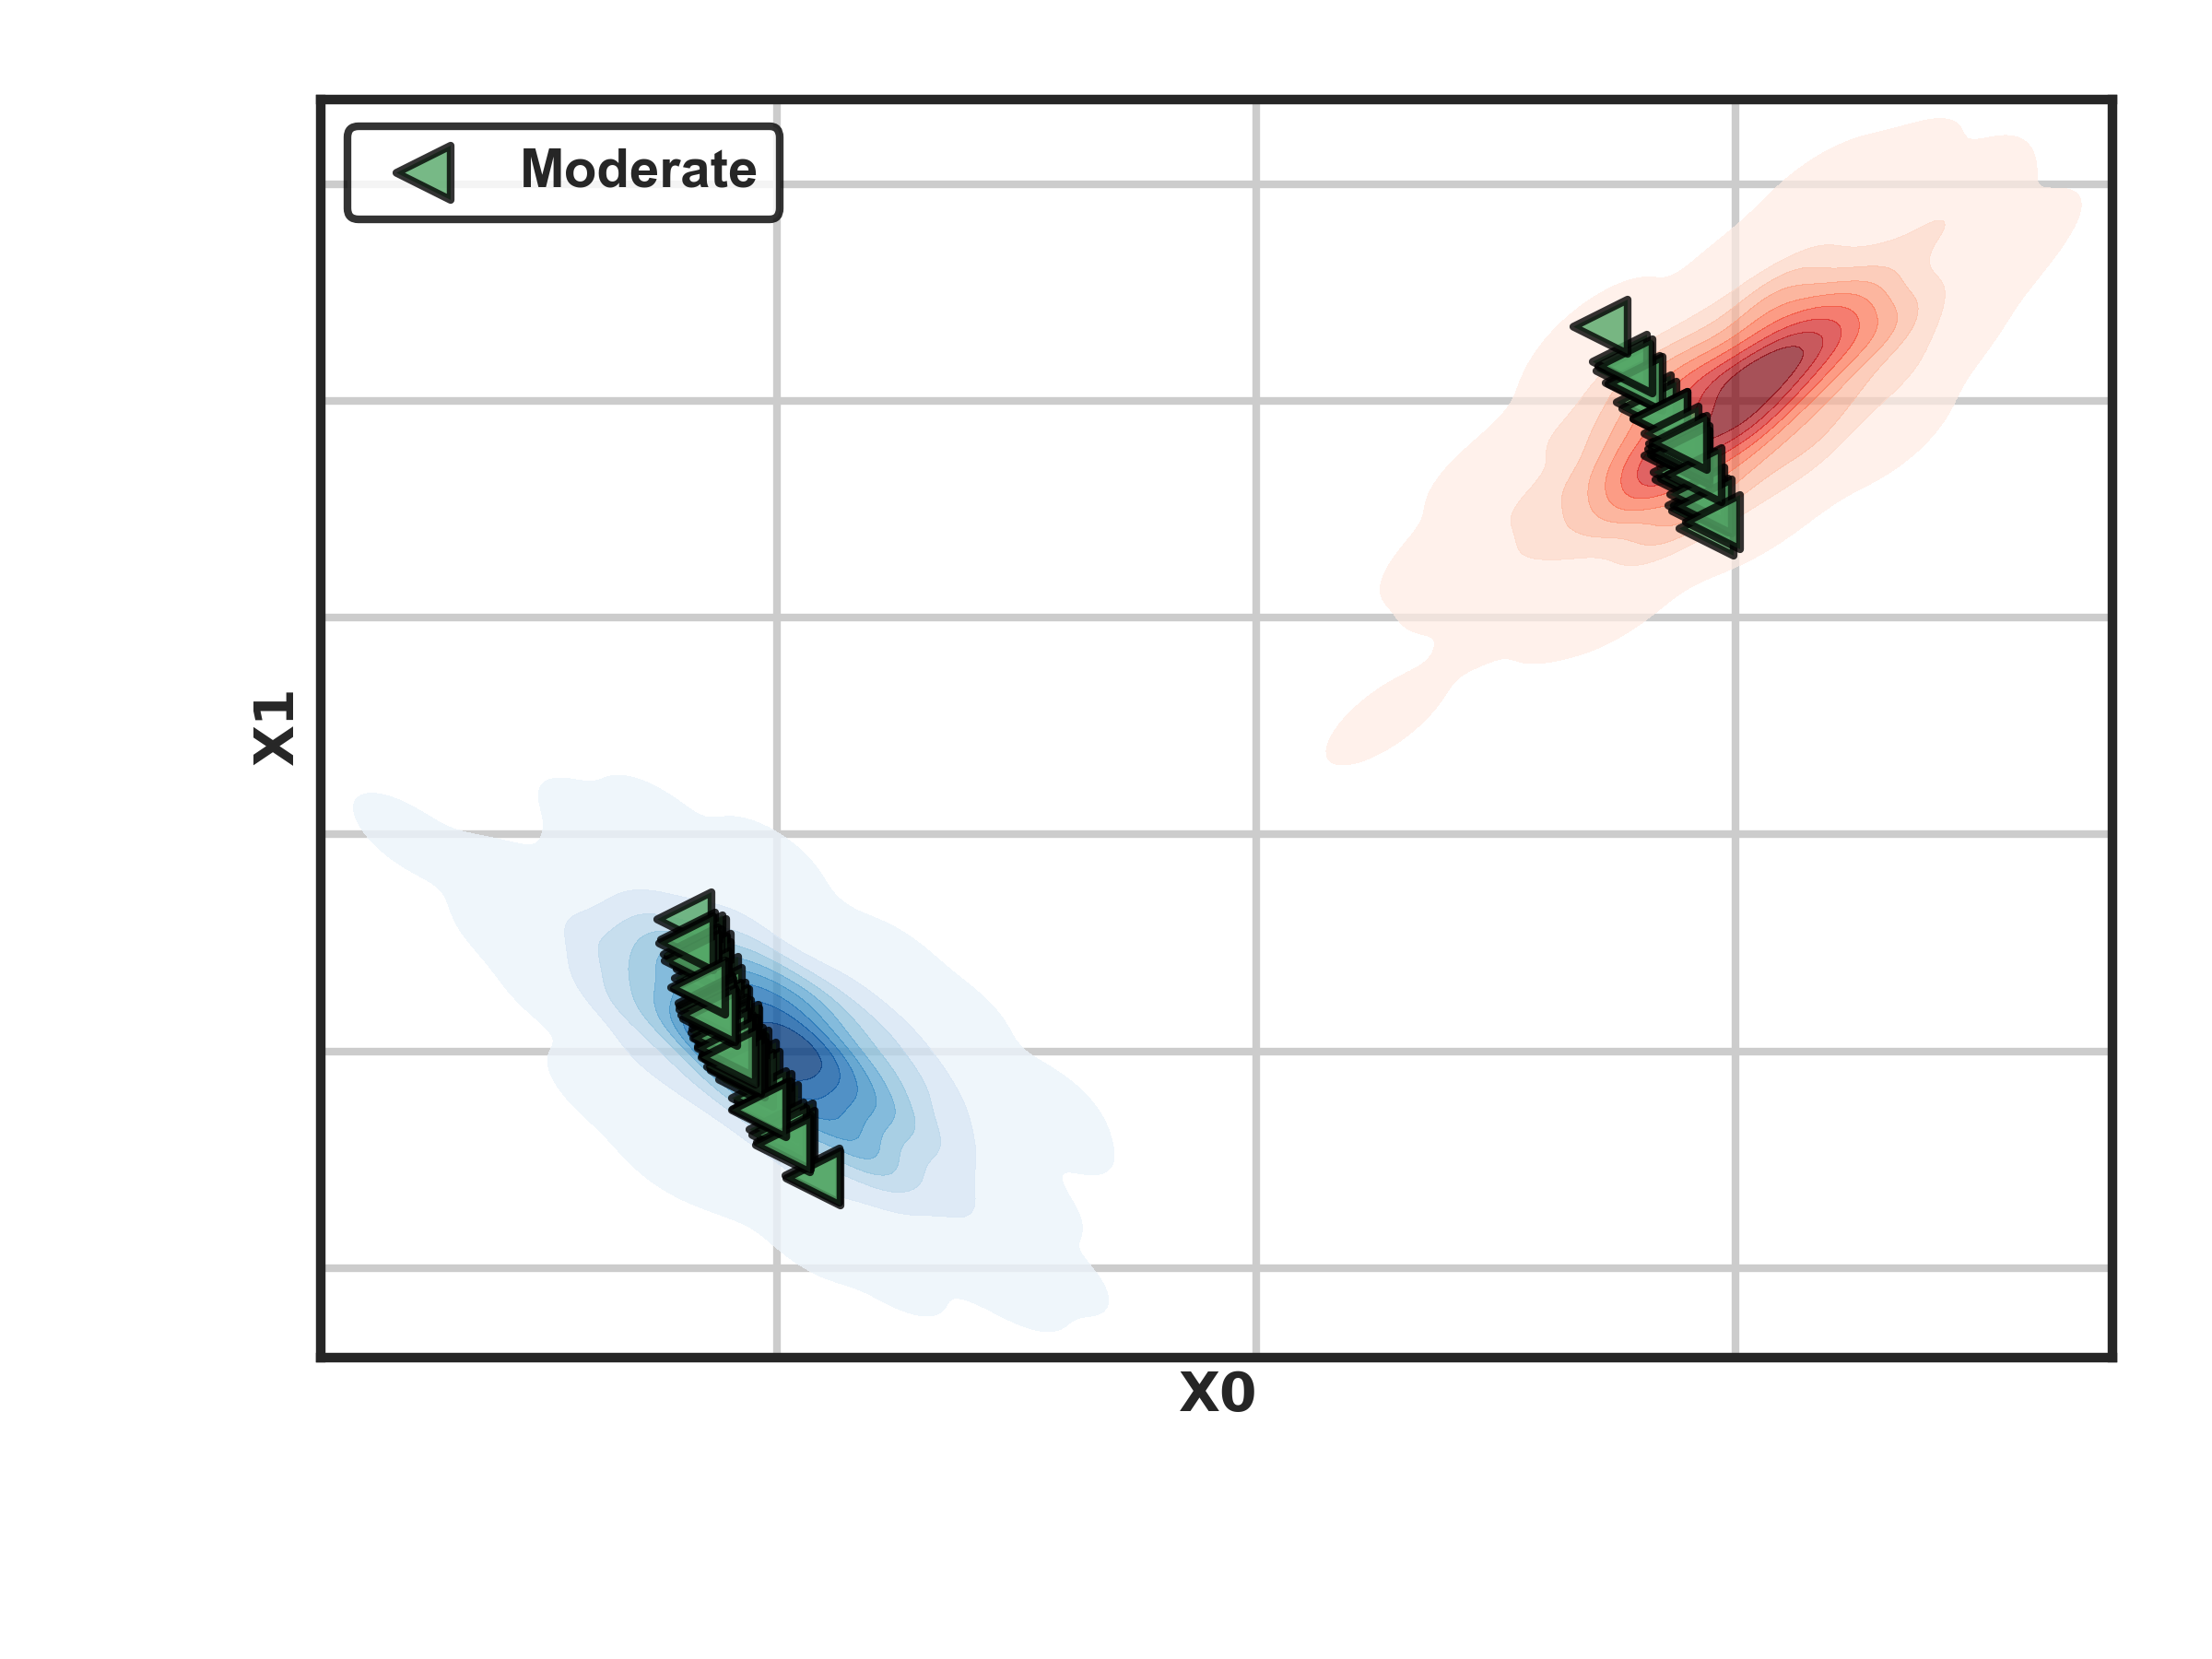}}
\subfloat[Herding]
{\includegraphics[width=0.3\textwidth]{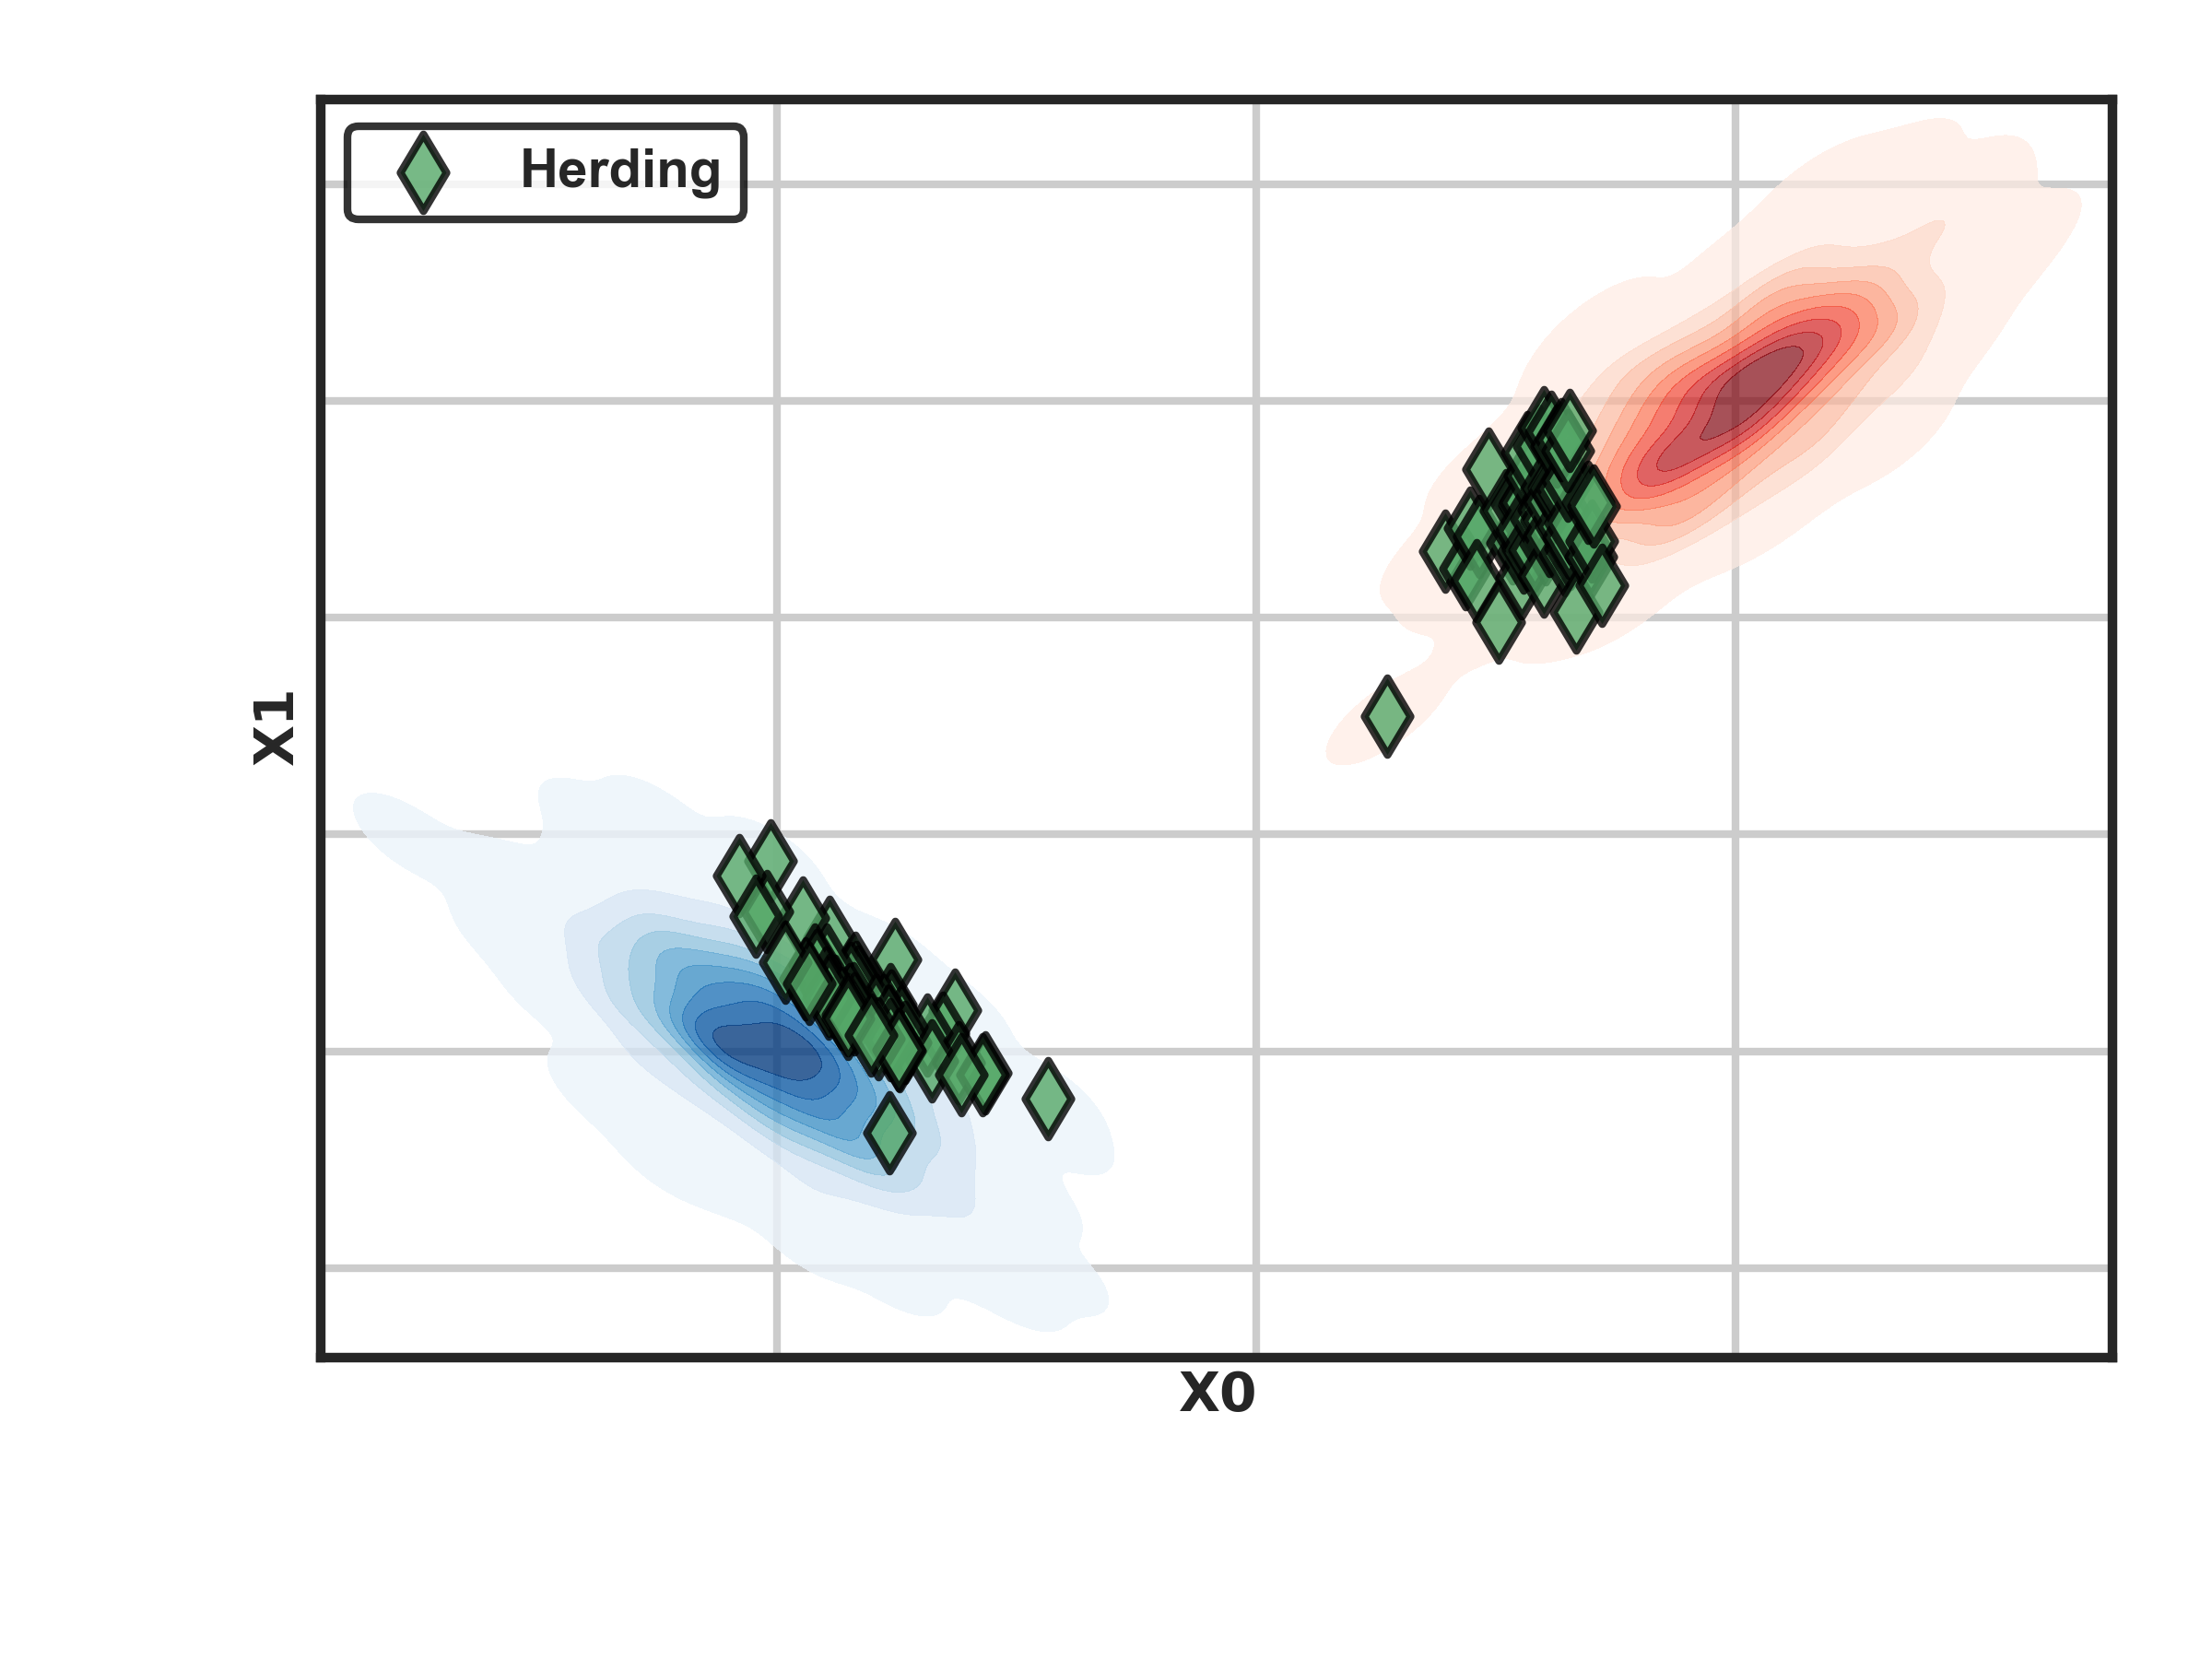}}
\subfloat[$\gmm$]
{\includegraphics[width=0.3\textwidth]{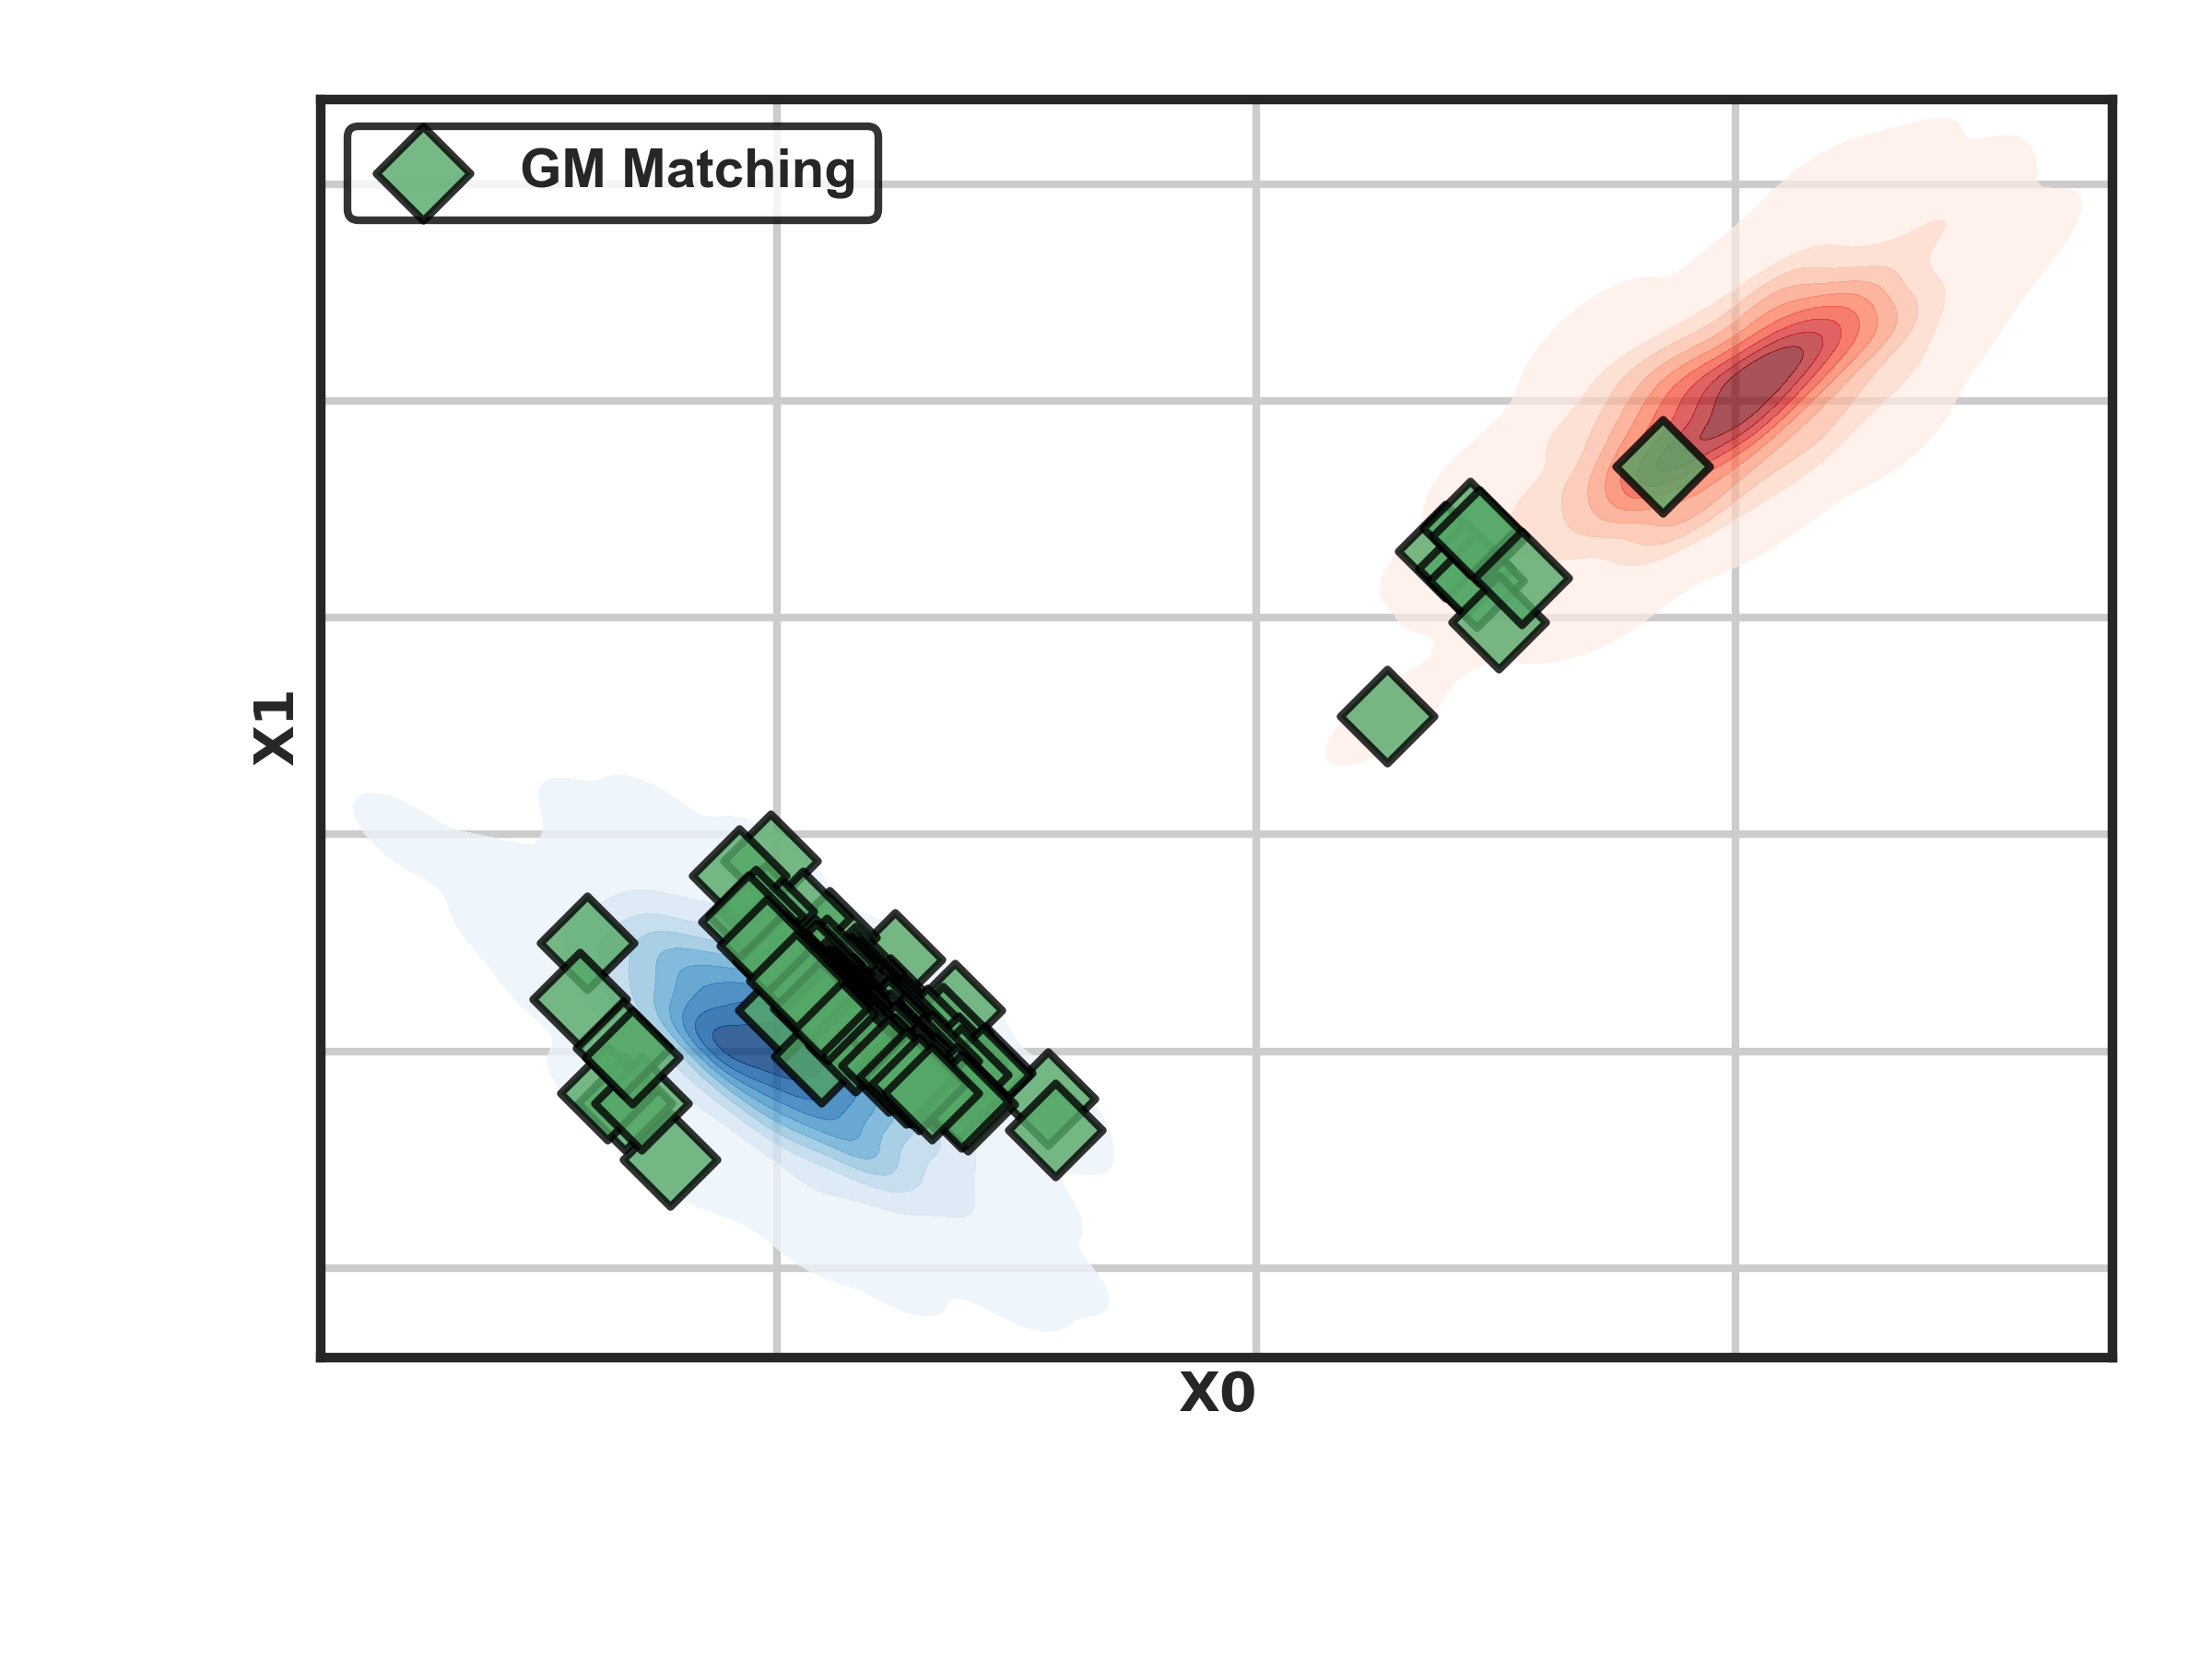}}
\caption{\footnotesize {\bf \textsc{(Sampling from Noisy Gaussian)45\% Corruption ($\psi=0.45$)}} i.e. drawn from an adversary chosen distribution (red). We compare several baselines for choosing 10\% samples: Uniform, Easy, Hard, Moderate, Kernel Herding, \textsc{GM Matching} (\cref{sec:exp-baselines}). $\gmm$ and Kernel Herding are performed using an identity kernel map $\phi(\vx) = \vx$. Clearly $\gmm$ is significantly more robust and diverse than the other approaches even at such high corruption rates.}

\label{fig:exp-syn-corr=45}
\end{figure*}

\clearpage
\section{Additional Details on Baselines}
\label{sec:app-baseline}
Here, we detail the technical aspects of the baselines used in our experiments:
\begin{itemize}
    \item \textbf{Random}: This approach involves randomly selecting a subset of the full dataset.
    \item \textbf{Herding} \cite{welling2009herding}: This method selects data points that are closest to the class centers.
    \item \textbf{Forgetting} \cite{toneva2018empirical}: Data points that are easily forgotten during optimization are chosen.
    \item \textbf{GraNd-score} \cite{paul2021deep}: Data points with larger loss gradient norms are included.
    \item \textbf{EL2N-score} \cite{paul2021deep}: This focuses on data points with larger norms of the error vector, which is the difference between the predicted class probabilities and the one-hot label encoding.
    \item \textbf{Optimization-based} \cite{yang2022dataset}: This method uses the influence function \cite{koh2017understanding} to select data points that minimize the generalization gap under strict constraints.
    \item \textbf{Self-sup.-selection} \cite{sorscher2022beyond}: After self-supervised pre-training and clustering, data points are selected based on their distance to the nearest cluster centroid, with the number of clusters set to the number of classes to avoid tuning. Points with larger distances are chosen.
\end{itemize}

\clearpage
\section{Implementation Details}
\label{sec:app-impl}

\subsection{Image Classification Setup}
For the CIFAR-10/100 experiments, we utilize a batch size of 128 and employ SGD optimizer with a momentum of 0.9, weight decay of 5e-4, and an initial learning rate of 0.1. The learning rate is reduced by a factor of 5 after the 60th, 120th, and 160th epochs, with a total of 200 epochs. Data augmentation techniques include random cropping and random horizontal flipping. 

In the Tiny-ImageNet experiments, a batch size of 256 is used with an SGD optimizer, momentum of 0.9, weight decay of 1e-4, and an initial learning rate of 0.1. The learning rate is decreased by a factor of 10 after the 30th and 60th epochs, with a total of 90 epochs. Random horizontal flips are applied for data augmentation. Each experiment is repeated over 5 random seeds and the variances are noted. Throughout this paper, we use Weiszfield Solver~\citep{weiszfeld1937point} to compute $\gm$ approximately.

\subsection{Diffusion Experiment Setup}
\label{sec:diffusion-setup}

Our diffusion model experiments are conducted on the MNIST dataset. We employ a standard Denoising Diffusion Probabilistic Model (DDPM) \citep{ho2020denoising}, which learns to generate images through a gradual denoising process. The diffusion process is defined as follows:

\begin{equation}
q(x_t | x_{t-1}) = \mathcal{N}(x_t; \sqrt{1 - \beta_t} x_{t-1}, \beta_t I)
\end{equation}

where $x_t$ represents the image at timestep $t$, and $\beta_t$ is the noise variance schedule. The generative model learns to reverse this process using a parameterized function $p_{\theta}(x_{t-1} | x_t)$.

{\bf FID Calculation}

To evaluate the quality of the generated samples, we use the Fréchet Inception Distance (FID), which measures the Wasserstein-2 distance between the feature distributions of real and generated images:

\begin{equation}
\text{FID} = \| \mu_r - \mu_g \|^2 + \text{Tr}(\Sigma_r + \Sigma_g - 2 (\Sigma_r \Sigma_g)^{1/2})
\end{equation}

where $(\mu_r, \Sigma_r)$ and $(\mu_g, \Sigma_g)$ are the mean and covariance of the real and generated feature distributions, respectively.

We use the following hyper-parameters in our diffusion experiments:
\begin{itemize}
    \item \textbf{Batch Size:} 128
    \item \textbf{Learning Rate:} 1e-4
    \item \textbf{Optimizer:} AdamW
    \item \textbf{Number of Diffusion Timesteps:} 1000
    \item \textbf{Beta Scheduler:} Linear
\end{itemize}

Our experiments involve running the model across multiple random seeds to ensure statistical robustness. Results are compared using FID scores to determine the effectiveness of different data selection strategies in training the diffusion model.

\clearpage
\section{Additional Benchmark Experiments (Image Classification)}
\label{sec:app-class}
We share additional results on benchmark datasets that were omitted from the main paper due to space constraints.~\cref{tab:cifarC}-\ref{tab:VGG-Shuffle}.

\subsection{Robustness to Corrupt Images}

\input{tables/benchmark/tab-cifarC}
\input{tables/benchmark/tab-tinyC}

\subsection{Robustness to Label Noise}

\begin{table*}
    \footnotesize
    \centering
    \resizebox{0.7\textwidth}{!}
{
    \begin{tabular}{lccccc}
        \toprule
        
        & \multicolumn{2}{c}{\bf CIFAR-100 (Label noise)} 
        & \multicolumn{2}{c}{\bf Tiny ImageNet (Label noise)} 
        & 
        \\
        \cmidrule(r){2-3} 
        \cmidrule(r){4-5} 
        {\bf Method / Ratio }
        & {\bf 20\%} 
        & {\bf 30\%} 
        & {\bf 20\%} 
        & {\bf 30\%} 
        & {\bf Mean $\uparrow$}
        \\
        \midrule
        \multicolumn{6}{c}{\bf 20\% Label Noise}
        \\
        \midrule
        Random 
        & 34.47$\pm$0.64 
        & 43.26$\pm$1.21 
        & 17.78$\pm$0.44 
        & 23.88$\pm$0.42 
        & 29.85
        \\
        Herding 
        & 42.29$\pm$1.75 
        & 50.52$\pm$3.38
        & 18.98$\pm$0.44 
        & 24.23$\pm$0.29 
        &  34.01
        \\
        Forgetting 
        & 36.53$\pm$1.11 
        & 45.78$\pm$1.04 
        & 13.20$\pm$0.38 
        & 21.79$\pm$0.43 
        & 29.33
        \\
        GraNd-score 
        & 31.72$\pm$0.67 
        & 42.80$\pm$0.30 
        & 18.28$\pm$0.32 
        & 23.72$\pm$0.18 
        & 28.05
        \\
        EL2N-score 
        & 29.82$\pm$1.19 
        & 33.62$\pm$2.35 
        & 13.93$\pm$0.69 
        & 18.57$\pm$0.31 
        & 23.99
        \\
        Optimization-based 
        & 32.79$\pm$0.62 
        & 41.80$\pm$1.14
        & 14.77$\pm$0.95 
        & 22.52$\pm$0.77 
        & 27.57
        \\
        Self-sup.-selection 
        & 31.08$\pm$0.78 
        & 41.87$\pm$0.63 
        & 15.10$\pm$0.73 
        & 21.01$\pm$0.36 
        & 27.27
        \\
        Moderate-DS 
        & 40.25$\pm$0.12 
        & 48.53$\pm$1.60 
        & 19.64$\pm$0.40 
        & 24.96$\pm$0.30
        & 31.33
        \\
        {\bf $\gm$ Matching}
        & {\bf 52.64$\pm$0.72}
        & {\bf 61.01$\pm$0.47}
        & {\bf 25.80$\pm$0.37} 
        & {\bf 31.71$\pm$0.24}
        & {\bf 42.79}
        \\
        \midrule
        \multicolumn{6}{c}{\bf 35\% Label Noise}
        \\
        \midrule
        Random 
        & 24.51$\pm$1.34 
        & 32.26$\pm$0.81 
        & 14.64$\pm$0.29 
        & 19.41$\pm$0.45 
        & 22.71
        \\
        Herding 
        & 29.42$\pm$1.54 
        & 37.50$\pm$2.12 
        & 15.14$\pm$0.45 
        & 20.19$\pm$0.45 
        & 25.56
        \\
        Forgetting 
        & 29.48$\pm$1.98 
        & 38.01$\pm$2.21 
        & 11.25$\pm$0.90 
        & 17.07$\pm$0.66 
        & 23.14
        \\
        GraNd-score 
        & 23.03$\pm$1.05 
        & 34.83$\pm$2.01 
        & 13.68$\pm$0.46 
        & 19.51$\pm$0.45 
        & 22.76
        \\
        EL2N-score 
        & 21.95$\pm$1.08 
        & 31.63$\pm$2.84 
        & 10.11$\pm$0.25 
        & 13.69$\pm$0.32 
        & 19.39
        \\
        Optimization-based 
        & 26.77$\pm$0.15 
        & 35.63$\pm$0.92 
        & 12.37$\pm$0.68 
        & 18.52$\pm$0.90 
        & 23.32
        \\
        Self-sup.-selection 
        & 23.12$\pm$1.47 
        & 34.85$\pm$0.68 
        & 11.23$\pm$0.32 
        & 17.76$\pm$0.69 
        & 22.64
        \\
        Moderate-DS 
        & 28.45$\pm$0.53 
        & 36.55$\pm$1.26 
        & 15.27$\pm$0.31 
        & 20.33$\pm$0.28 
        & 25.15
        \\
        {\bf $\gm$ Matching}
        & {\bf 43.33$\pm$ 1.02}
        & {\bf 58.41$\pm$ 0.68}
        & {\bf 23.14$\pm$ 0.92} 
        & {\bf 27.76$\pm$ 0.40}
        & {\bf 38.16}
        \\
        \bottomrule
    \end{tabular}
}
    \caption{
    \footnotesize
    {\bf \textsc{(Label Noise) Image Classification:}} Comparing (Test Accuracy) pruning methods on CIFAR-100 and TinyImageNet datasets, under 20\% and 35\% Symmetric Label Corruption, at 20\% and 30\% selection ratio. ResNet-50 is used both as proxy and for downstream classification.
    }
    \label{tab:main-N}
\end{table*}
\begin{table*}[t]
    \footnotesize
    \centering
    \resizebox{0.7\textwidth}{!}
{
    \begin{tabular}{lccccc}
        \toprule
        & \multicolumn{2}{c}{\bf CIFAR-100 (PGD Attack)} 
        & \multicolumn{2}{c}{\bf CIFAR-100 (GS Attack)} 
        & \\
        \cmidrule(r){2-3} 
        \cmidrule(r){4-5} 
        {\bf Method / Ratio } 
        & 20\% 
        & 30\% 
        & 20\% 
        & 30\% 
        & {\bf Mean $\uparrow$} 
        \\
        \midrule
        Random 
        & 43.23$\pm$0.31 
        & 52.86$\pm$0.34 
        & 44.23$\pm$0.41 
        & 53.44$\pm$0.44 
        & 48.44
        \\
        Herding 
        & 40.21$\pm$0.72 
        & 49.62$\pm$0.65 
        & 39.92$\pm$1.03 
        & 50.14$\pm$0.15 
        & 44.97
        \\
        Forgetting 
        & 35.90$\pm$1.30 
        & 47.37$\pm$0.99 
        & 37.55$\pm$0.53 
        & 46.88$\pm$1.91 
        & 41.93
        \\
        GraNd-score 
        & 40.87$\pm$0.84 
        & 50.13$\pm$0.30 
        & 40.77$\pm$1.11 
        & 49.88$\pm$0.83 
        & 45.41
        \\
        EL2N-score 
        & 26.61$\pm$0.58 
        & 34.50$\pm$1.02 
        & 26.72$\pm$0.66 
        & 35.55$\pm$1.30 
        & 30.85
        \\
        Optimization-based 
        & 38.29$\pm$1.77 
        & 46.25$\pm$1.82 
        & 41.36$\pm$0.92 
        & 49.10$\pm$0.81 
        & 43.75
        \\
        Self-sup.-selection 
        & 40.53$\pm$1.15 
        & 49.95$\pm$0.50 
        & 40.74$\pm$1.66 
        & 51.23$\pm$0.25 
        & 45.61
        \\
        Moderate-DS 
        & 43.60$\pm$0.97 
        & 51.66$\pm$0.39 
        & 44.69$\pm$0.68 
        & 53.71$\pm$0.37 
        & 48.42
        \\
        {\bf $\gm$ Matching}
        & {\bf 45.41 $\pm$0.86}
        & {\bf 51.80 $\pm$1.01}
        & {\bf 49.78 $\pm$0.27}
        & {\bf 55.50 $\pm$0.31}
        & {\bf 50.62}
        \\
        \toprule
        & \multicolumn{2}{c}{\bf Tiny ImageNet (PGD Attack)} 
        & \multicolumn{2}{c}{\bf Tiny ImageNet (GS Attack)} 
        & \\
        \cmidrule(r){2-3} 
        \cmidrule(r){4-5} 
        {\bf Method / Ratio } 
        & 20\% 
        & 30\% 
        & 20\% 
        & 30\% 
        & {\bf Mean $\uparrow$} 
        \\
        \midrule
        Random 
        & 20.93$\pm$0.30 
        & 26.60$\pm$0.98 
        & 22.43$\pm$0.31 
        & 26.89$\pm$0.31 
        & 24.21
        \\
        Herding 
        & 21.61$\pm$0.36 
        & 25.95$\pm$0.19 
        & 23.04$\pm$0.28 
        & 27.39$\pm$0.14 
        & 24.50
        \\
        Forgetting 
        & 20.38$\pm$0.47 
        & 26.12$\pm$0.19 
        & 22.06$\pm$0.31 
        & 27.21$\pm$0.21 
        & 23.94
        \\
        GraNd-score 
        & 20.76$\pm$0.21 
        & 26.34$\pm$0.32 
        & 22.56$\pm$0.30 
        & 27.52$\pm$0.40 
        & 24.30
        \\
        EL2N-score 
        & 16.67$\pm$0.62 
        & 22.36$\pm$0.42 
        & 19.93$\pm$0.57 
        & 24.65$\pm$0.32 
        & 20.93
        \\
        Optimization-based 
        & 19.26$\pm$0.77 
        & 24.55$\pm$0.92 
        & 21.26$\pm$0.24 
        & 25.88$\pm$0.37 
        & 22.74
        \\
        Self-sup.-selection 
        & 19.23$\pm$0.46 
        & 23.92$\pm$0.51 
        & 19.70$\pm$0.20 
        & 24.73$\pm$0.39 
        & 21.90
        \\
        Moderate-DS 
        & 21.81$\pm$0.37 
        & 27.11$\pm$0.20 
        & 23.20$\pm$0.13 
        & 28.89$\pm$0.27 
        & 25.25
        \\
        {\bf $\gm$ Matching}
        & {\bf 25.98 $\pm$1.12}
        & {\bf 30.77 $\pm$0.25}
        & {\bf 29.71 $\pm$0.45}
        & {\bf 32.88 $\pm$0.73}
        & {\bf 29.84}
        \\
        \bottomrule
    \end{tabular}
    }
    \caption{
    \footnotesize
    {\bf \textsc{(Adversarial Attack) Image Classification:}} . Comparing (Test Accuracy) pruning methods under PGD and GS attacks. ResNet-50 is used both as proxy and for downstream classification.
    }
    \label{tab:main-A}
\end{table*}

\input{tables/benchmark/tab-noisy}
\begin{table*}
    \footnotesize
    \centering
    \begin{tabular}{lccccc}
        \toprule
        
        & \multicolumn{2}{c}{\bf CIFAR-100 (Label noise)} 
        & \multicolumn{2}{c}{\bf Tiny ImageNet (Label noise)} 
        & \\
        \cmidrule(r){2-3} 
        \cmidrule(r){4-5} 
        {\bf Method / Ratio } 
        & 20\% 
        & 30\% 
        & 20\% 
        & 30\% 
        \\
        \midrule
        Random 
        & 24.51$\pm$1.34 
        & 32.26$\pm$0.81 
        & 14.64$\pm$0.29 
        & 19.41$\pm$0.45 

        \\
        Herding 
        & 29.42$\pm$1.54 
        & 37.50$\pm$2.12 
        & 15.14$\pm$0.45 
        & 20.19$\pm$0.45 

        \\
        Forgetting 
        & 29.48$\pm$1.98 
        & 38.01$\pm$2.21 
        & 11.25$\pm$0.90 
        & 17.07$\pm$0.66 

        \\
        GraNd-score 
        & 23.03$\pm$1.05 
        & 34.83$\pm$2.01 
        & 13.68$\pm$0.46 
        & 19.51$\pm$0.45 
        & 
        \\
        EL2N-score 
        & 21.95$\pm$1.08 
        & 31.63$\pm$2.84 
        & 10.11$\pm$0.25 
        & 13.69$\pm$0.32 
        & 
        \\
        Optimization-based 
        & 26.77$\pm$0.15 
        & 35.63$\pm$0.92 
        & 12.37$\pm$0.68 
        & 18.52$\pm$0.90 
        & 
        \\
        Self-sup.-selection 
        & 23.12$\pm$1.47 
        & 34.85$\pm$0.68 
        & 11.23$\pm$0.32 
        & 17.76$\pm$0.69 
        &
        \\
        Moderate-DS 
        & 28.45$\pm$0.53 
        & 36.55$\pm$1.26 
        & 15.27$\pm$0.31 
        & 20.33$\pm$0.28 
        & 
        \\
        {\bf $\gm$ Matching}
        & {\bf 43.33$\pm$ 1.02}
        & {\bf 58.41$\pm$ 0.68}
        & {\bf 23.14$\pm$ 0.92} 
        & {\bf 27.76$\pm$ 0.40}
        & 
        \\
        \bottomrule
    \end{tabular}
    \caption{35\% Label Noise}
    \label{tab:label-noise-0.35}
\end{table*}

\input{tables/benchmark/tab-noisy-tiny}

\subsection{Robustness to Adversarial Attack}
\input{tables/benchmark/tab-attacks}

\clearpage
\section{Ablations with Proxy Model}
\label{sec:app-prox}
We perform experiments across multiple choices of proxy encoder scenarios: {\bf (A) Standard Setting: } when the proxy model shares the same architecture as the model~\cref{tab:main-clean}-~\ref{tab:main-A}). Additionally, we also experiment with {\bf (B) Distribution Shift: } proxy model pretrained on a different (distribution shifted) dataset(~\cref{fig:main-cifar-vanilla}-\ref{fig:main-cifar-lp}) e.g. ImageNet and used to sample from CIFAR10. {\bf (C) Network Transfer: } where, the proxy has a different network compared to the downstream classifier (\cref{tab:main-nw-T}).

\input{tables/benchmark/tab-vgg-shuffle}
\input{tables/benchmark/tab-main-nw-transfer}
\begin{figure}[htbp]
    \centering
    % First row of subfigures
    \begin{subfigure}[b]{0.3\textwidth}
        \centering
        \includegraphics[width=\textwidth]{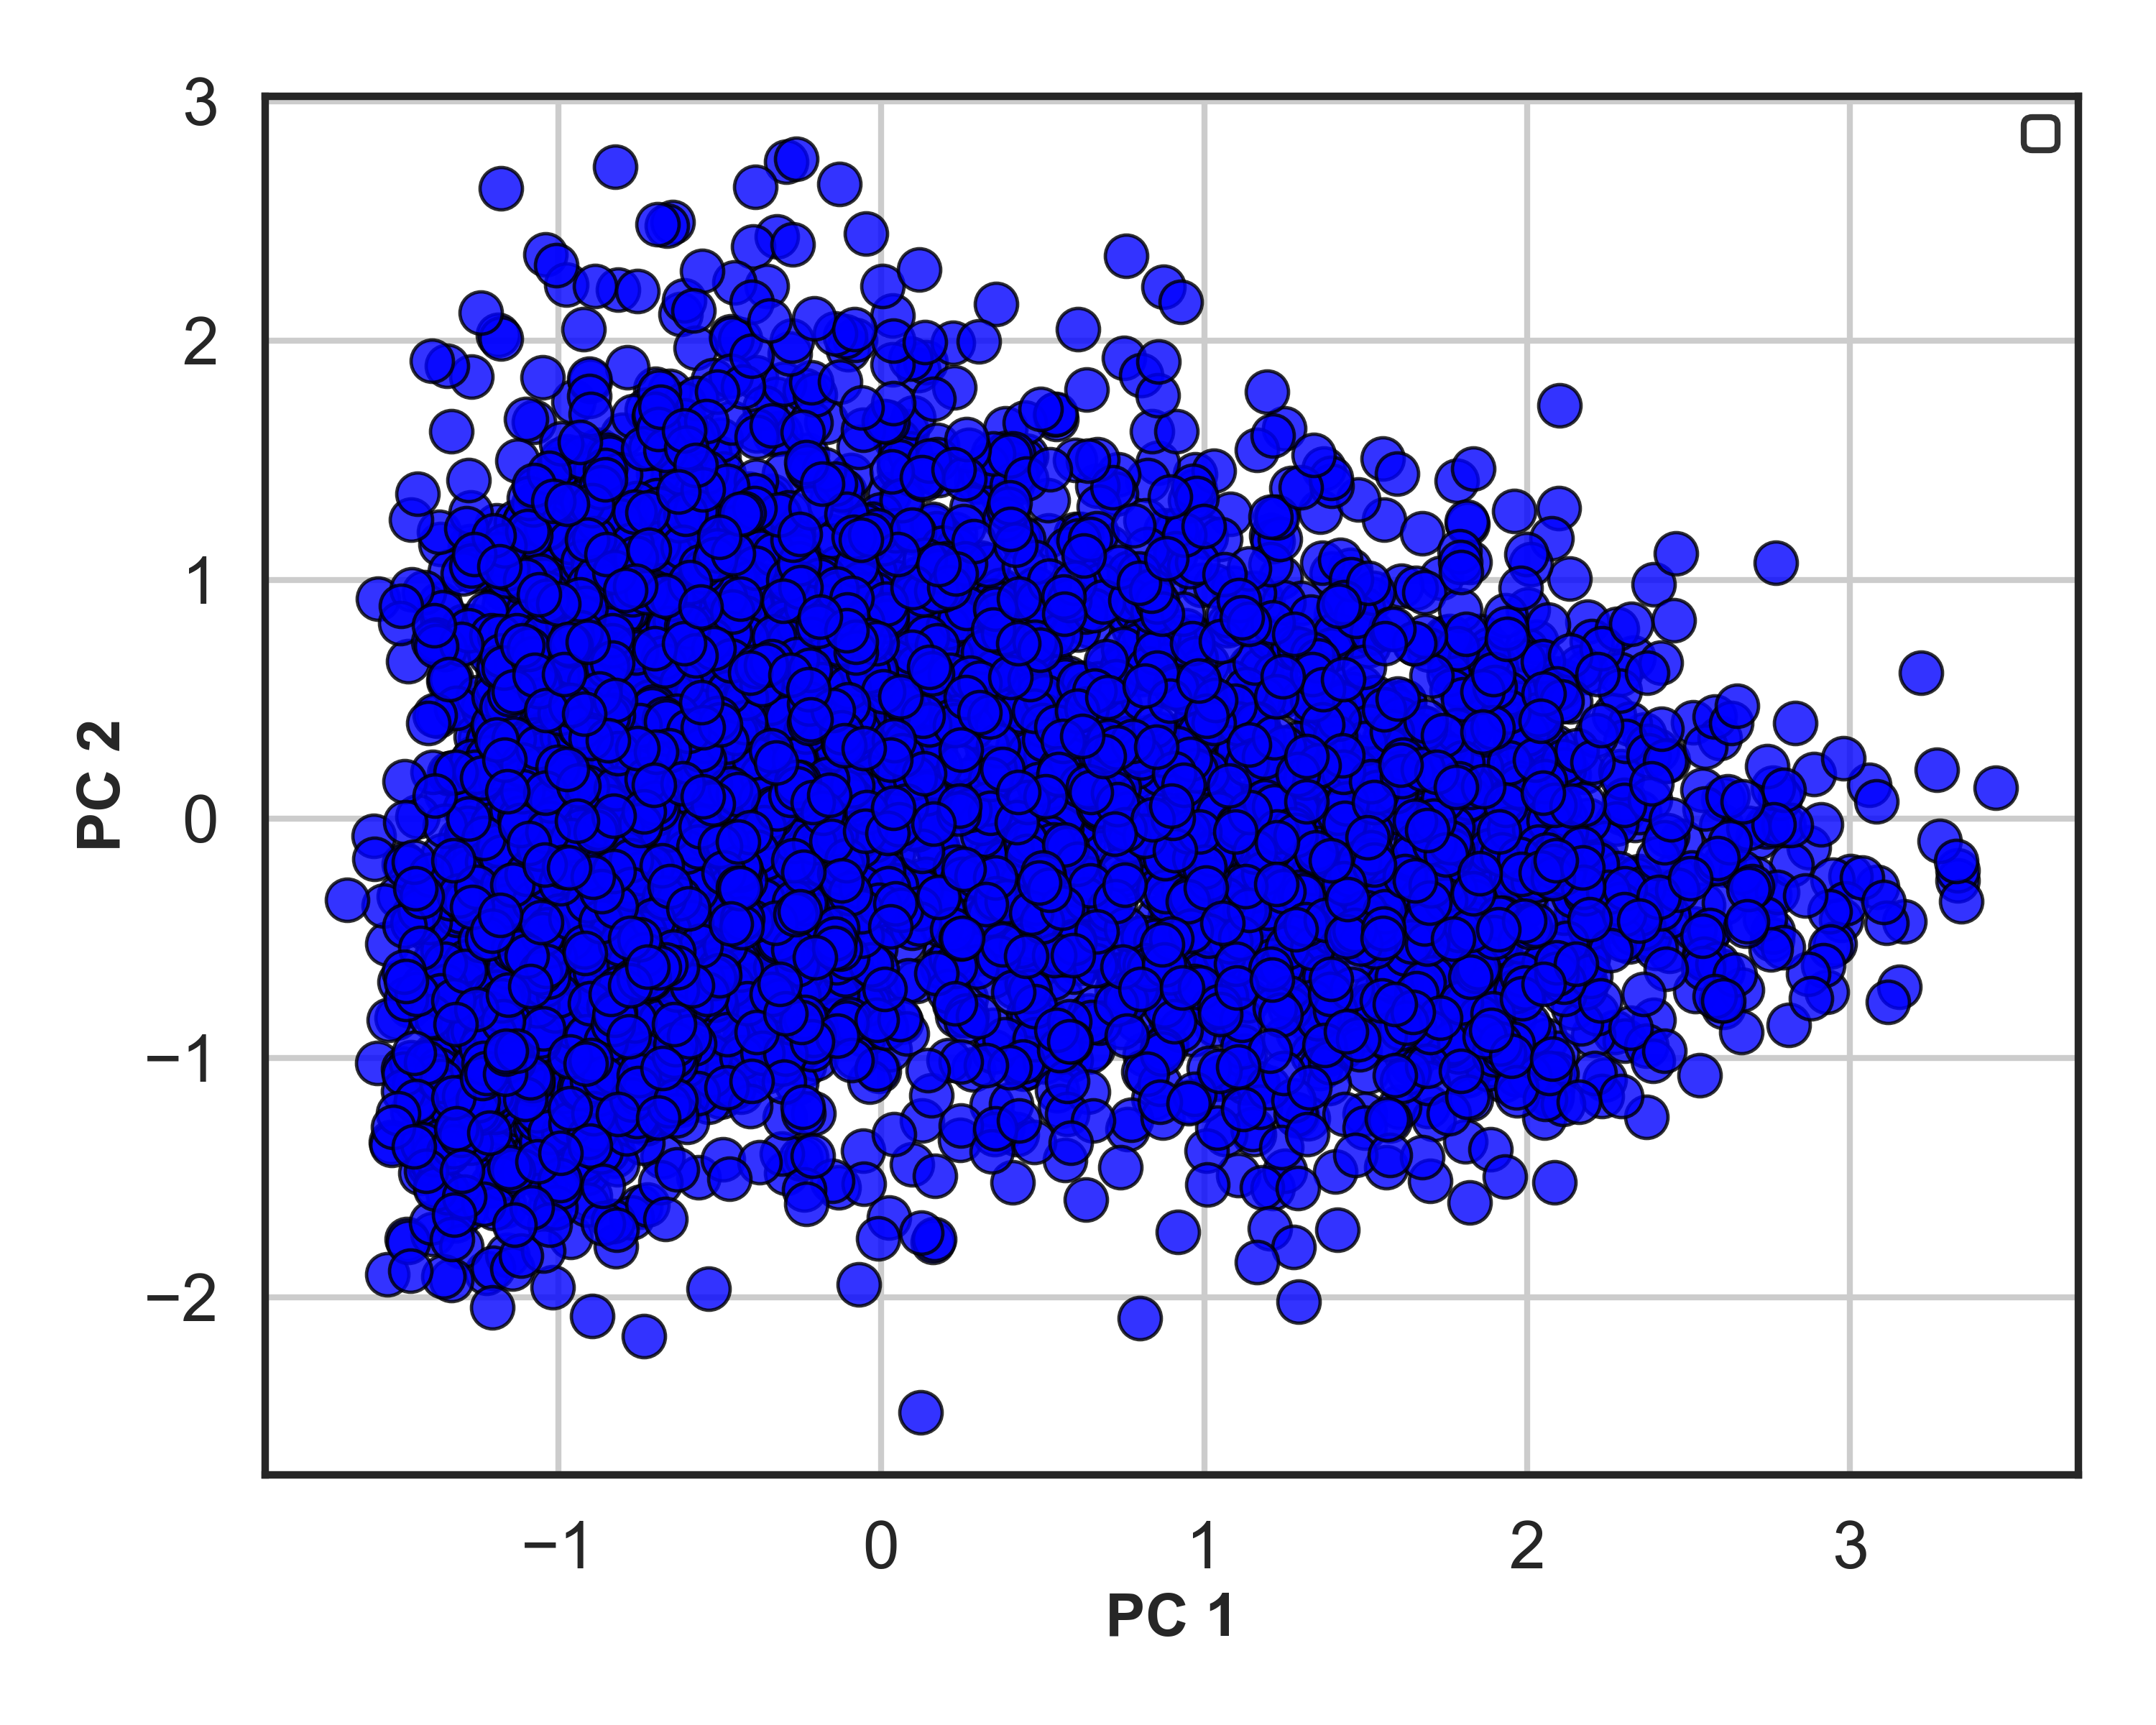}
        \caption{Clean Samples}
    \end{subfigure}    
    \hfill
    \begin{subfigure}[b]{0.3\textwidth}
        \centering
        \includegraphics[width=\textwidth]{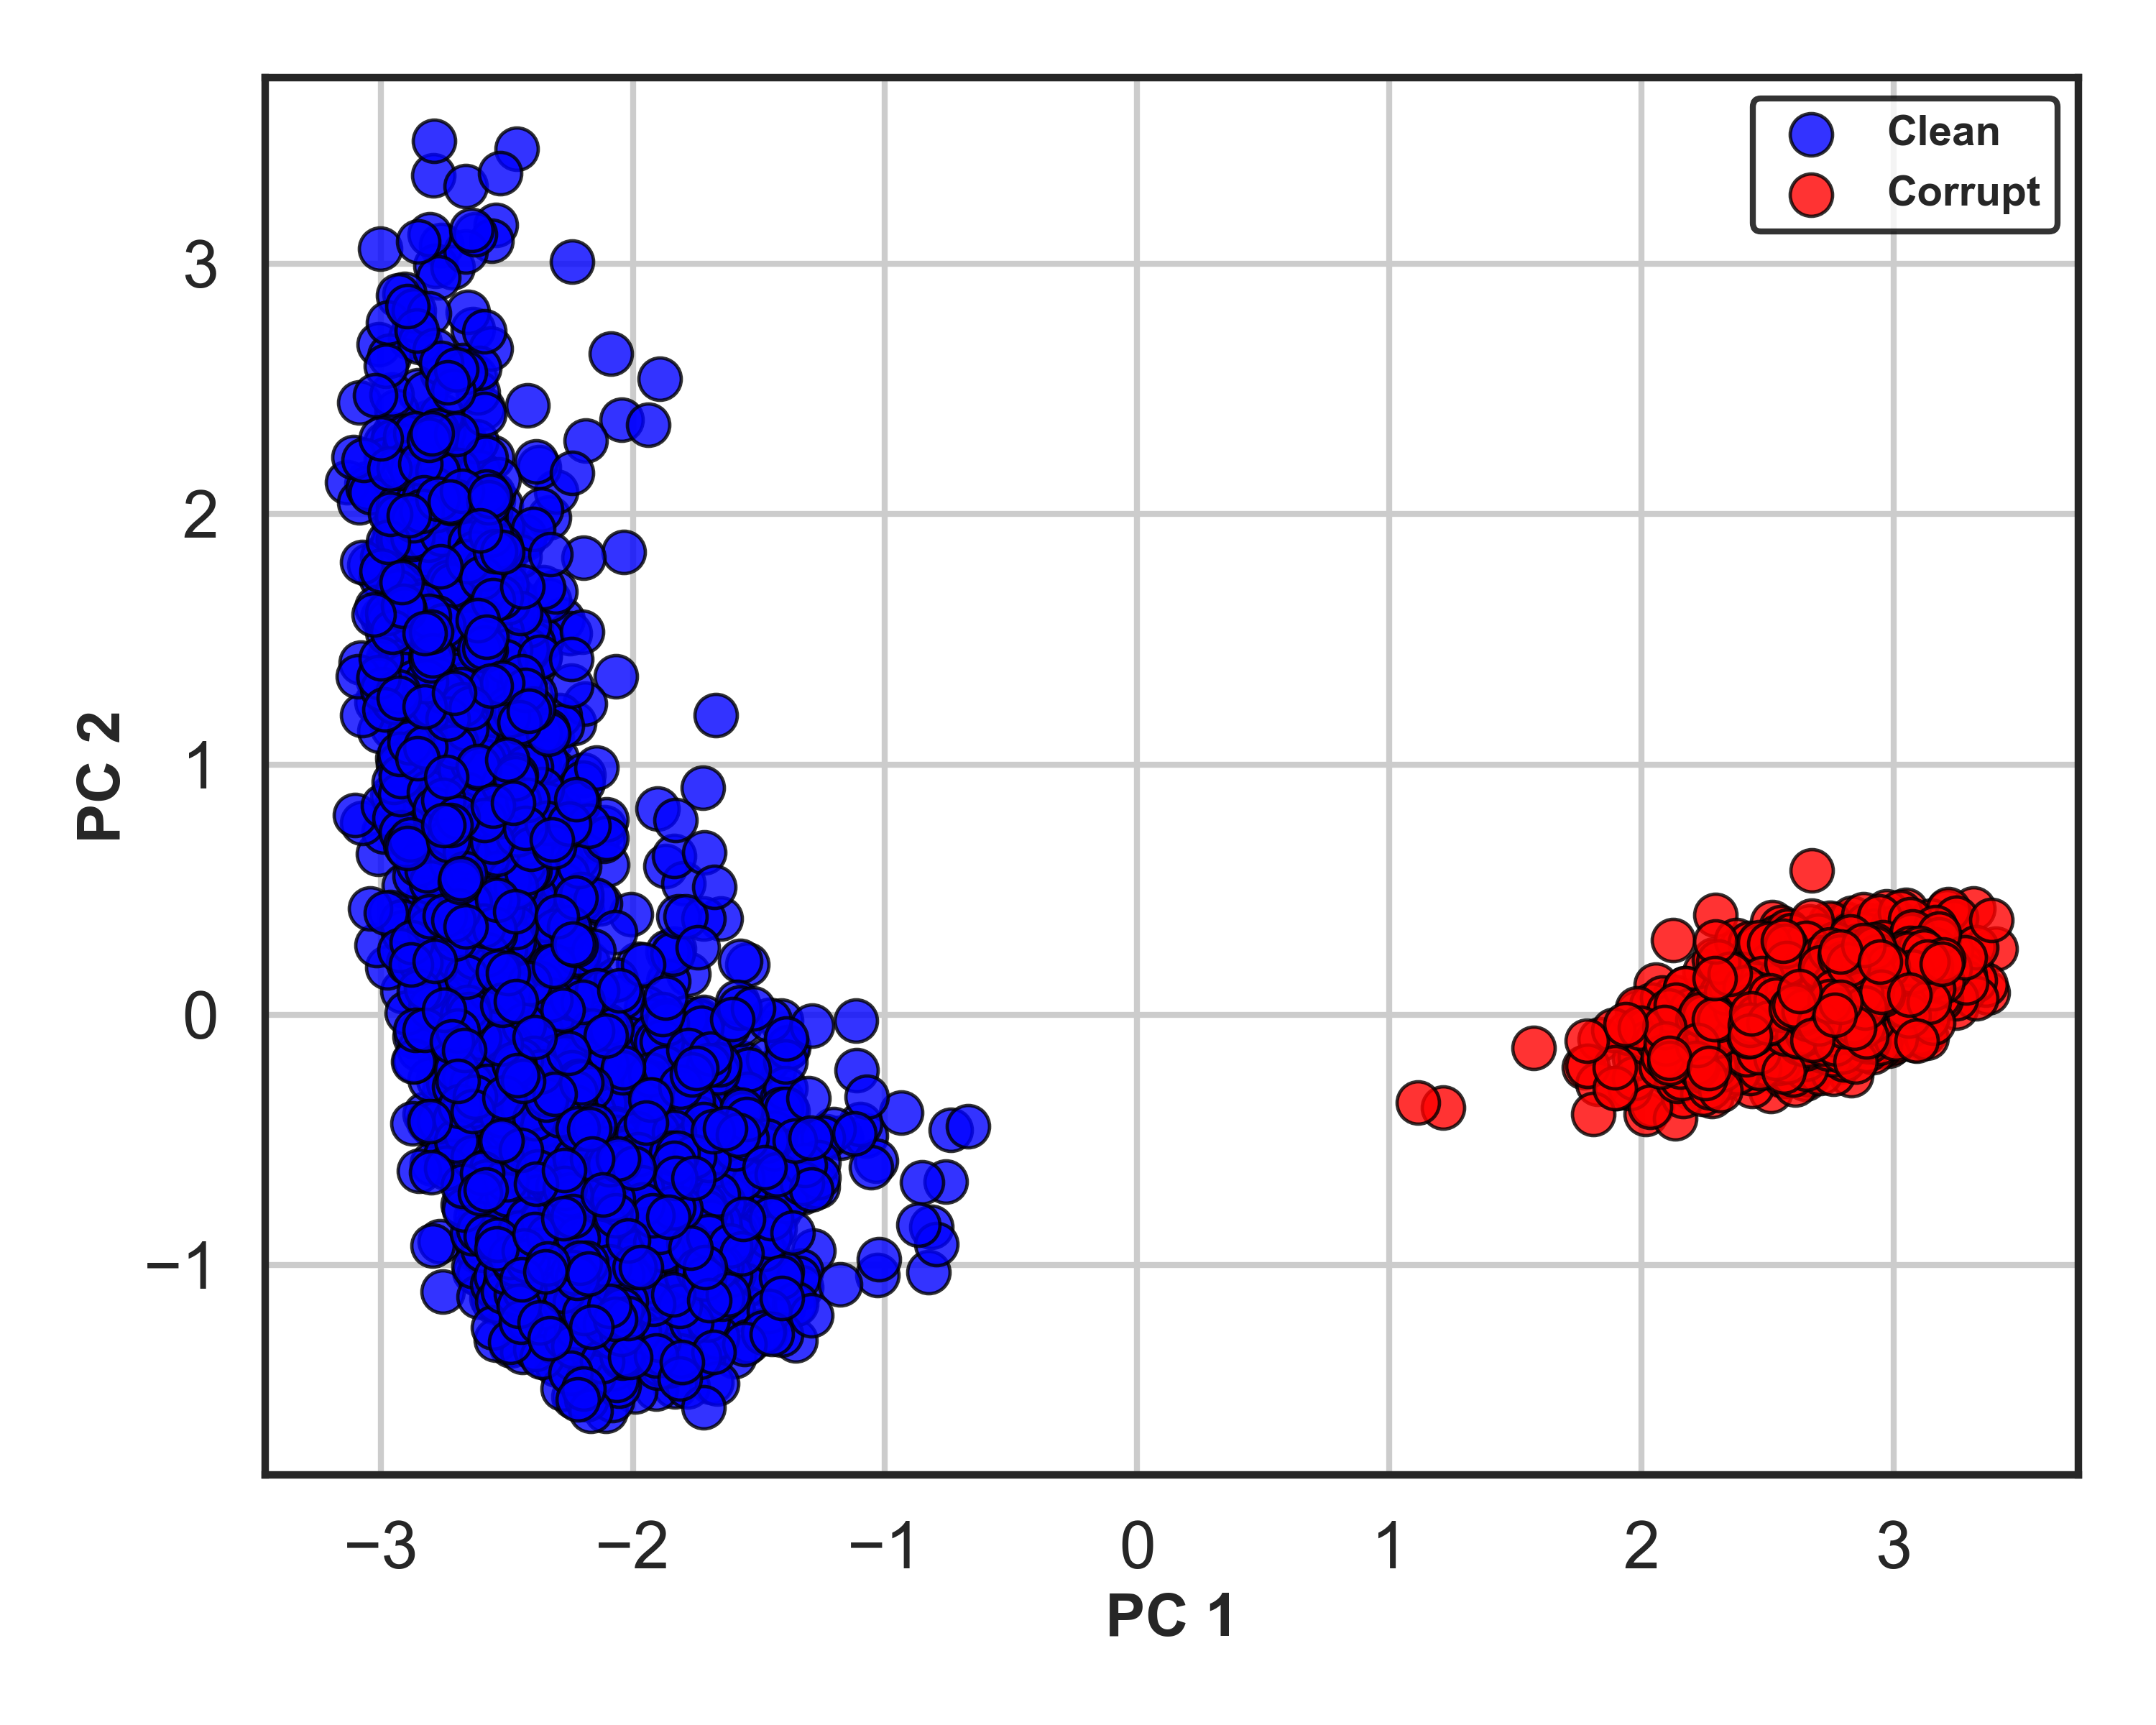}
        \caption{(Additive) Gaussian Noise}
    \end{subfigure}
    \hfill
    \begin{subfigure}[b]{0.3\textwidth}
        \centering
        \includegraphics[width=\textwidth]{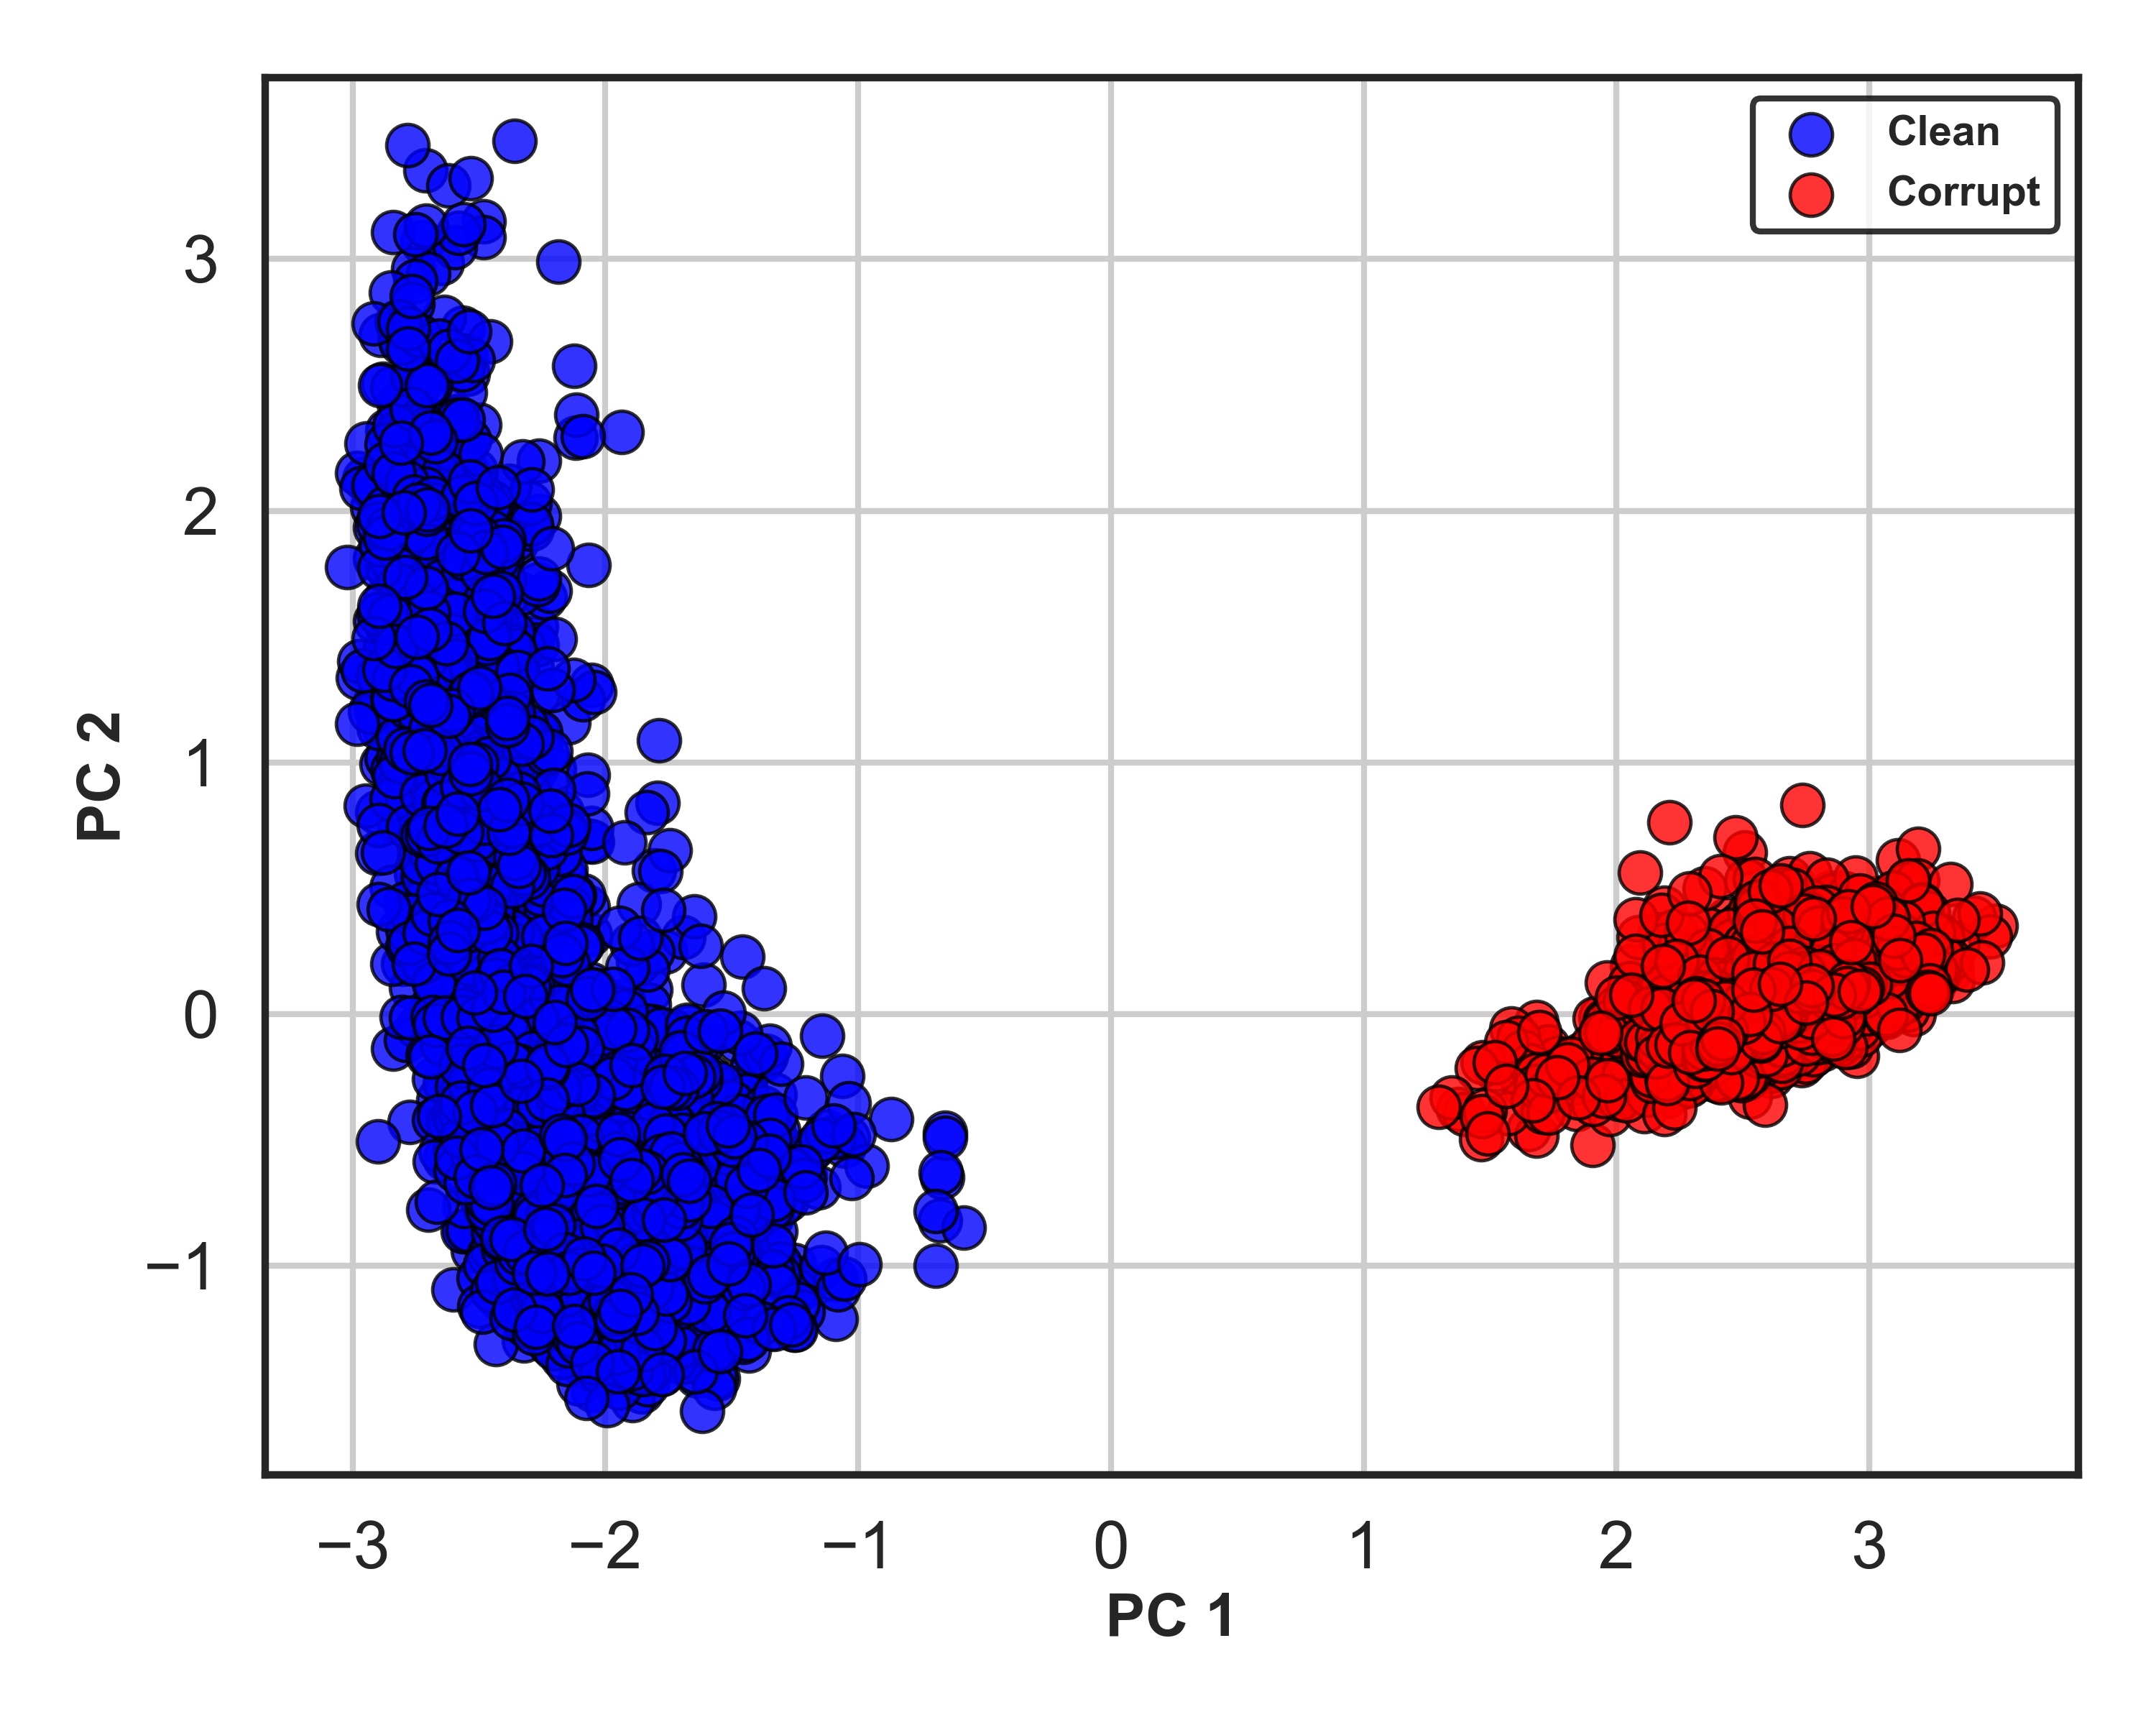}
        \caption{(Additive) Uniform Noise}
    \end{subfigure}

    \vspace{1.5em}
    
    % Second row of subfigures
    \begin{subfigure}[b]{0.3\textwidth}
        \centering
        \includegraphics[width=\textwidth]{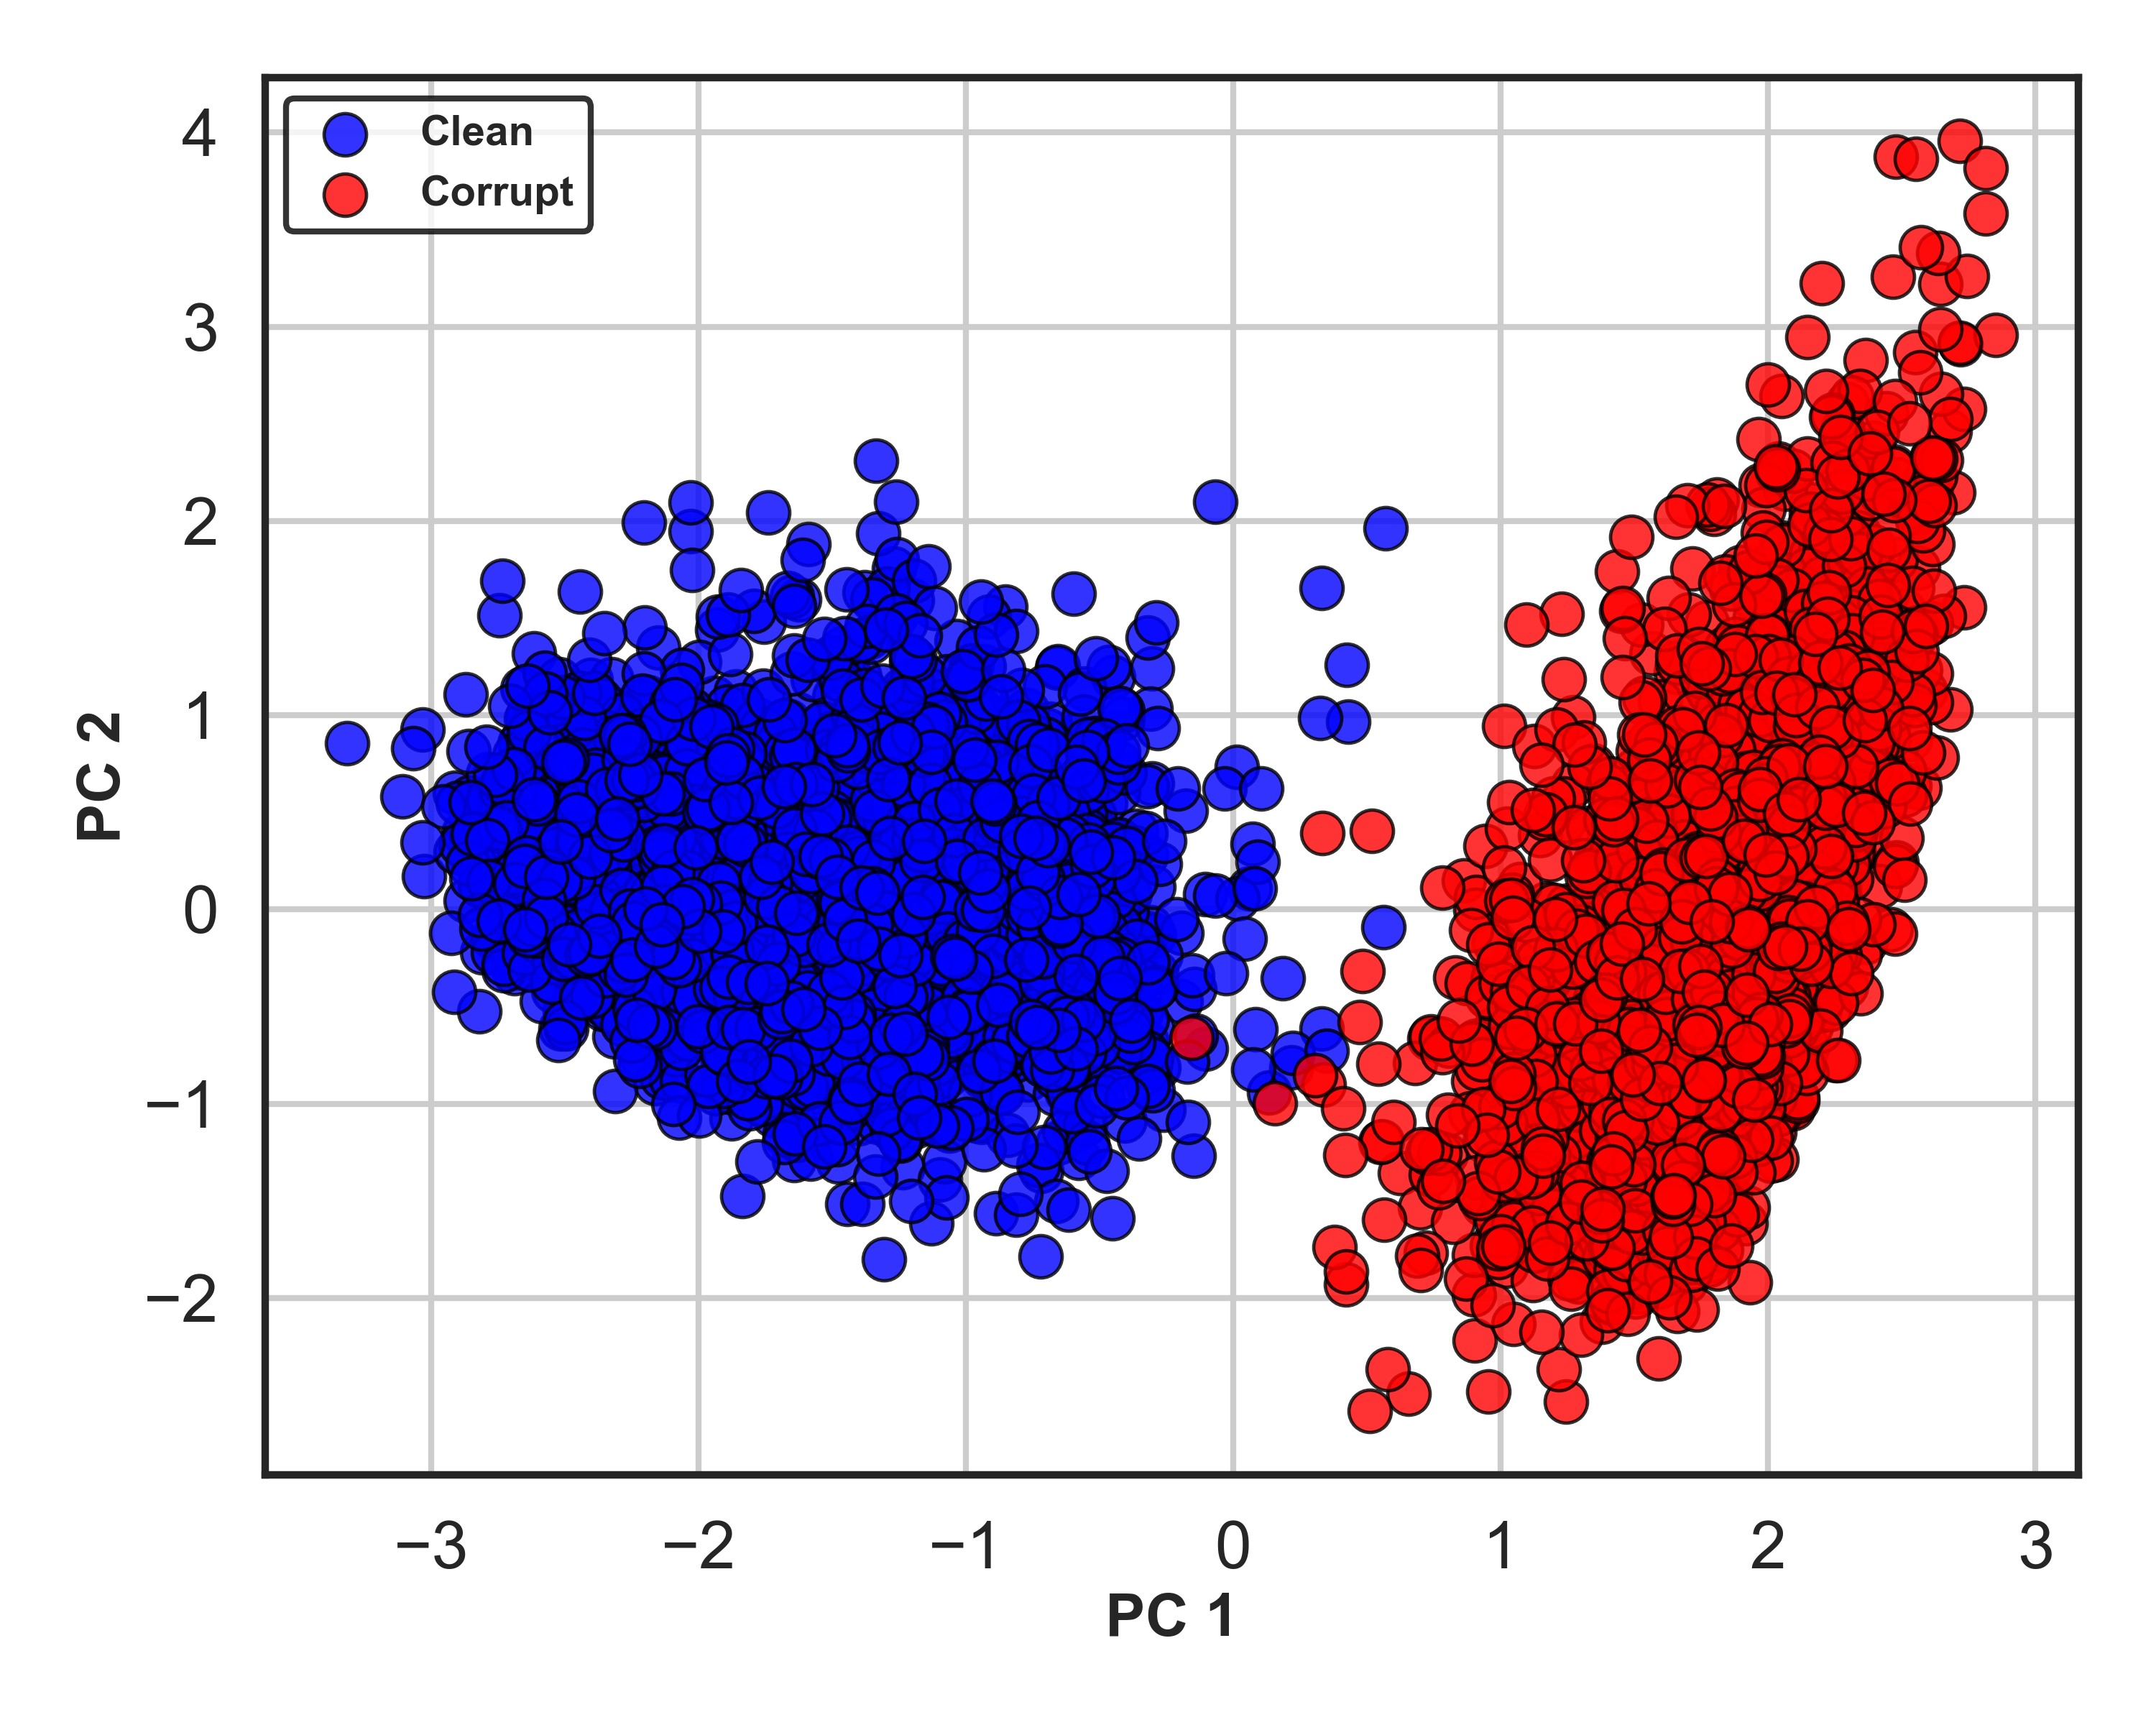}
        \caption{Random Patches}
    \end{subfigure}
    \hfill
    \begin{subfigure}[b]{0.3\textwidth}
        \centering
        \includegraphics[width=\textwidth]{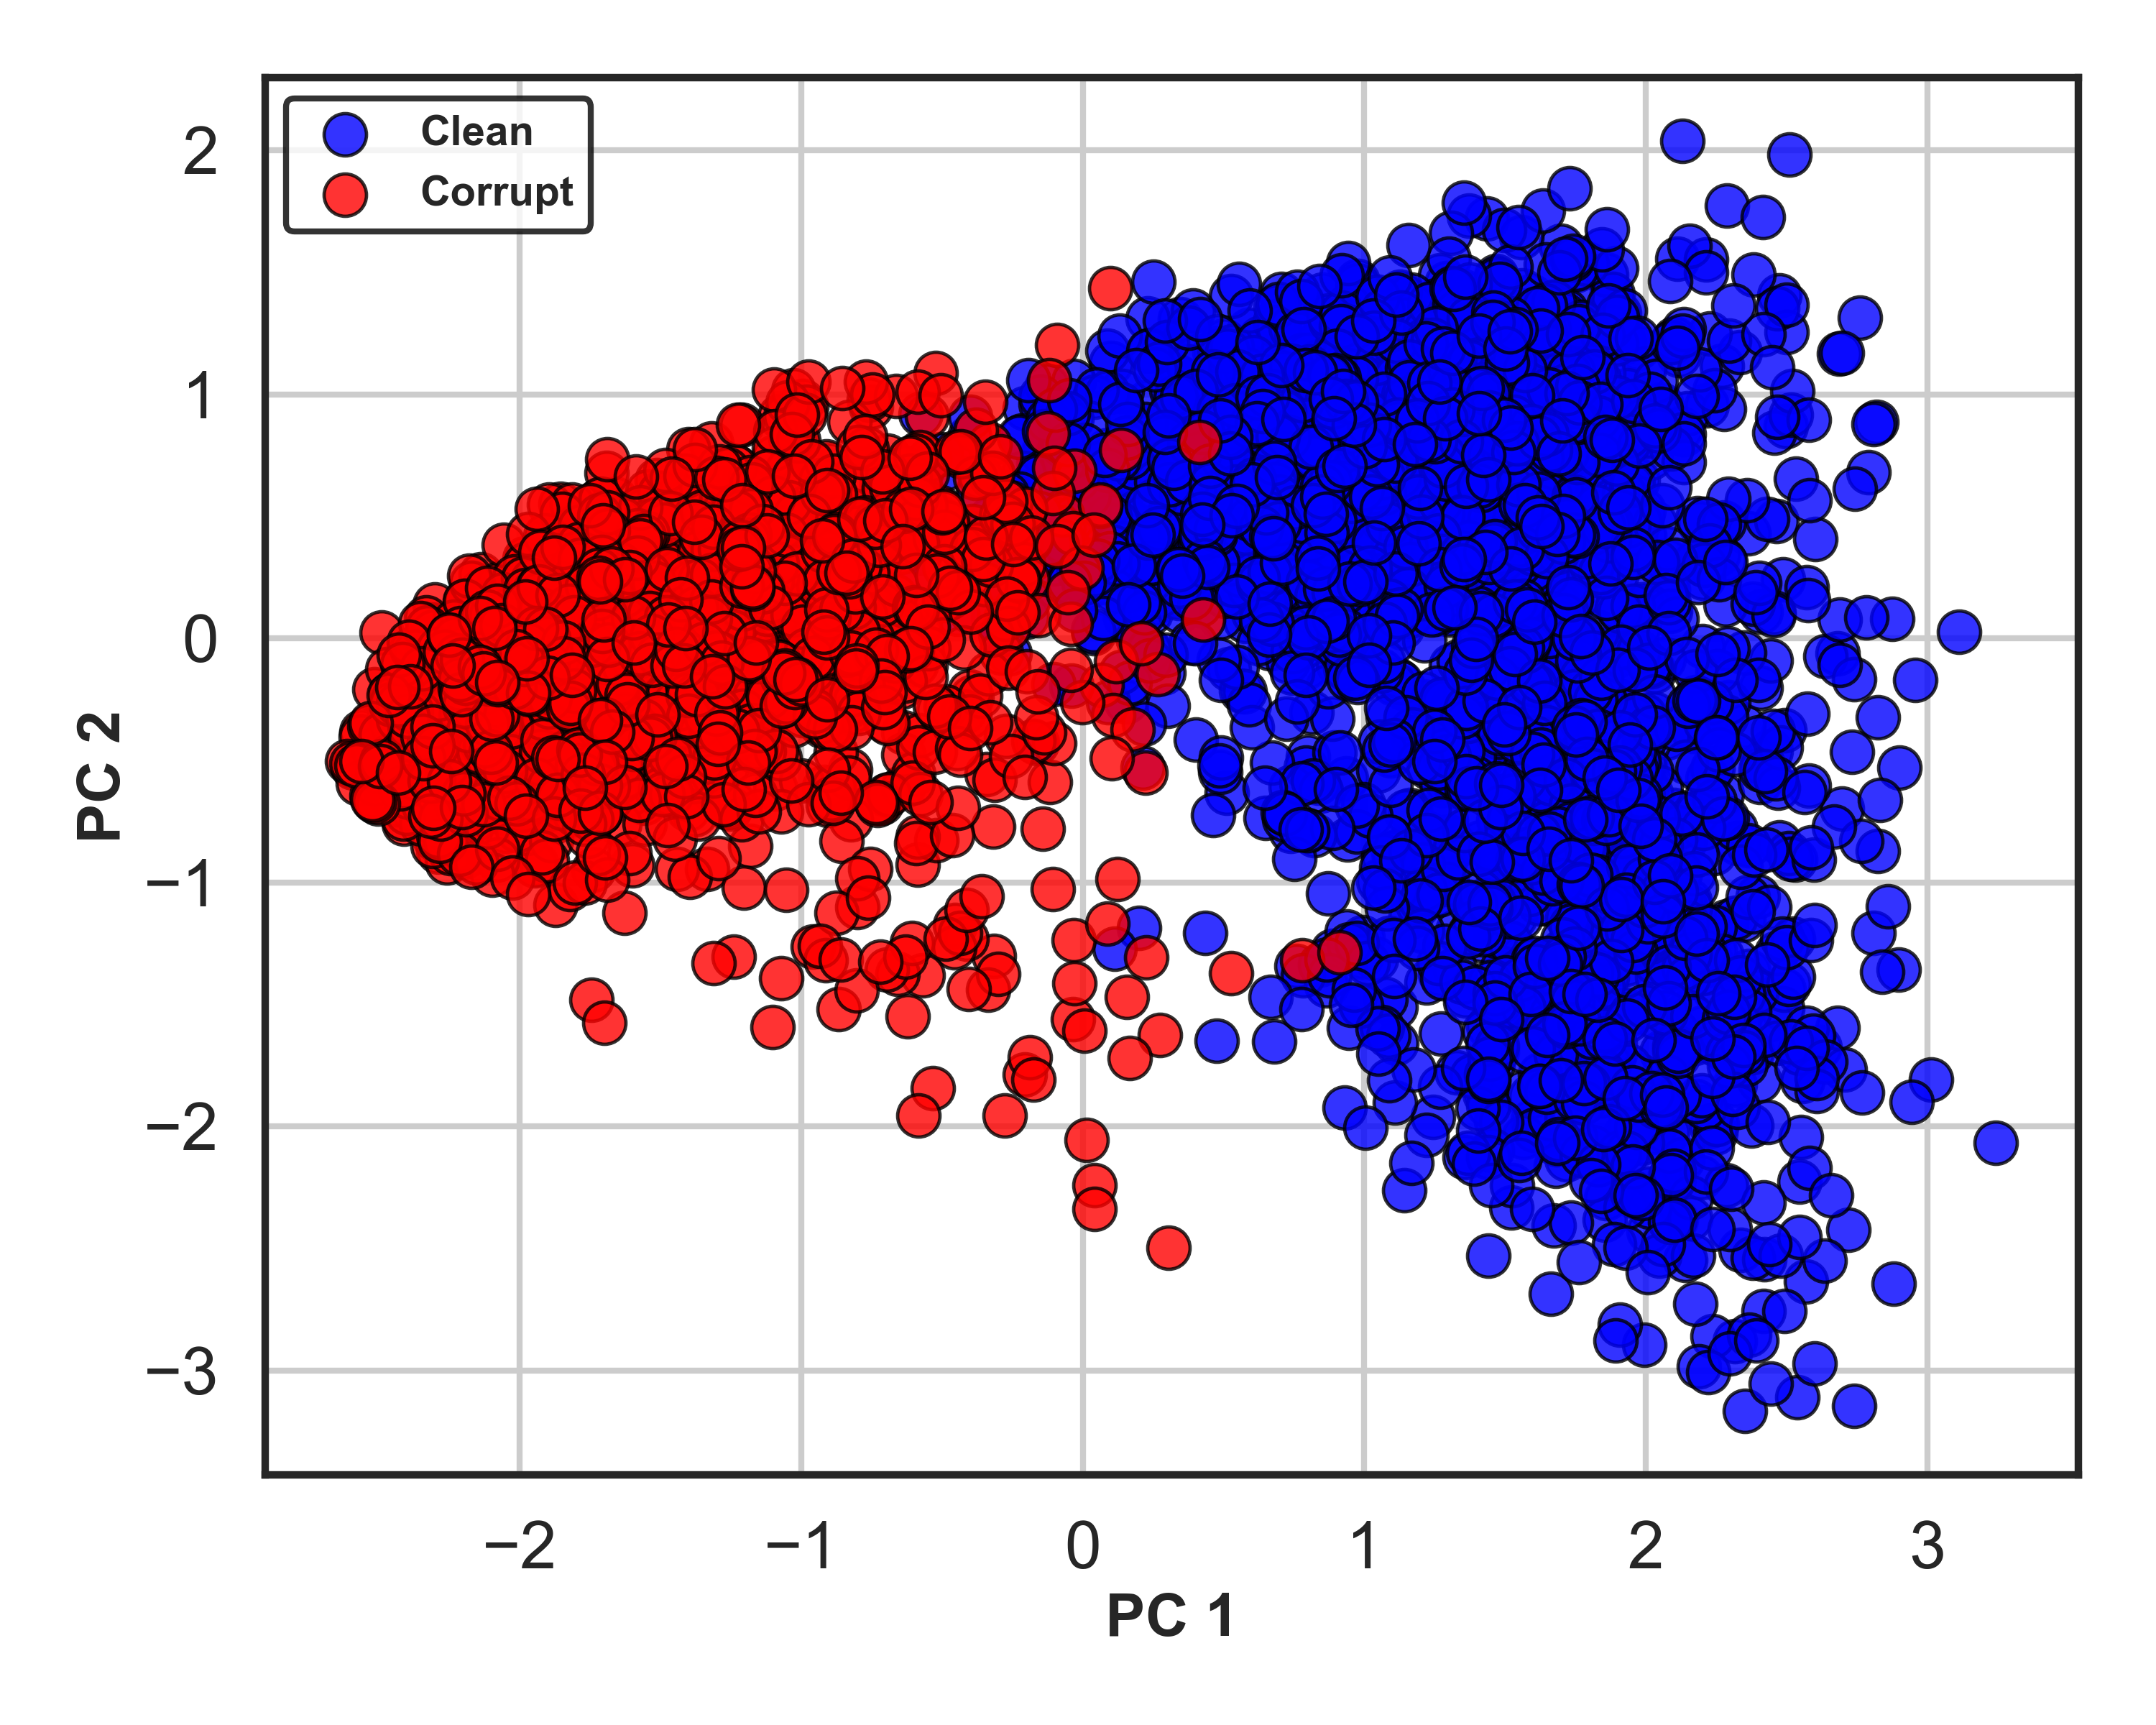}
        \caption{Cutout Noise}
    \end{subfigure}
    \hfill
    \begin{subfigure}[b]{0.3\textwidth}
        \centering
        \includegraphics[width=\textwidth]{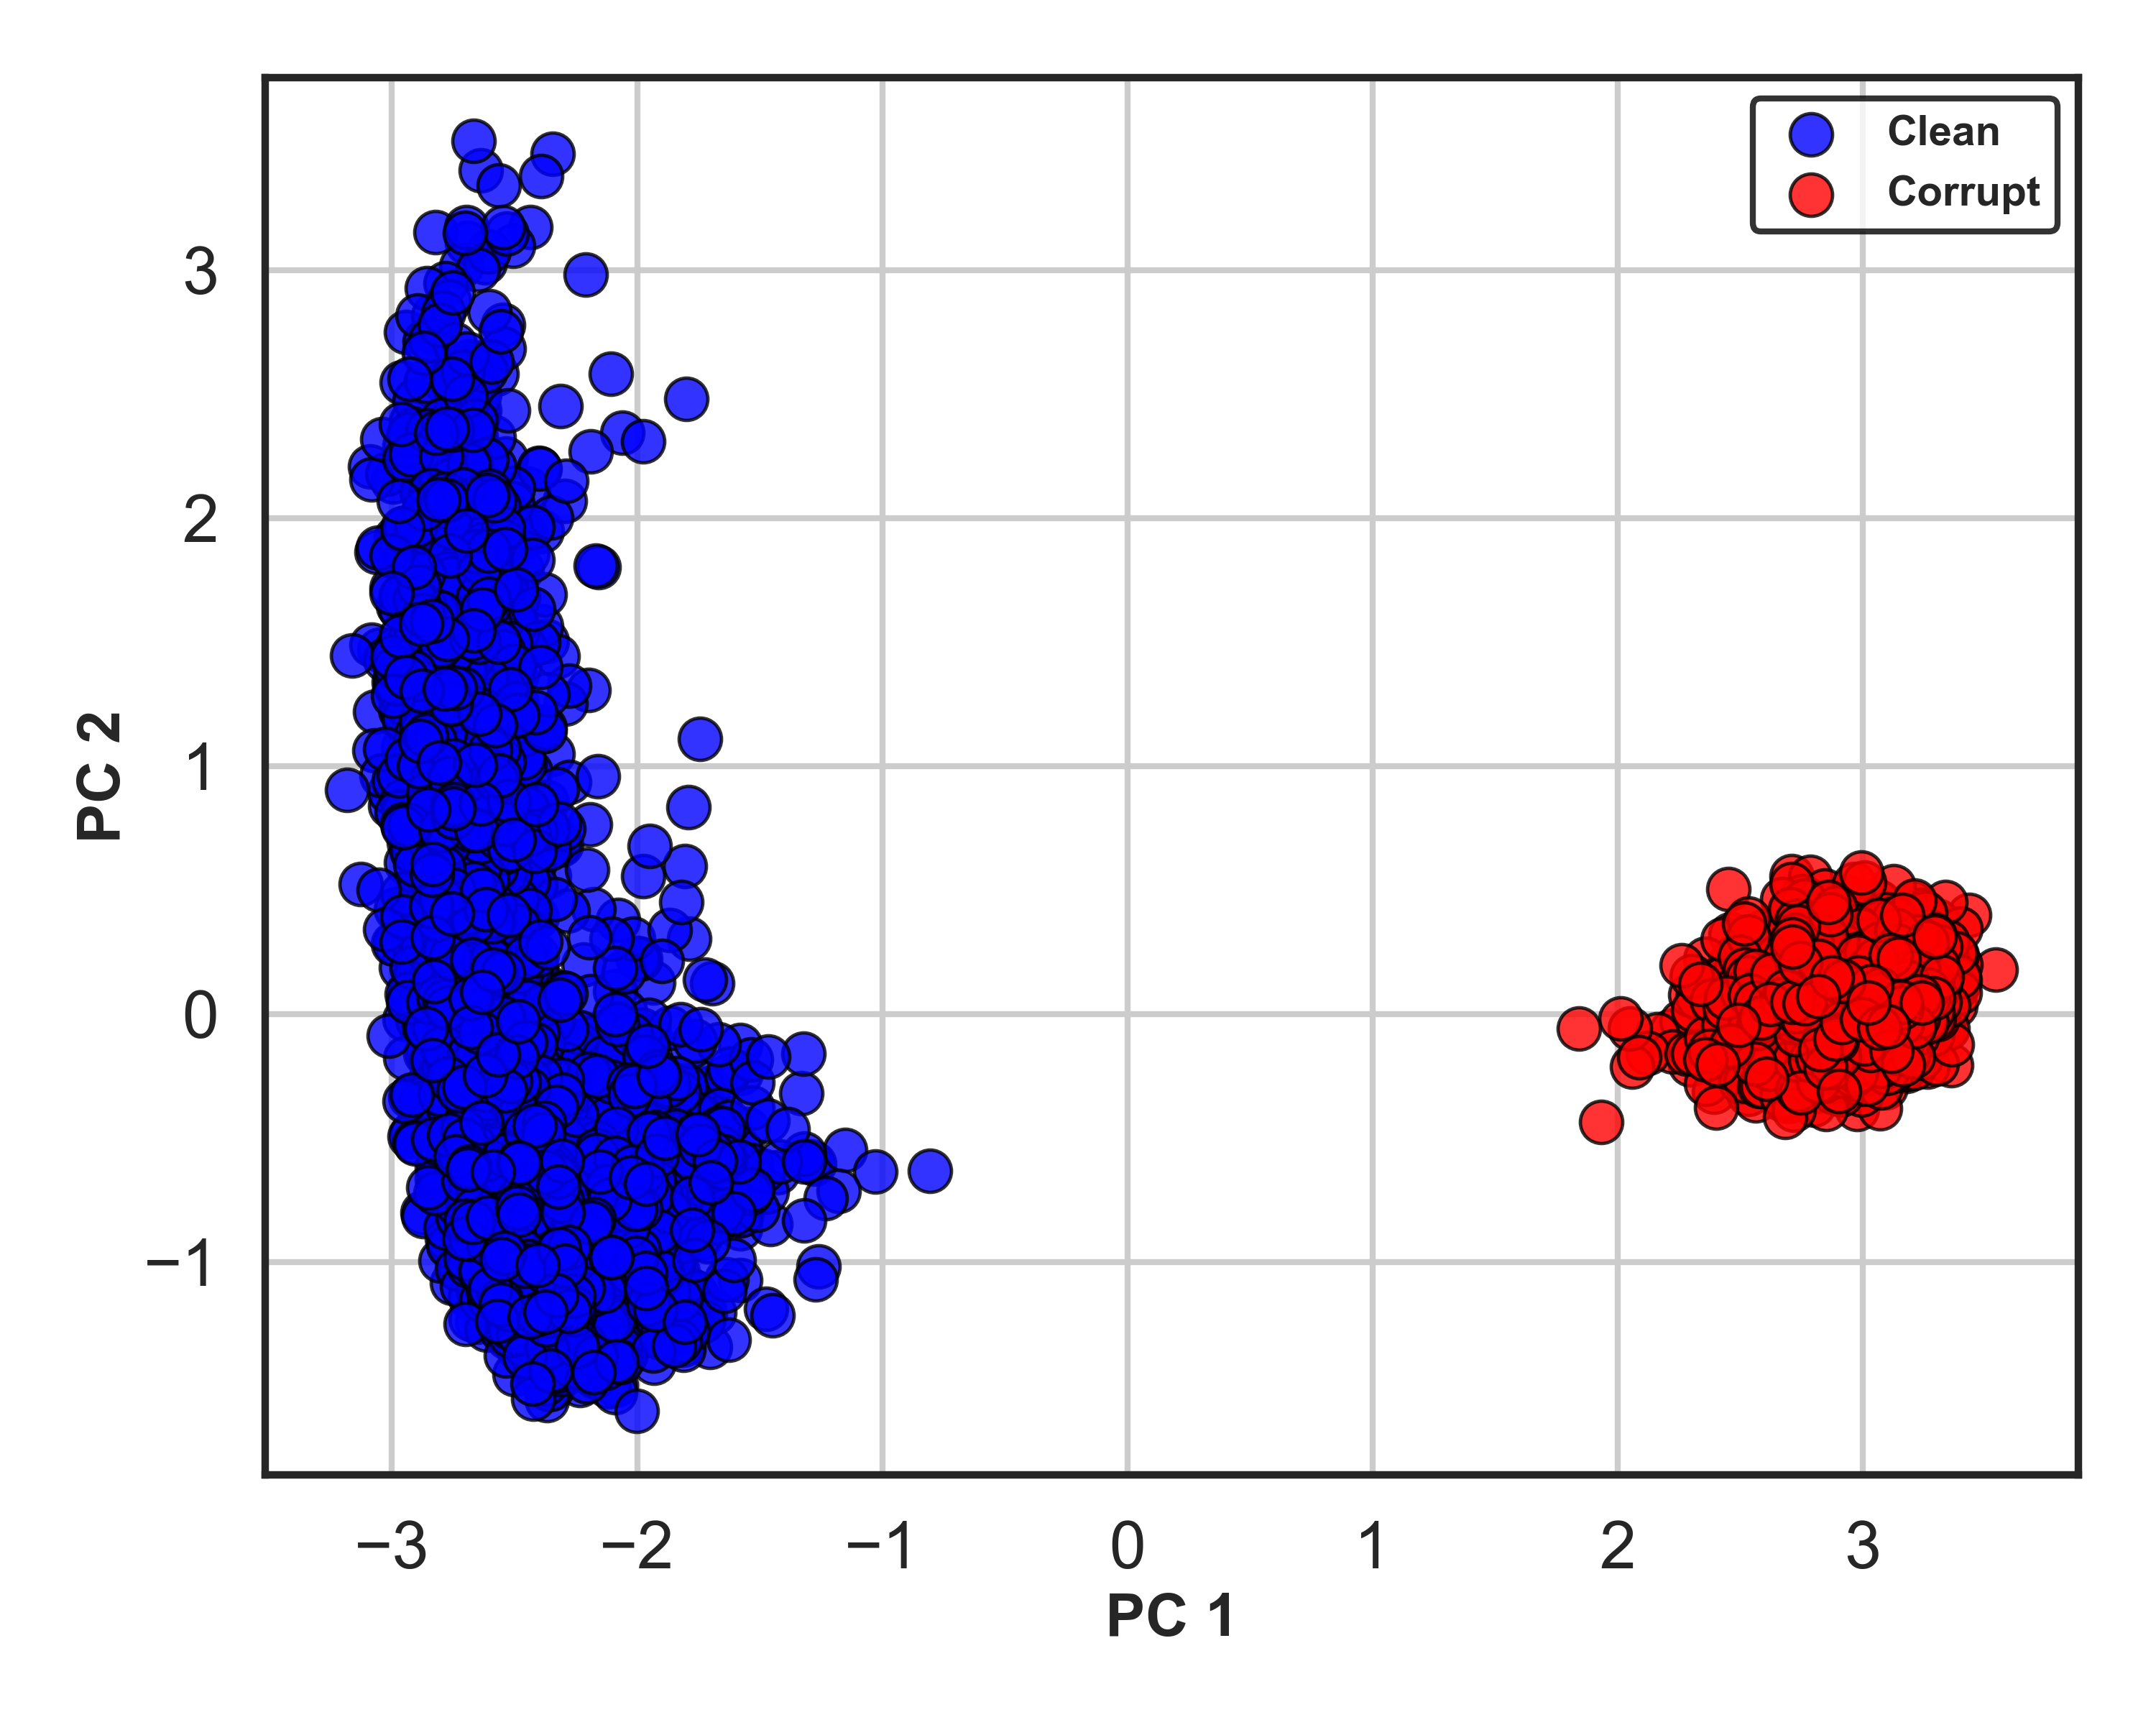}
        \caption{Random Noise}
    \end{subfigure}

    \caption{{\bf (PCA)} Visualization of CLIP ViT-B/32 Embeddings of a subset of MNIST images :  
    (a) Clean (baseline), and where 45\% samples corrupted with (b) Gaussian noise, (c) Uniform noise, (d) Random patches, (e) Cutout noise.}
    \label{fig:diffusion_noise_samples_pca_mnist}
\end{figure}

\input{plots/benchmarks/CIFAR10-LP-Label-Noise/main-fig}

\subsection{Generalization to Unseen Network / Domain}

Since the input features (e.g. images) often reside on a non-separable manifold, data pruning strategies rely on a proxy model to map the samples into a separable manifold (embedding space), wherein the data pruning strategies can now assign importance scores. However, it is important for the data pruning strategies to be robust to architecture changes i.e. to say that samples selected via a proxy network should generalize well when trained on unseen (during sample selection) networks / domains. We perform experiments on two such scenarios: 

\subsection{Network Transfer}

In this setting, the proxy model is trained on the target dataset (no distribution shift). However, the proxy architecture is different from the downstream network. In~\cref{tab:main-nw-T}, we use a ResNet-50 proxy trained on Mini-ImageNet to sample the data. However, then we train a downstream SENet and EfficientNet-B0 on the sampled data.

\subsection{Domain Transfer}

Next, we consider the setting where the proxy shares the same architecture with the downstream model. However, the proxy used to select the samples is pretrained on a different dataset (distribution shift) than the target dataset. In~\cref{fig:main-cifar-vanilla} we use a proxy ResNet-18 pretrained on ImageNet to select samples from CIFAR10. The selected samples are used to train a subsequent ResNet-18. In~\cref{fig:main-cifar-lp}, we additionally freeze the pretrained encoder i.e. we use ResNet-18 encoder pretrained on ImageNet as proxy. Further, we freeze the encoder and train a downstream linear classifier on top over CIFAR-10.

\clearpage
\section{Additional Diffusion Experiments (Image Generation)}
\label{sec:app-diff}
In this section, we will discuss additional details about our diffusion (Image Generation) experiments.

\subsection{Corruptions}

\subsection{CLIP Embedding Visualization}

\subsection{Experimental Results}
\begin{table}
\centering
\caption{
\footnotesize{\bf \textsc{Unconditional Image Generation}}: FID Scores for training a Denoising Diffusion Probabilistic Model (DDPM)~\citep{ho2020denoising} with data sampled by different methods across varying Subset Sizes and Corruption fractions from MNIST. Bold values highlight the best performance at each subset size and . Lower FID indicates better generative quality.
}
\label{tab:fid_scores}
\begin{adjustbox}{max width=\linewidth}
\begin{tabular}{@{}lccccc@{}}
\toprule
\multirow{2}{*}{\textbf{Sampling}} & \multicolumn{5}{c}{\textbf{Subset Size}} \\
\cmidrule(lr){2-6}
& \textbf{5\%} & \textbf{10\%} & \textbf{20\%} & \textbf{40\%} & \textbf{100\%} \\
\midrule
\multicolumn{5}{c}{{\bf No Corruption}}
\\
\midrule
\textbf{Random}       
& 115.11
& {\bf 13.79}
& 10.93
& 3.68
& 0.48
\\
\textbf{Easy}         
& {\bf 95.13}
& 54.33
& 12.62
& 9.08
& 0.48
\\
\textbf{Hard}         
& 148.73
& 25.82
& 43.71
& 8.37
& 0.48
\\
\textbf{Moderate}     
& 119.40
& 28.87
& 14.72
& 5.26
& 0.48
\\
\textbf{Herding}      
& 120.21
& 52.18
& 18.76
& \textcolor{gray}{\bf 2.55}
& 0.48
\\
\textbf{GM Matching}  
& \textcolor{gray}{\bf 100.24}
& \textcolor{gray}{\bf 17.72}
& {\bf 5.26}
& {\bf 1.77}
& 0.48
\\
\midrule
\multicolumn{6}{c}{{\bf 20\% Corruption}}
\\
\midrule
\textbf{Random}       
& 121.58
& 89.02
& 60.58
& 52.76
& 42.05
\\
\textbf{Easy}         
& \textcolor{gray}{\bf 102.72}
& 87.05
& 34.23
& 21.06
& 42.05
\\
\textbf{Hard}         
& 128.64
& 87.69
& 56.98
& 48.17
& 42.05
\\
\textbf{Moderate}     
& 114.61
& 14.86
& 11.73
& 7.99
& 42.05
\\
\textbf{Herding}      
& 129.10
& 52.61
& 23.96
& 12.76
& 42.05
\\
\textbf{GM Matching}  
& {\bf 87.31} 
& {\bf 12.52} 
& 14.91
& 4.00
& 42.05
\\
\midrule
\multicolumn{6}{c}{{\bf 30\% Corruption}}
\\
\midrule
\textbf{Random}       
& 121.97
& 98.95
& 81.64
& 61.79
& 65.55
\\
\textbf{Easy}         
& 90.06
& 88.81
& 39.67
& 20.89
& 65.55
\\
\textbf{Hard}         
& 124.31
& 110.58
& 95.59
& 87.18
& 65.55
\\
\textbf{Moderate}     
& 102.67    
& \textcolor{gray}{\bf 17.95}
& 30.13
& 22.66
& 65.55
\\
\textbf{Herding}      
& 125.67
& 80.20
& 74.68
& 72.63
& 65.55
\\
\textbf{GM Matching}  
& {\bf 73.57}
& {\bf 7.52}
& {\bf 3.30}
& {\bf 2.45}
& 65.55
\\
\bottomrule
\end{tabular}
\end{adjustbox}
\end{table}

\subsection{Generated Samples}
\input{gen/clean}
\input{gen/noisy}
